# Supplementary material for: Inclusive cross section measurements in final states with and without protons for charged-current $\nu_\mu$-Ar scattering in MicroBooNE
Source: arXiv:2402.19216 ancillary file (2024-07-27)
Supplement: Supplementary file 1 [file SupplementalMaterial.pdf]

# Supplemental Material for "Inclusive cross section measurements in final states with and without protons for charged-current $\nu_\mu$-Ar scattering in MicroBooNE"

## I. 2D AND 3D SMEARING AND EFFICIENCIES

The section presents the smearing matrices for the 2D $\{\cos\theta_p^{rec} K_p^{rec}\}$, 2D 0pNp $\{\cos\theta_\mu^{rec}, E_\mu^{rec}\}$, and 3D $\{E_{avail}^{rec}, \cos\theta_\mu^{rec}, E_\mu^{rec}\}$ distributions. The efficiency of the $\nu_\mu$CC selection as a function of the same variables is also shown. The binning used for these plots is the same as used for $S$ and $M$ in the cross section extraction. All bins are equal width and do not represent the physical width of the energy and angular bins. For the 2D distributions, the bins are in angular slices that go from backwards on the left to forwards on the right with increasing energy bins within each slice. The 3D distribution is further divided into $E_{avail}$ slices, with least energetic on the left and most energetic on the right. A complete set of angular slices is contained in each $E_{avail}$ slice with same structure as the 2D distributions. More information on the binning can be found in Sec. VIII.

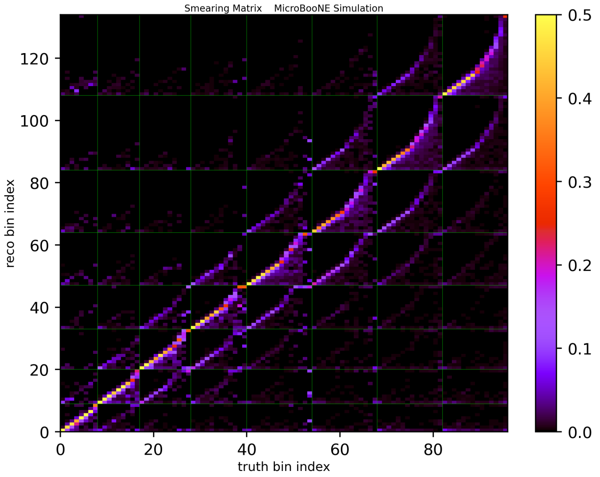


(a) $\cos\theta_p$ and $K_p$ smearing matrix for FC events.

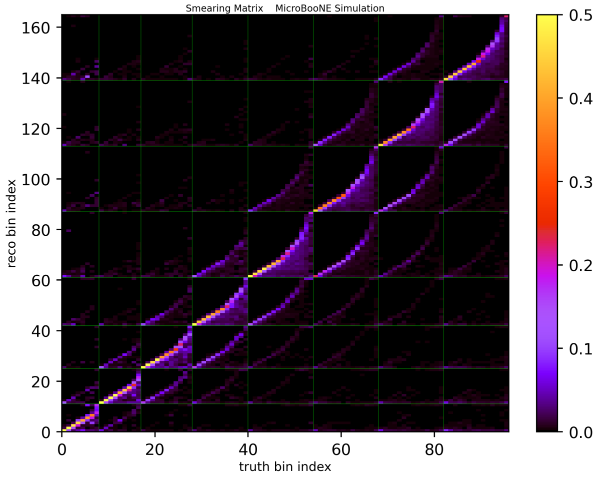


(b) $\cos\theta_p$ and $K_p$ smearing matrix for PC events.

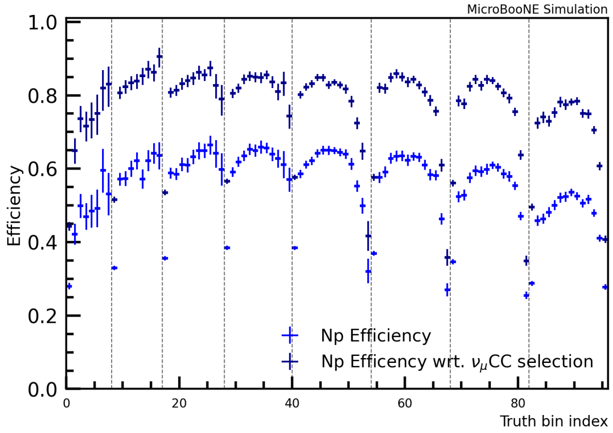


(c) $\nu_\mu$CC selection efficiency as a function of $\cos\theta_p$ and $K_p$

FIG. 1: Smearing matrix for the double differential measurement of $\cos\theta_p$ and $K_p$ for FC events (a) and PC events (b). All columns have been normalized to one. The green lines indicate the different angular slices. (c) Vectored efficiency of the $\nu_\mu$CC selection for each true $\cos\theta_p$ and $K_p$ bin in the double differential measurement. The dotted lines indicate the different angular slices. In all plots, the bins are the same as those on $M$ and $S$ in the cross section extraction but are all equal width and do not represent the physical width of the energy and angular slices. The angular slices go from backwards on the left to forward on the right. The last bin in each angular slice corresponds to overflow and no 0p bin is included.

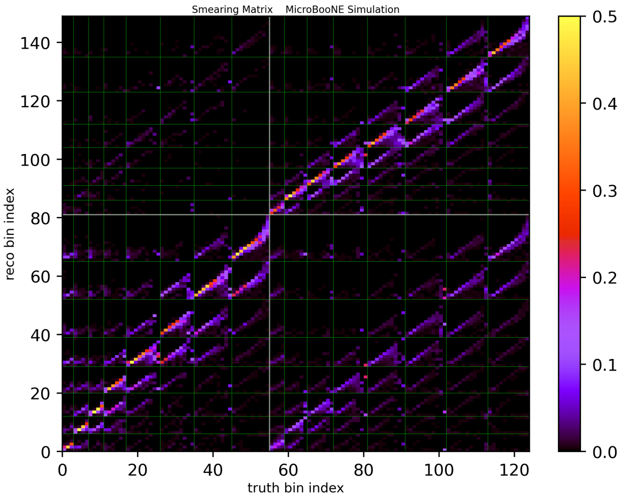


(a) $\cos\theta_\mu$ and $E_\mu$ 0pNp smearing matrix for FC events.

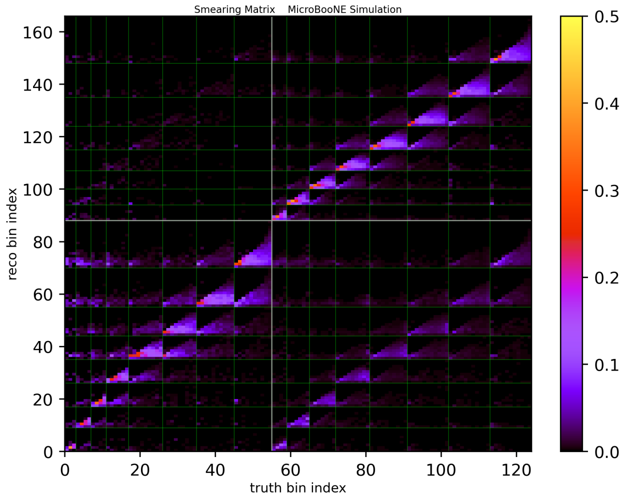


(b) $\cos\theta_\mu$ and $E_\mu$ 0pNp smearing matrix for PC events.

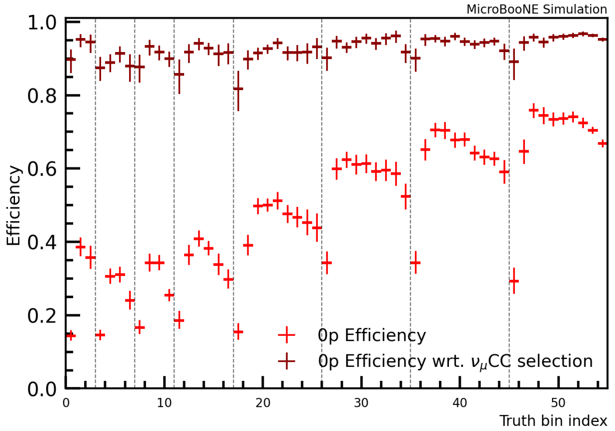


(c) $\nu_\mu$CC 0p selection efficiency as a function of $\cos\theta_\mu$ and $E_\mu$

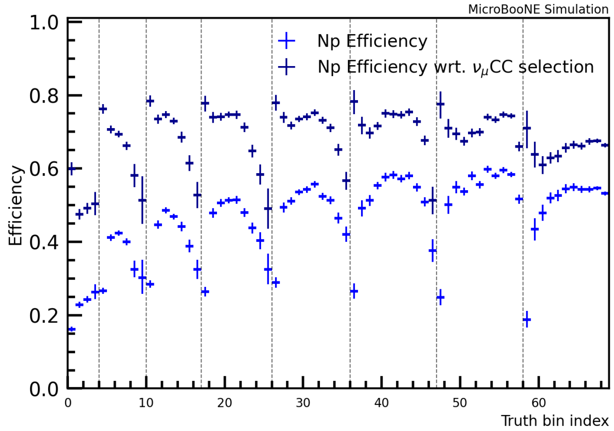


(d) $\nu_\mu$CC Np selection efficiency as a function of $\cos\theta_\mu$ and $E_\mu$

FIG. 2: Smearing matrix for the 0pNp double differential measurement of $\cos\theta_\mu$ and $E_\mu$ for FC events (a) and PC events (b). All columns have been normalized to one. The white lines indicate the split between 0p and Np bins and the green lines indicate the different angular slices. The reconstructed 0p true 0p bins are on the bottom left and the true Np reconstructed Np bins are on the top right. The vectorized 0p (c) and Np (d) efficiency of the $\nu_\mu$CC selection for each true $\cos\theta_\mu$ and $E_\mu$ bin in the double differential measurement. The dotted lines indicate the different angular slices. In all plots, the bins are the same as those on $M$ and $S$ in the cross section extraction but are all equal width and do not represent the physical width of the energy and angular bins. The angular slices go from backwards on the left to forward on the right. The last bin in each angular slice corresponds to overflow.

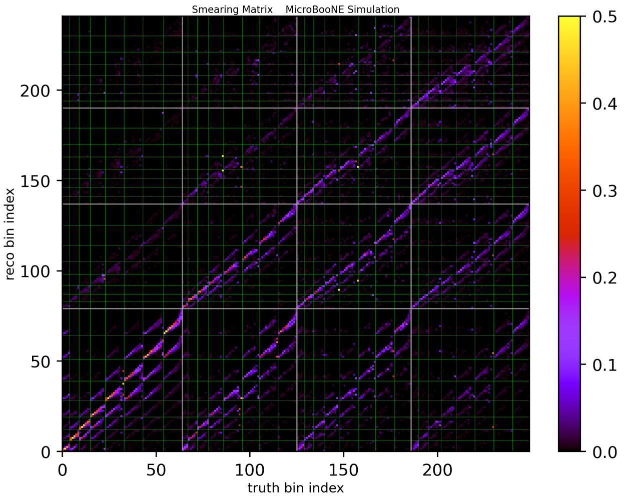


(a) $E_{avail}$, $\cos\theta_\mu$ and $E_\mu$ smearing matrix for FC events.

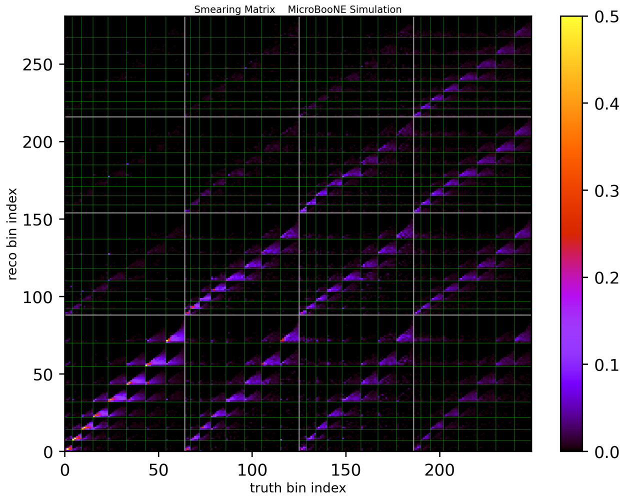


(b) $E_{avail}$, $\cos\theta_\mu$ and $E_\mu$ smearing matrix for PC events.

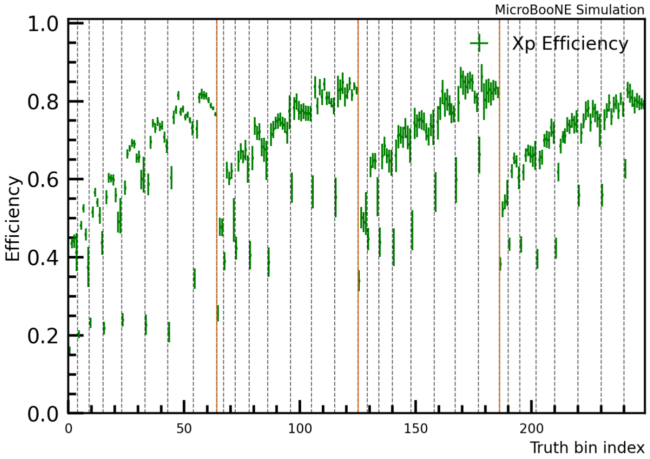


(c) $\nu_\mu$CC selection efficiency as a function of $E_{avail}$, $\cos\theta_\mu$ and $E_\mu$

FIG. 3: Smearing matrix for the Xp triple differential measurement of $E_{avail}$, $\cos\theta_\mu$ and $E_\mu$ for FC events (a) and PC events (b). All columns have been normalized to one. The brown lines indicate the separation between different $E_{avail}$ slices and the green lines indicate the separation between different angular slices. (c) the vectorized efficiency of the efficiency of the $\nu_\mu$CC selection for the $E_{avail}$, $\cos\theta_\mu$ and $E_\mu$ bins used in the triple differential measurement. The dotted lines indicate the different angular slices, and the brown lines indicate the different $E_{avail}$ slices. In all plots, the bins are the same as those on $M$ and $S$ in the cross section extraction but are all equal width and do not represent the physical width of the energy and angular bins. The $E_{avail}$ slices go from leas energetic on the left to most energetic on the right. The angular slices go from backwards on the left to forward on the right. The last bin in each angular slice corresponds to overflow.

## II. FAKE DATA STUDIES

Fake data studies (FDS) were conducted to evaluate if the model validation is sufficient for detecting relevant mis-modeling before it becomes prominent enough to bias the extracted cross sections beyond stated uncertainties. These supplement the FDS shown in [1] that utilize a fake data set produced by the `NuWro` event generator to demonstrate the sensitivity of the validation and the subsequent efficacy of the procedure used for deriving an additional reweighting uncertainty. The FDS shown here are conducted at $6.4 \times 10^{20}$ POT with all systematic uncertainties, except the additional reweighing uncertainty, which was derived specifically for real data only after the model was shown to be insufficient. Including all systematic uncertainties, rather than only cross section uncertainties as is common done for FDS, serves as a more realistic test of the stringency of the model validation. Through the conditional constraint, the validation cancels shared systematics from all sources, including neutrino flux, cross section, and detector effects. Thus, a test with the complete set of systematics is required to demonstrate that the constraint is able to reduce uncertainties on the reconstructed distributions enough to detect relevant mismodeling that will bias the extraction beyond stated uncertainties. These FDS indicate that the validation used for this work is significantly more stringent than the cross section extraction and that, when the model passes these tests, it can be used to extract cross sections that do not bias the results beyond the quoted total model uncertainty.

Similar to the FDS described in the Supplemental Material of [2], fake data sets are generated from the nominal MicroBooNE MC by scaling the reconstructed proton energy by some factor. The reconstructed and true muon kinematics remain unaltered for these studies. This mimics a systematic effect whereby the model incorrectly predicts the amount of visible energy (e.g. from protons) that becomes invisible (e.g. neutrons, below threshold particles) as a result of extra nuclear effects or final-state interactions. The more the scaling factor deviates from unity, the greater the difference between the fake data and the model in the fraction of the true energy transfer which is invisible. Such an effect is expected to be especially relevant to the extraction of the $E_\nu$, $\nu$, $E_{avail}$ and $K_p$ cross sections, especially in the context of the 0p and Np final states studies in this work. Generating fake data in this way does not change the underlying true neutrino energy or transfer energy spectrum from the nominal MicroBooNE MC. However, since the reduction in the proton energy is assumed to arise from a cross section effect, the true proton energy is also scaled by the same factor as the reconstructed distribution. This alters the relative size of the 0p and Np cross sections, and the differential cross sections directly related to the proton energy (i.e. $K_p$ and $E_{avail}$). Thus, closure of these FDS is achieved when the fake data cross section extraction reproducing the MicroBooNE MC prediction with the appropriate scaling applied to the true proton energy spectrum.

The results of these FDS with proton energy scalings are summarised in Fig. 4(a). The x-axis indicates the degree to which the proton energy was scaled and the y-axis indicates the tension between the fake data and nominal MicroBooNE MC in the model validation tests, and the tension between the extracted fake data cross sections and truth. This is expressed in terms of one-dimensional $\sigma$ values computed from the $p$-values obtained in each test. The band indicates the range of $\sigma$ values obtained for the validation tests and the various points indicate the level of agreement between the extracted fake data cross sections and truth. The measurements expected to be most sensitive to mis-modeling are shown. The results for each FDS are also tabulated in Table I.

For all FDS, the $\sigma$ values for the extraction of the cross sections are well below the $\sigma$ values for the corresponding model validation tests. In other words, the bias induced by the cross section extraction is significantly less than the mismodeling detected by the model validation. This indicates that the validation is more stringent than the cross section extraction, allowing us to detect relevant mismodeling of the missing hadronic energy before it becomes relevant to the extraction. Success of the model in the validation procedure thus suggests that the difference between the data and simulation are within the quoted total model uncertainty. Furthermore, even at proton energy scalings past the point at which the validation indicates that there is relevant mismodeling, the agreement between the underlying truth and extracted results remains quite good for many of the cross sections. In particular, extraction of the cross section as a function of $E_\nu$ and the differential cross section as a function of $E_{avail}$ appears quite robust.

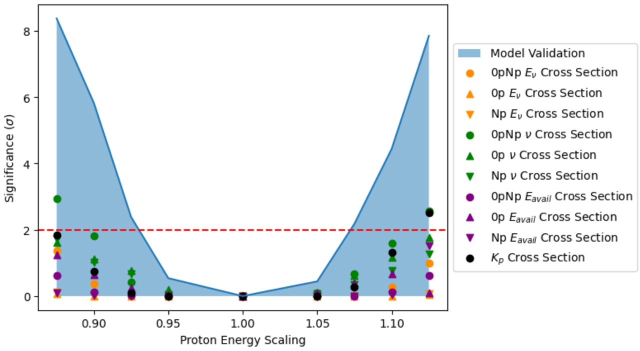


(a) FDS with various $K_p^{rec}$ scalings

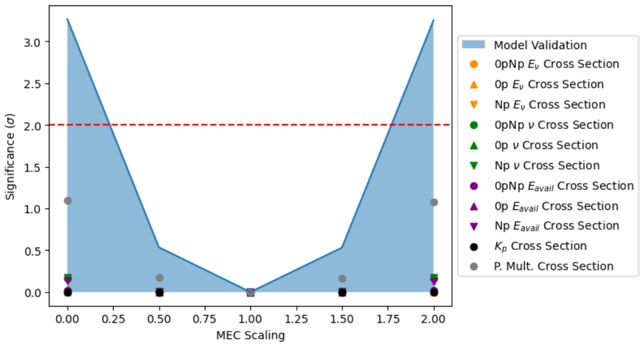


(b) FDS with various MEC event weight scalings

FIG. 4: Comparison of the stringency of the model validation to the amount of bias induced in the cross section extraction using fake data sets constructed from the nominal MicroBooNE MC by applying various scaling factors to the true and reconstructed proton energy spectrum (left) and MEC event weights (right). The x-axis corresponds to this scaling. The y-axis indicates the agreement between the fake data and nominal MicroBooNE MC for the model validation tests, or the extracted fake data cross section and truth. This is expressed in terms of one-dimensional $\sigma$ values. The band corresponds to the range of values obtained in validation tests and the points indicate the level of agreement between the extracted fake data cross sections and truth. For the model validation, large $\sigma$ values indicate high stringency. For the cross section extraction, large $\sigma$ values indicates more biased results and worse closure on the underlying true distribution.

| FDS Results With $K_p$ scaling at 6.4e20 POT | | | | | | | | | | |
|---|---|---|---|---|---|---|---|---|---|---|
| | | | 0.875 | 0.9 | 0.925 | 0.95 | 1.05 | 1.075 | 1.1 | 1.125 |
| XS Extr. | $E_\nu$ | 0p | 0.06 | 0.00 | 0.00 | 0.00 | 0.00 | 0.00 | 0.01 | 0.05 |
| | | Np | 0.13 | 0.01 | 0.00 | 0.00 | 0.00 | 0.00 | 0.02 | 0.08 |
| | | 0pNp | 1.36 | 0.38 | 0.02 | 0.00 | 0.00 | 0.02 | 0.28 | 0.99 |
| | $\nu$ | 0p | 1.63 | 1.11 | 0.78 | 0.19 | 0.07 | 0.62 | 1.18 | 1.76 |
| | | Np | 1.72 | 1.02 | 0.67 | 0.05 | 0.07 | 0.34 | 0.78 | 1.27 |
| | | 0pNp | 2.95 | 1.82 | 0.41 | 0.04 | 0.09 | 0.67 | 1.60 | 2.57 |
| | $E_{avail}$ | 0p | 1.25 | 0.65 | 0.25 | 0.05 | 0.09 | 0.41 | 0.67 | 0.09 |
| | | Np | 0.10 | 0.02 | 0.00 | 0.00 | 0.00 | 0.00 | 0.04 | 1.52 |
| | | 0pNp | 0.62 | 0.12 | 0.01 | 0.00 | 0.00 | 0.01 | 0.13 | 0.63 |
| | $K_p$ | Xp | 1.84 | 0.74 | 0.10 | 0.00 | 0.00 | 0.28 | 1.31 | 2.52 |
| Mod. Val. | Np $E_{had}^{rec}$ | FC $\chi^2$ | 0.00 | 0.00 | 0.00 | 0.00 | 0.00 | 0.00 | 0.00 | 0.00 |
| | | PC $\chi^2$ | 0.23 | 0.04 | 0.00 | 0.00 | 0.00 | 0.00 | 0.01 | 0.04 |
| | | FC&PC $\chi^2$ | 0.09 | 0.00 | 0.00 | 0.00 | 0.00 | 0.00 | 0.00 | 0.01 |
| | | FC dec. $\chi^2$ | 0.00 | 0.00 | 0.00 | 0.00 | 0.00 | 0.00 | 0.00 | 0.00 |
| | | PC dec. $\chi^2$ | 0.76 | 0.00 | 0.00 | 0.00 | 0.00 | 0.00 | 0.00 | 0.66 |
| | | FC&PC dec. $\chi^2$ | 1.43 | 0.53 | 0.00 | 0.00 | 0.00 | 0.00 | 0.56 | 1.38 |
| | $K_p^{rec}$ | FC $\chi^2$ | 3.02 | 1.33 | 0.17 | 0.00 | 0.00 | 0.31 | 2.16 | 4.05 |
| | | PC $\chi^2$ | 6.19 | 3.75 | 1.41 | 0.06 | 0.04 | 0.59 | 3.80 | 6.01 |
| | | FC&PC $\chi^2$ | 7.02 | 3.81 | 0.89 | 0.00 | 0.00 | 0.82 | 4.44 | 7.56 |
| | | FC dec. $\chi^2$ | 4.33 | 2.64 | 0.80 | 0.00 | 0.00 | 2.18 | 1.77 | 3.68 |
| | | PC dec. $\chi^2$ | 6.78 | 4.17 | 1.29 | 0.00 | 0.00 | 1.58 | 3.82 | 6.25 |
| | | FC&PC dec. $\chi^2$ | 8.37 | 5.82 | 2.39 | 0.52 | 0.44 | 0.72 | 4.42 | 7.85 |

TABLE I: Results of the model validation and cross section extraction for each $6.4 \times 10^{20}$ POT fake data set generated from the nominal MicroBooNE MC by scaling the proton energy. All sources of uncertainty are included for these test. Distinct FDS are grouped together in individual columns. The first row indicates the scaling used for the fake data tests displayed in that column. The $\sigma$ values in the XS Extr. rows indicate the level of closure the extracted fake data cross sections have with the underlying truth. The different rows correspond to different cross section measurements. The $\sigma$ values in the Mod. Val. rows indicate the level at which the fake data and the nominal MicroBooNE MC used for the extraction disagree. The rows correspond to different validation tests, all of which utilize the muon kinematics for constraint but are performed on different sets of events (FC, PC or FC&PC) or utilize different GoF tests ($\chi^2$ or decomposition $\chi^2$).

| FDS Results With MEC event weight scaling at 6.4e20 POT | | | | | | |
|---|---|---|---|---|---|---|
| | | | 0 | 0.5 | 1.5 | 2 |
| XS Extr. | $E_\nu$ | 0p | 0.00 | 0.00 | 0.00 | 0.00 |
| | | Np | 0.00 | 0.00 | 0.00 | 0.00 |
| | | 0pNp | 0.00 | 0.00 | 0.00 | 0.00 |
| | $\nu$ | 0p | 0.03 | 0.00 | 0.00 | 0.03 |
| | | Np | 0.18 | 0.01 | 0.01 | 0.17 |
| | | 0pNp | 0.17 | 0.00 | 0.00 | 0.16 |
| | $E_{avail}$ | 0p | 0.02 | 0.00 | 0.00 | 0.02 |
| | | Np | 0.13 | 0.00 | 0.00 | 0.13 |
| | | 0pNp | 0.02 | 0.00 | 0.00 | 0.01 |
| | $K_p$ | Xp | 1.10 | 0.17 | 0.17 | 1.08 |
| | P. mult | Xp | 0.00 | 0.00 | 0.00 | 0.00 |
| Mod. Val. | Np $\cos\theta_\mu^{rec}$ | 0p $\chi^2$ | 0.00 | 0.00 | 0.00 | 0.00 |
| | | Np $\chi^2$ | 0.64 | 0.00 | 0.00 | 0.62 |
| | | 0p&Np $\chi^2$ | 0.00 | 0.00 | 0.00 | 0.00 |
| | | 0p dec. $\chi^2$ | 1.16 | 0.00 | 0.00 | 1.15 |
| | | Np dec. $\chi^2$ | 3.27 | 0.54 | 0.53 | 3.25 |
| | | 0p&Np dec. $\chi^2$ | 2.94 | 0.00 | 0.00 | 2.93 |
| | $K_p^{rec}$ | FC $\chi^2$ | 0.10 | 0.00 | 0.00 | 0.07 |
| | | PC $\chi^2$ | 1.14 | 0.00 | 0.00 | 1.09 |
| | | FC&PC $\chi^2$ | 0.95 | 0.00 | 0.00 | 0.92 |
| | | FC dec. $\chi^2$ | 2.29 | 0.00 | 0.00 | 2.14 |
| | | PC dec. $\chi^2$ | 1.64 | 0.00 | 0.00 | 1.55 |
| | | FC&PC dec. $\chi^2$ | 3.16 | 0.00 | 0.00 | 3.14 |

TABLE II: Same as Table I, but for fake data sets generated by scaling MEC event weights in the nominal MicroBooNE MC: Results of the model validation and cross section extraction for each $6.4 \times 10^{20}$ POT fake data set generated from the nominal MicroBooNE MC by scaling MEC event weights. All sources of uncertainty are included for these test. Distinct FDS are grouped together in individual columns. The first row indicates the scaling used for the fake data tests displayed in that column. The $\sigma$ values in the XS Extr. rows indicate the level of closure the extracted fake data cross sections have with the underlying truth. The $\sigma$ values in the Mod. Val. rows indicate the level at which the fake data and the nominal MicroBooNE MC used for the extraction disagree. The rows correspond to different validation tests. The test on $\cos\theta_\mu^{rec}$ utilize the FC distribution to constraint the PC distribution and the test on $K_p^{rec}$ utilize the muon kinematics for constraint. Different rows correspond to tests performed on different sets of events (0p, Np or 0p&Np for $\cos\theta_\mu^{rec}$, and FC, PC or FC&PC for $K_p^{rec}$) or utilize different GoF tests ($\chi^2$ or decomposition $\chi^2$).

An analogous set of FDS were performed on fake data sets generated in the same way as above, but with the scaling factor applied to MEC events weights instead. This mimics a situation where the MEC contribution to the cross section is significantly larger or smaller than predicted by the MicroBooNE model. These FDS are likewise performed with full systematics to properly probe the sensitivity of the model validation. Closure is achieved when the fake data cross section extraction reproducing the MicroBooNE MC cross section prediction with the appropriate scaling applied to MEC events. The results of these FDS are presented in Fig. 4(b) and Table II in the same format as the ones described above. These studies likewise indicate that for all cross section extractions, there are model validation tests with larger $\sigma$ values (i.e. more sensitive to the defect of the model). Furthermore, even at significant MEC scalings far past the point at which the validation indicates that there may be relevant mismodeling, the agreement between the underlying truth and extracted results remains quite good. These observations support the notion that the stringency of the model validation is equal to or greater than the bias in the cross section extraction induced by mismodeling. Alongside the FDS presented in [1], these tests give us confidence that the methodology used for model validation and expansion is capable of detecting and mitigating mismodeling relevant to the cross section extraction, thus minimizing the possibility of extracting biased cross section results due to model dependence or insufficient uncertainties.

As a validation of the reweighting uncertainty described in Sec. VII of the main text, we perform an additional FDS in which the fake data set is generated by applying the reweighting function to the CV $\mu$`BooNE` tune prediction. Statistical fluctuations at $6.4{\times}10^{20}$ POT are then added to the reconstructed fake data distributions. These are then unfolded using the nominal $\mu$`BooNE` tune MC prediction considering only statistical and the reweighting uncertainties.

Comparisons to the nominal $\mu$`BooNE` tune MC prediction and the reweighted one, which corresponds to the truth in this study, are shown in Table III. Plots of $E_\nu$ and $\nu$ are also shown in Figs. 5 and 6 as representative examples. We see in these examples that the reweighting uncertainty is indeed able to cover the reweighted model at $1\sigma$, as intended by the construction of the reweighting function. The extremely large $\chi^2$ values obtained for the nominal model emphasizes the stringency of these tests.

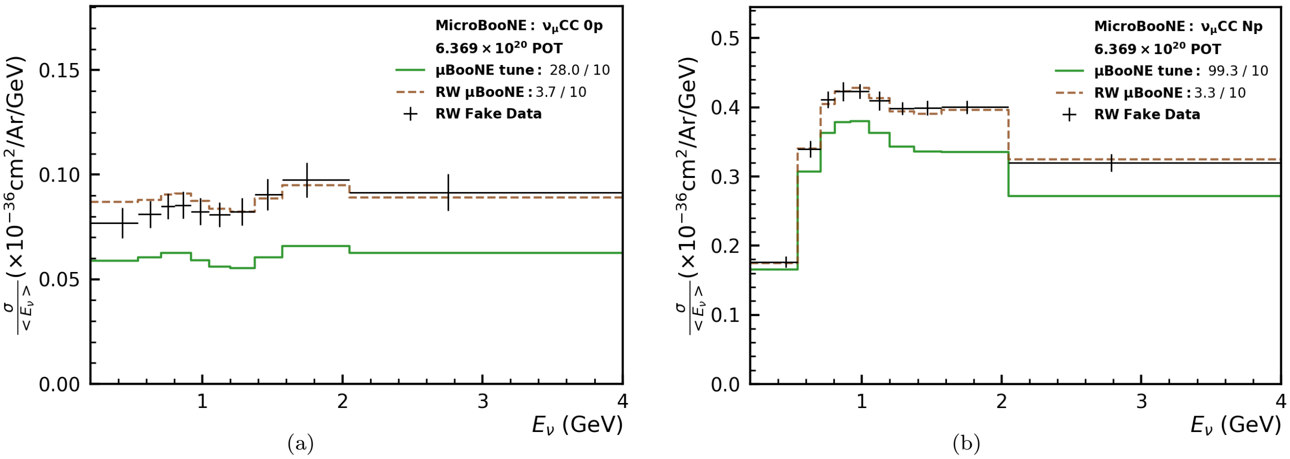


(a) (b)

FIG. 5: Unfolded 0pNp $E_\nu$ differential cross section results for fake data obtained from the reweighing function. The 0p result is shown in (a) and the Np result is shown in (b). Only the reweighting uncertainty is included in the unfolding and subsequent $\chi^2$ comparisons.

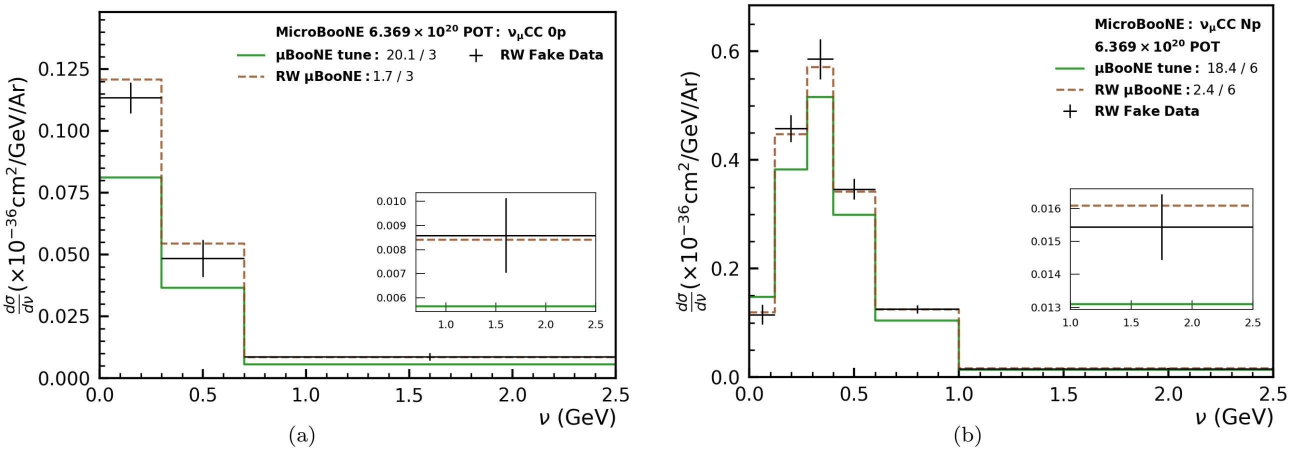


(a) (b)

FIG. 6: Unfolded 0pNp $\nu$ differential cross section results for fake data obtained from the reweighing function. The 0p result is shown in (a) and the Np result is shown in (b). Only the reweighting uncertainty is included in the unfolding and subsequent $\chi^2$ comparisons.

| Measurement | | *ndf* | Reweighted (truth) | $\mu$BooNE tune (nominal) |
|---|---|---|---|---|
| $\frac{d\sigma}{dE_\mu}$ | 0p | 11 | 9.8 | 14.6 |
| | Np | 11 | 7.2 | 17.4 |
| | 0pNp | 22 | 20.0 | 896.2 |
| $\frac{d\sigma}{d\cos\theta_\mu}$ | 0p | 17 | 15.9 | 24.8 |
| | Np | 17 | 9.2 | 130.4 |
| | 0pNp | 34 | 20.0 | 739.4 |
| $\frac{d\sigma}{d\nu}$ | 0p | 3 | 1.7 | 20.1 |
| | Np | 6 | 2.4 | 18.4 |
| | 0pNp | 9 | 3.2 | 976.8 |
| $\frac{d\sigma}{dE_{avail}}$ | 0p | 5 | 4.8 | 26.4 |
| | Np | 9 | 6.0 | 202.6 |
| | 0pNp | 14 | 7.1 | 851.7 |
| $\sigma(E_\nu)$ | 0p | 10 | 3.7 | 28.0 |
| | Np | 10 | 3.3 | 99.3 |
| | 0pNp | 20 | 9.3 | 1234.9 |
| $\frac{d\sigma}{dK_p}$ | Xp | 15 | 10.7 | 993.9 |
| $\frac{d\sigma}{d\cos\theta_p}$ | Np | 20 | 11.7 | 107.1 |
| Proton Multiplicity | Xp | 4 | 1.8 | 202.2 |
| $\frac{d^2\sigma}{d\cos\theta_\mu dE_\mu}$ | 0p | 55 | 49.1 | 315.5 |
| | Np | 69 | 63.9 | 1059.4 |
| | 0pNp | 124 | 101.8 | 1177.0 |
| $\frac{d^2\sigma}{d\cos\theta_p dK_p}$ | Np | 96 | 64.7 | 997.5 |
| $\frac{d^3\sigma}{dE_{avail} d\cos\theta_\mu dE_\mu}$ | Xp | 249 | 174.3 | 1377.9 |

TABLE III: Summary of the comparisons between the reweighted $\mu$BooNE tune prediction and the extracted results from fake data produced with the reweighting function. Only the reweighting uncertainty is included. A comparison against the $\mu$BooNE tune without reweighting is shown for comparison. When applicable, the 0p, Np, 0pNp and Xp $\chi^2$ and respective *ndf* are shown for each measured variable. When a 0p row is present for a variable, the 0p and Np cross sections are extracted simultaneously. As such, the 0p (Np) $\chi^2$ value is calculated using only the 0p (Np) bins. The 0pNp $\chi^2$ is calculated using both sets of bins and accounts for the correlations between the two channels due to the form of Eq. (2) in the main text.

## III. 2D AND 3D RECONSTRUCTED DISTRIBUTIONS

This section contains the results of the $\nu_\mu$CC event selection for the 2D $\{\cos\theta_p^{rec} K_p^{rec}\}$, 2D 0pNp $\{\cos\theta_\mu^{rec}, E_\mu^{rec}\}$, and 3D $\{E_{avail}^{rec}, \cos\theta_\mu^{rec}, E_\mu^{rec}\}$ distributions. The binning used for these plots is the same as used for $M$ in the cross section extraction. Both data and MC are shown. More details on these MC predictions can be found in Sec. V A of the main text. The event breakdown categories for the MC are identical to those described in Sec. IV D of the main text. The full nominal uncertainty, as is used for the model validation and including the additional reweighting systematic described in Sec. VII of the main text, is included on the MC and the $\chi^2$ in the legend of each plot is calculated with the corresponding covariance matrix. The number of degrees of freedom, $ndf$, is equal to the number of bins, including the overflow. Good agreement between the data and MC prediction is seen in all distributions with each $\chi^2/ndf$ value being below unity.

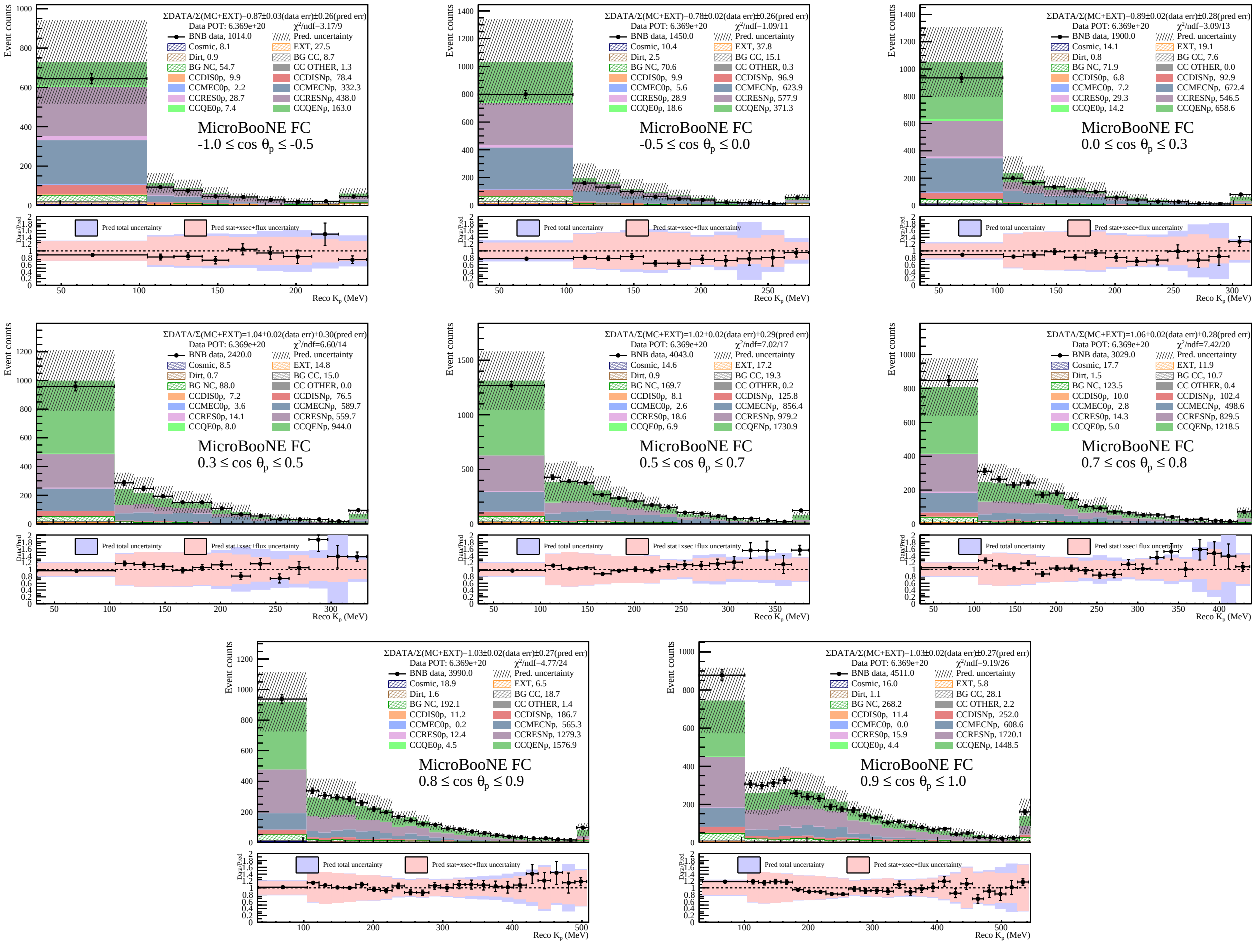


FIG. 7: The $\nu_\mu$CC Np selection as a function of $K_p^{rec}$ in $\cos\theta_p^{rec}$ slices for FC events. The MC prediction is categorized by interaction types with separate categories for true 0p and Np events. The binning is the same as for $M$ in the cross section extraction and the last bin of each slice corresponds to overflow. In the bottom sub-panels, the pink band includes the statistical, cross section, flux uncertainties and the additional reweighting systematic discussed in Sec. VII of the main text, and the purple band corresponds to the full uncertainty with the addition of the detector systematic uncertainty. Data statistical errors are shown on the data points.

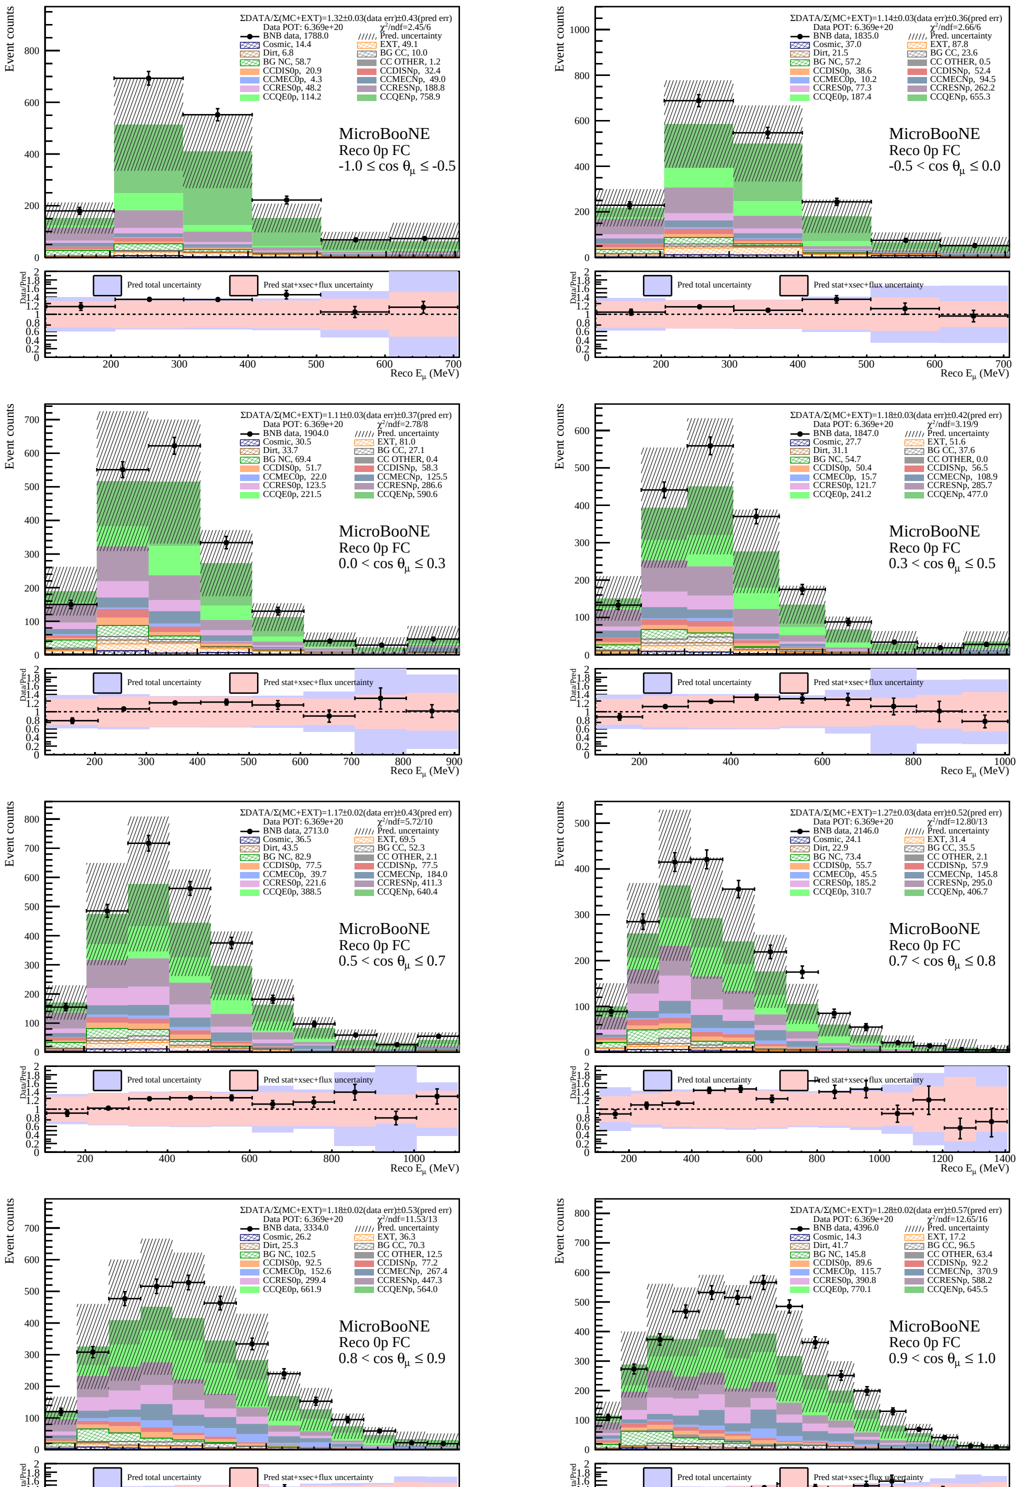


FIG. 8: The $\nu_\mu$CC 0p selection as a function of $E_\mu^{rec}$ in $\cos\theta_\mu^{rec}$ slices for FC events. The MC prediction is categorized by interaction types with separate categories for true 0p and Np events. The binning is the same as for $M$ in the cross section extraction and the last bin of each slice corresponds to overflow. In the bottom sub-panels, the pink band includes the statistical, cross section, flux uncertainties and the additional reweighting systematic discussed in Sec. VII of the main text, and the purple band corresponds to the full uncertainty with the addition of the detector systematic uncertainty. Data statistical errors are shown on the data points.

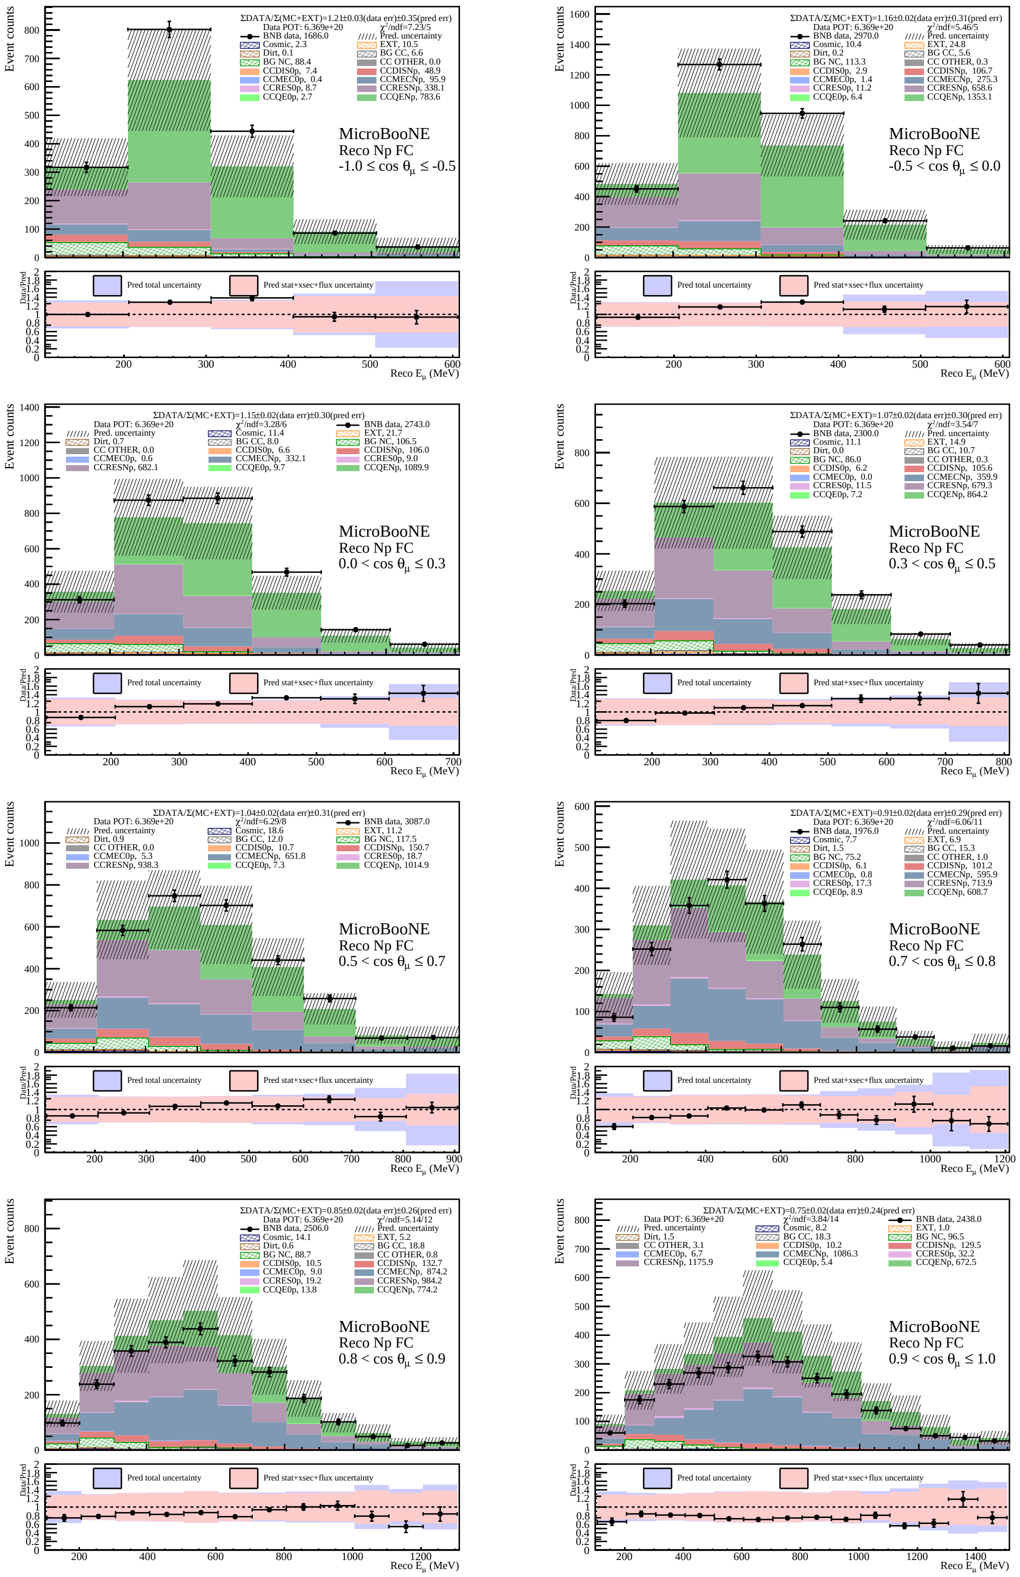


FIG. 9: The $\nu_\mu$CC Np selection as a function of $E_\mu^{rec}$ in $\cos\theta_\mu^{rec}$ slices for FC events. The MC prediction is categorized by interaction types with separate categories for true 0p and Np events. The binning is the same as for $M$ in the cross section extraction and the last bin of each slice corresponds to overflow. In the bottom sub-panels, the pink band includes the statistical, cross section, flux uncertainties and the additional reweighting systematic discussed in Sec. VII of the main text, and the purple band corresponds to the full uncertainty with the addition of the detector systematic uncertainty. Data statistical errors are shown on the data points.

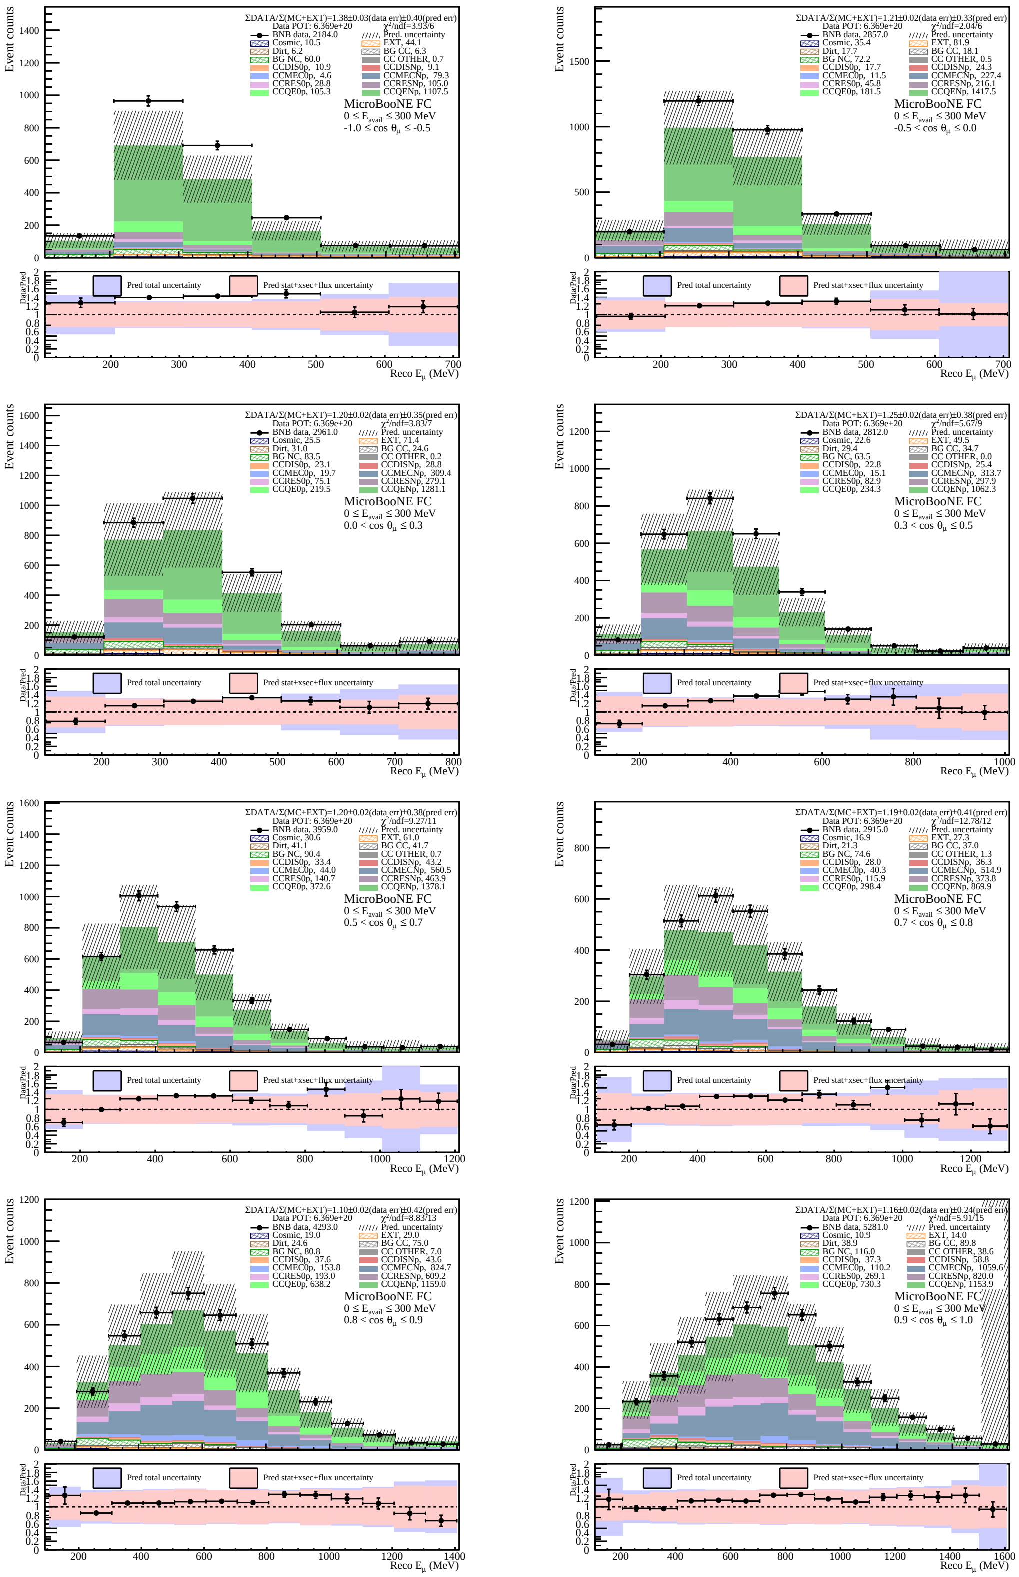


FIG. 10: The $\nu_\mu$CC selection as a function of $E_\mu^{rec}$ in $\cos\theta_\mu^{rec}$ slices for FC events with $0 \leq E_{avail}^{rec} \leq 300$ MeV. The MC prediction is categorized by interaction types with separate categories for true 0p and Np events. The binning is the same as for $M$ in the cross section extraction and the last bin of each slice corresponds to overflow. In the bottom sub-panels, the pink band includes the statistical, cross section, flux uncertainties and the additional reweighting systematic discussed in Sec. VII of the main text, and the purple band corresponds to the full uncertainty with the addition of the detector systematic uncertainty. Data statistical errors are shown on the data points.

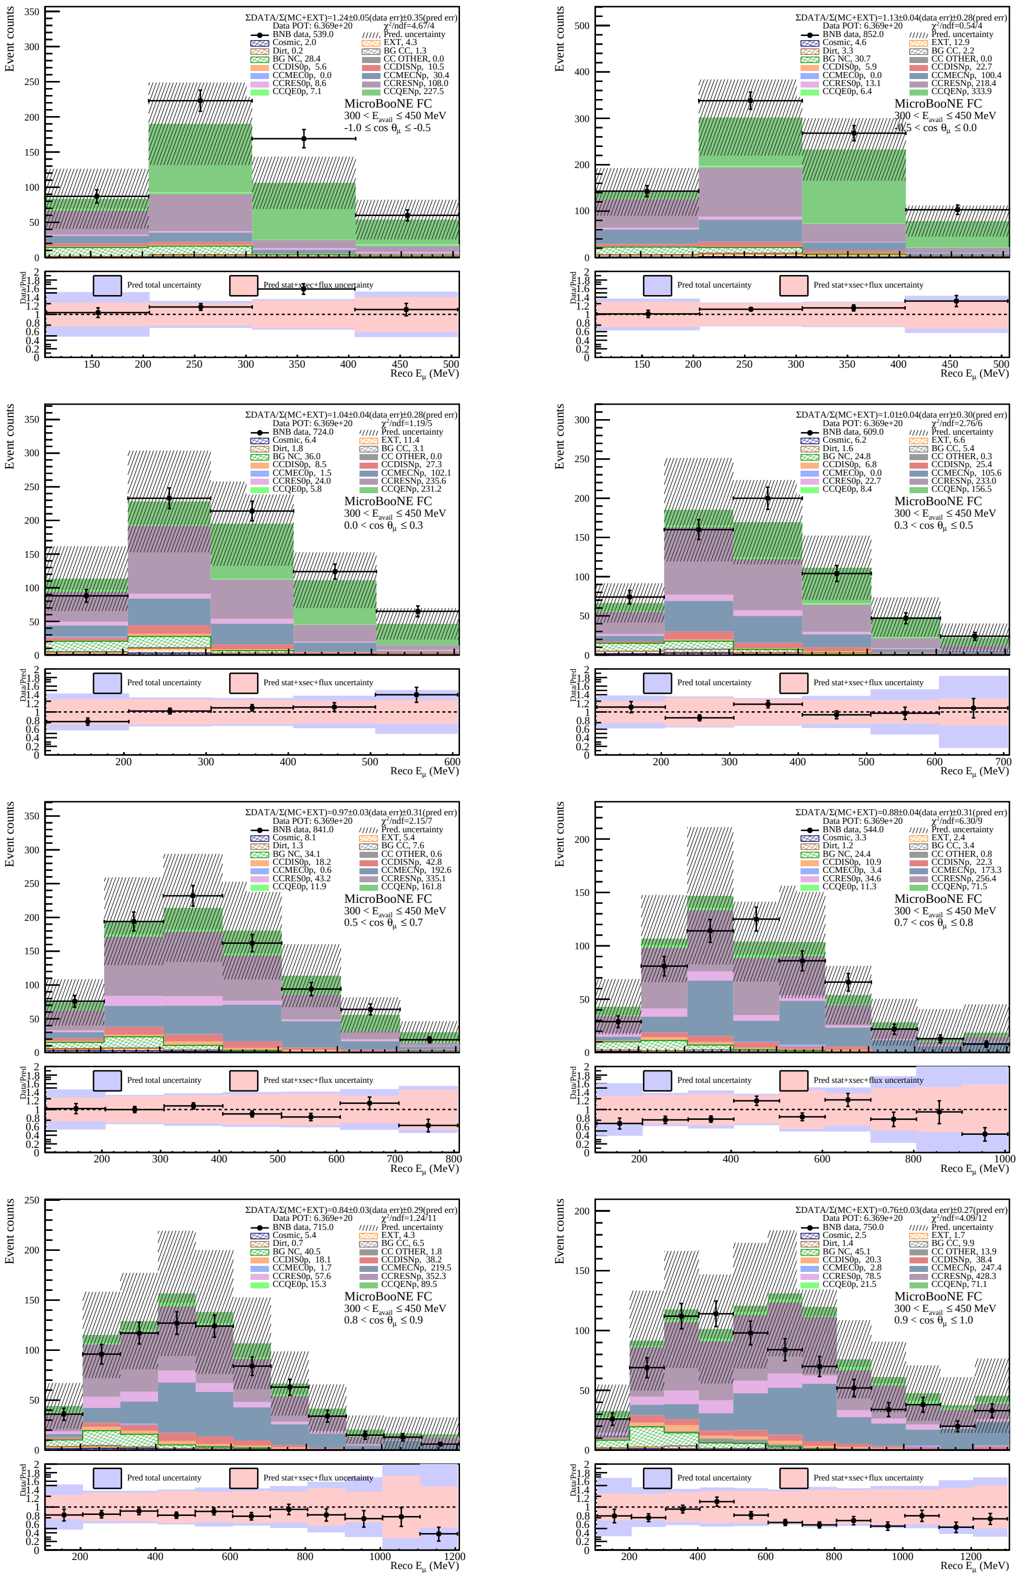


FIG. 11: The $\nu_\mu$CC selection as a function of $E_\mu^{rec}$ in $\cos\theta_\mu^{rec}$ slices for FC events with $300 < E_{avail}^{rec} \leq 450$ MeV. The MC prediction is categorized by interaction types with separate categories for true 0p and Np events. The binning is the same as for $M$ in the cross section extraction and the last bin of each slice corresponds to overflow. In the bottom sub-panels, the pink band includes the statistical, cross section, flux uncertainties and the additional reweighting systematic discussed in Sec. VII of the main text, and the purple band corresponds to the full uncertainty with the addition of the detector systematic uncertainty. Data statistical errors are shown on the data points.

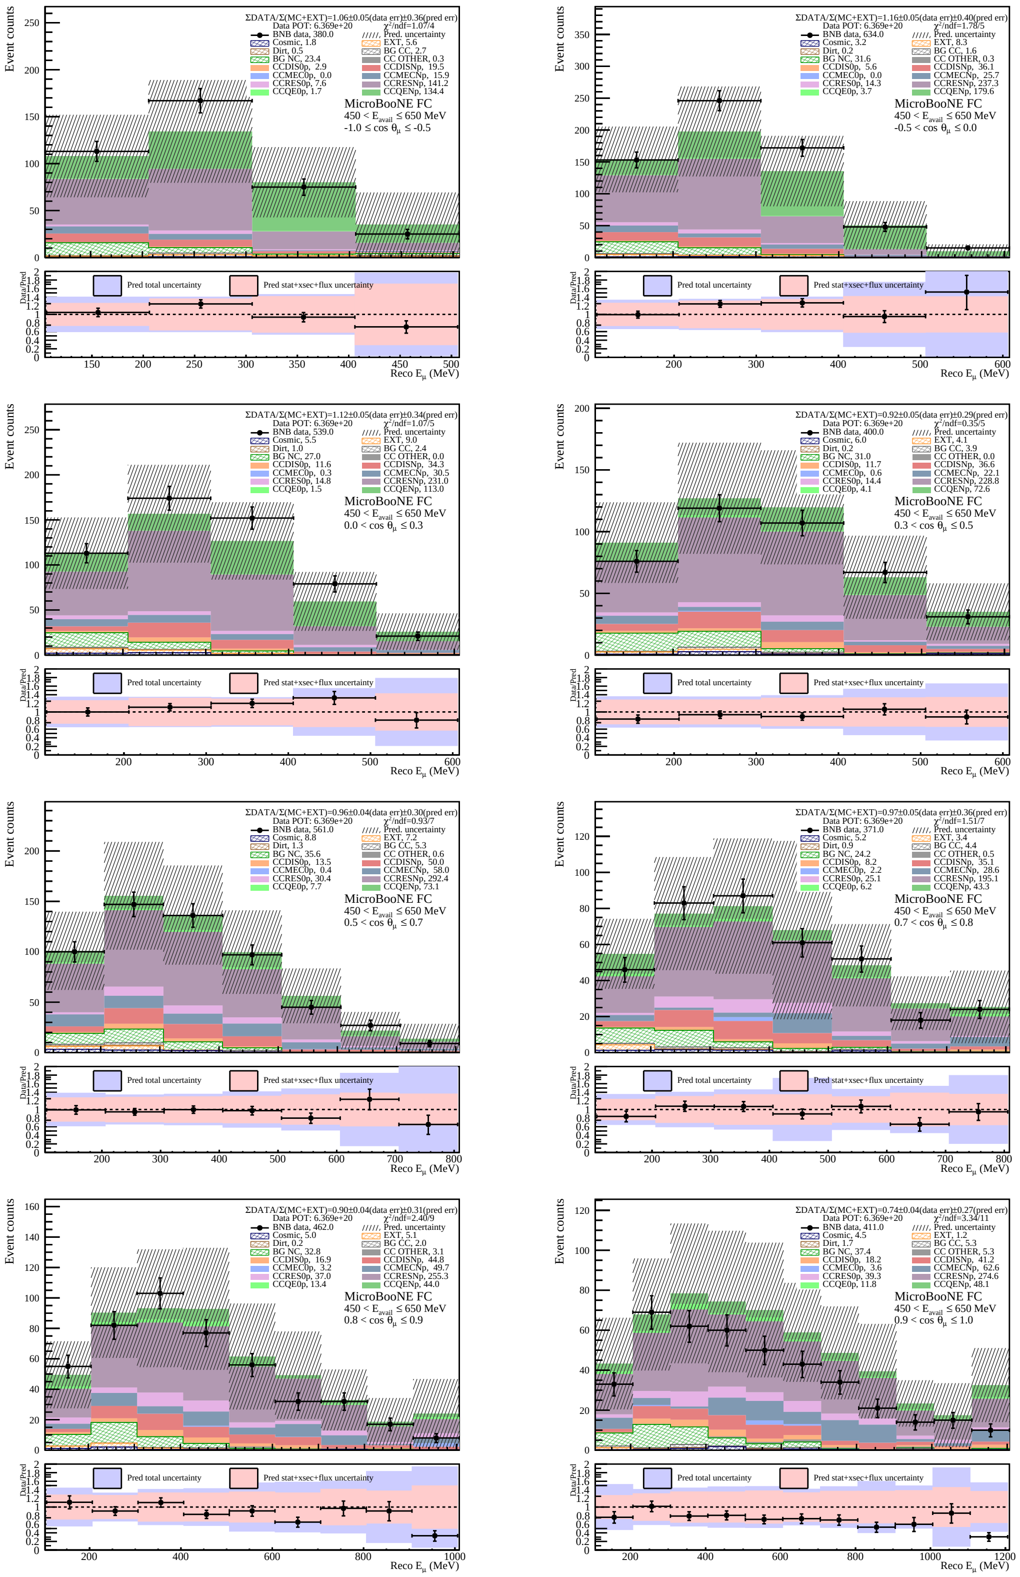


FIG. 12: The $\nu_\mu$CC selection as a function of $E_\mu^{rec}$ in $\cos\theta_\mu^{rec}$ slices for FC events with $450 < E_{avail}^{rec} \leq 650$ MeV. The MC prediction is categorized by interaction types with separate categories for true 0p and Np events. The binning is the same as for $M$ in the cross section extraction and the last bin of each slice corresponds to overflow. In the bottom sub-panels, the pink band includes the statistical, cross section, flux uncertainties and the additional reweighting systematic discussed in Sec. VII of the main text, and the purple band corresponds to the full uncertainty with the addition of the detector systematic uncertainty. Data statistical errors are shown on the data points.

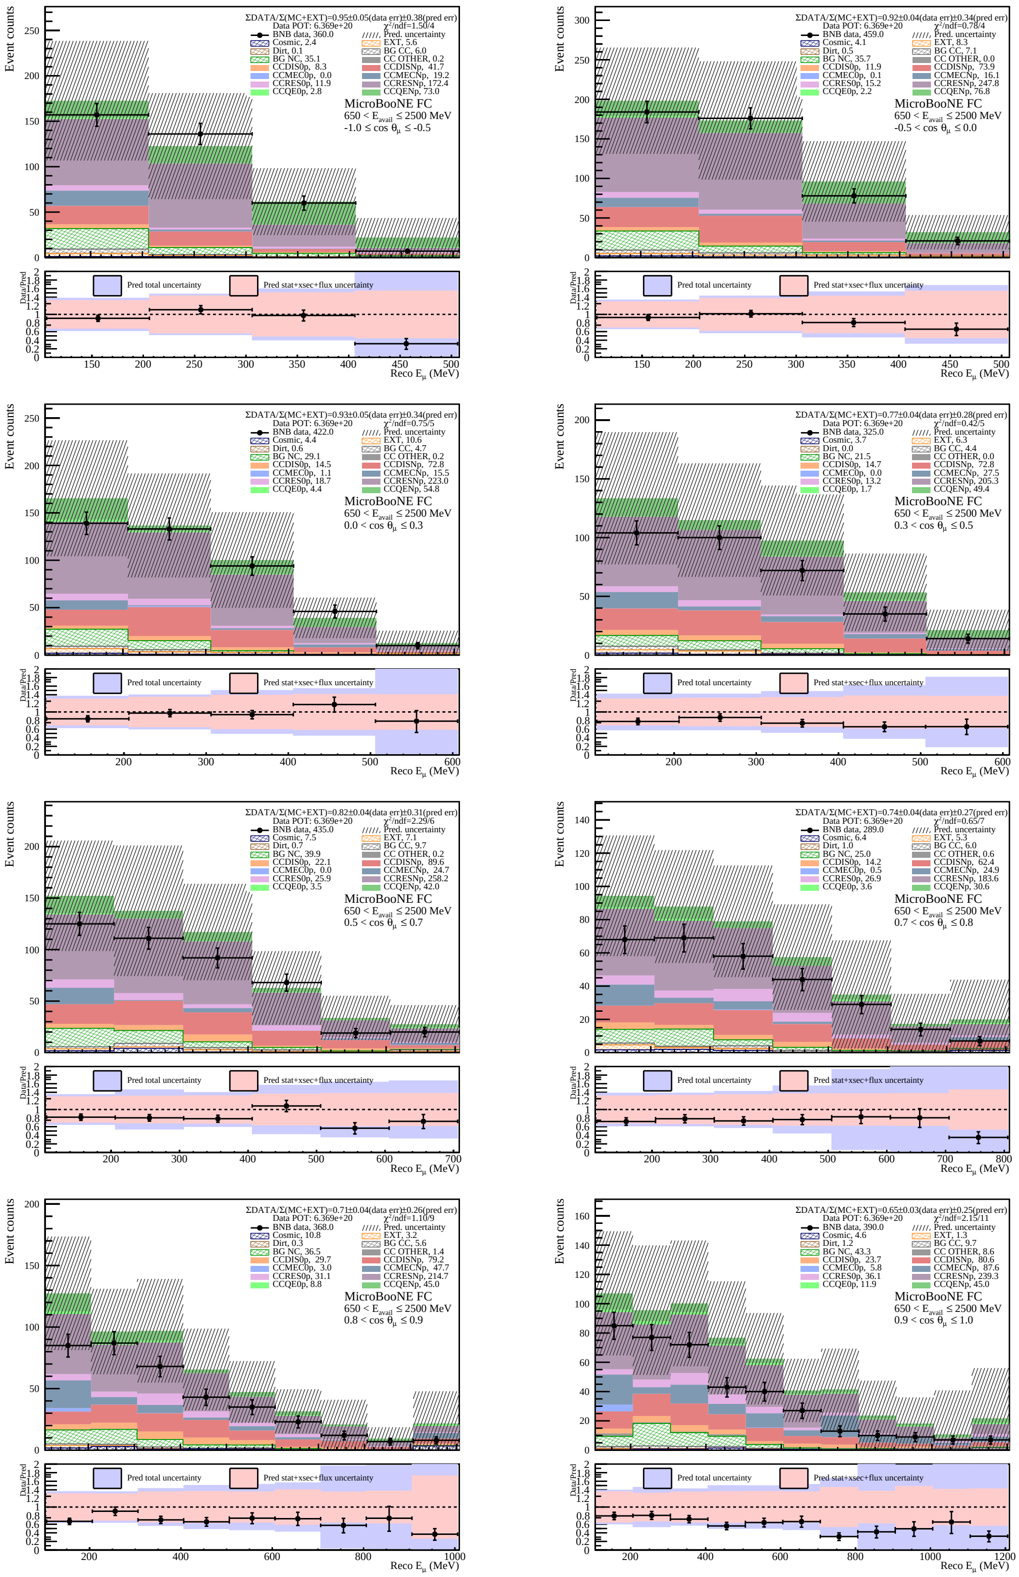


FIG. 13: The $\nu_\mu$CC selection as a function of $E_\mu^{rec}$ in $\cos\theta_\mu^{rec}$ slices for FC events with $450 < E_{avail}^{rec} \leq 2500$ MeV. The MC prediction is categorized by interaction types with separate categories for true 0p and Np events. The binning is the same as for $M$ in the cross section extraction and the last bin of each slice corresponds to overflow. In the bottom sub-panels, the pink band includes the statistical, cross section, flux uncertainties and the additional reweighting systematic discussed in Sec. VII of the main text, and the purple band corresponds to the full uncertainty with the addition of the detector systematic uncertainty. Data statistical errors are shown on the data points.

## IV. ADDITIONAL MODEL VALIDATION PLOTS

This section contains a variety of additional model validation plots which were discussed in Sec. VI but not shown in the main text.

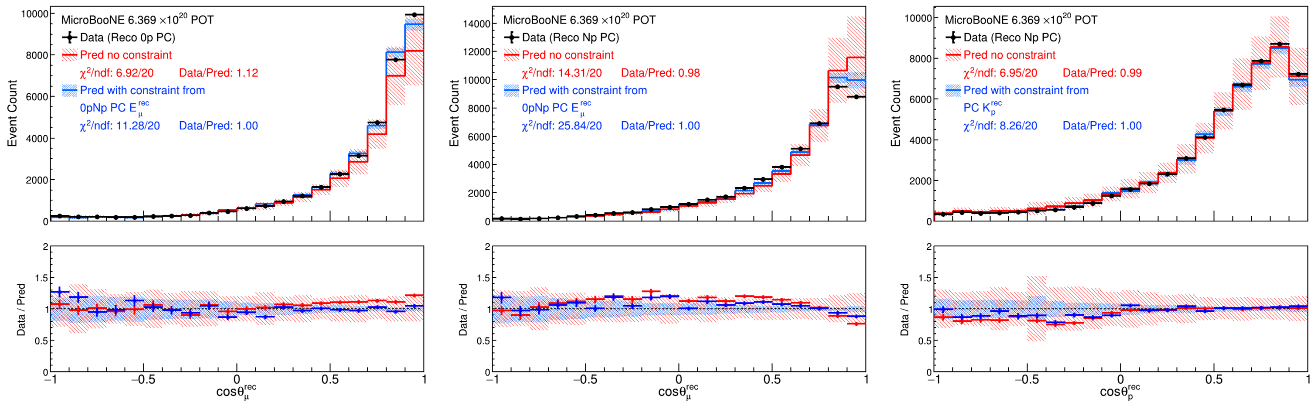


(a) Reconstructed 0p PC muon angle constrained by the reconstructed 0pNp PC muon energy.

(b) Reconstructed Np PC muon angle constrained by the reconstructed 0pNp PC muon energy.

(c) Reconstructed Np PC leading proton angle constrained by the PC leading proton kinetic energy.

FIG. 14: Comparison between data and prediction as a function of the [(a) and (b)] reconstructed muon angle and (c) reconstructed proton angle for PC events. For the muon angle, the 0p selection is seen in (a) and the Np selection is seen in (b). The red (blue) lines and bands show the prediction without (with) the constraint. In (a) and (b) the constraint is from the reconstructed 0pNp PC muon energy distributions and in (c) the constraint is from PC leading proton kinetic energy distribution. The statistical and systematic uncertainties of the Monte Carlo are shown in the bands. The data statistical errors are shown on the data points and are often too small to be seen.

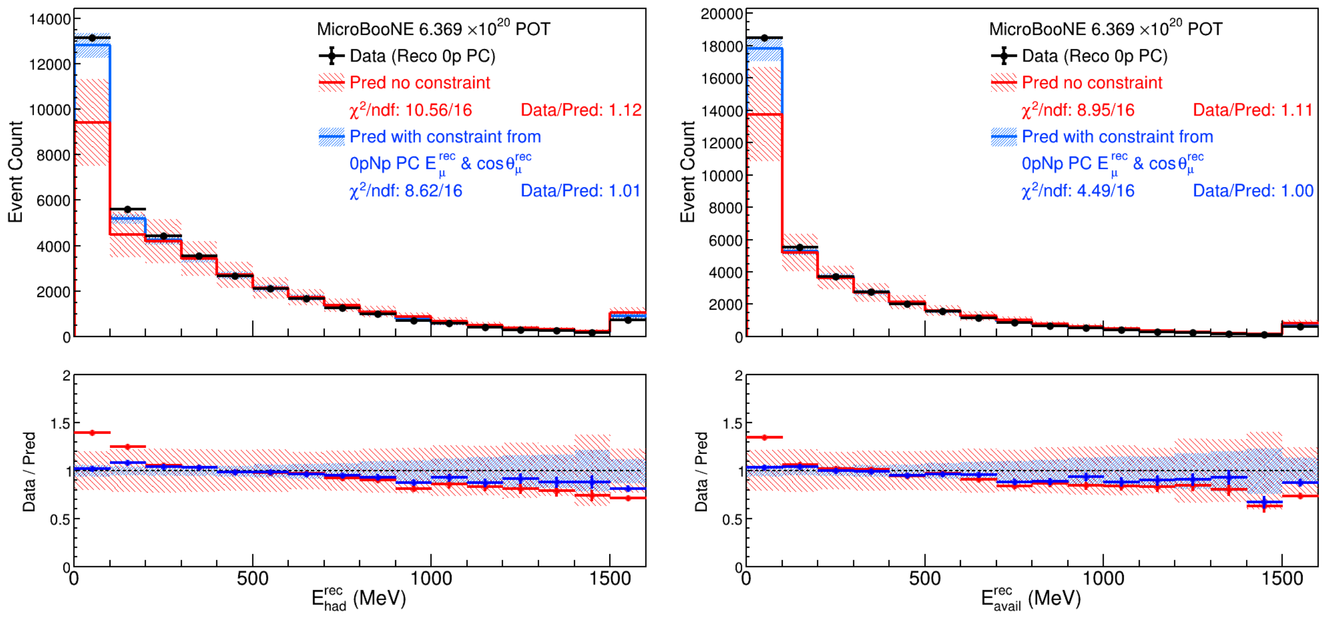


(a) Reconstructed 0p PC reconstructed hadronic energy constrained by reconstructed 0pNp PC reconstructed muon kinematics.

(b) Reconstructed 0p PC reconstructed available energy constrained by reconstructed 0pNp PC reconstructed muon kinematics.

FIG. 15: Comparison between data and prediction as a function of the (a) reconstructed hadronic energy and (b) reconstructed available energy for PC events in the 0p selection. The last bin corresponds to overflow. The red (blue) lines and bands show the prediction without (with) the constraint from the reconstructed 0pNp FC muon energy and muon angle distributions. The statistical and systematic uncertainties of the Monte Carlo are shown in the bands. The data statistical errors are shown on the data points and are often too small to be seen.

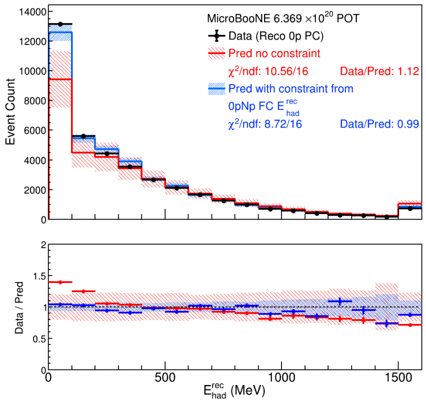


(a) Reconstructed 0p PC reconstructed hadronic energy constrained by 0pNp FC reconstructed hadronic energy.

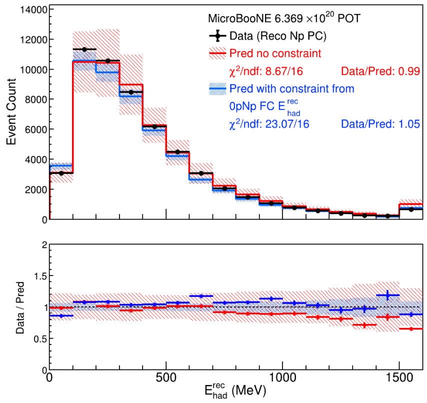


(b) Reconstructed Np PC reconstructed hadronic energy constrained by 0pNp FC reconstructed hadronic energy.

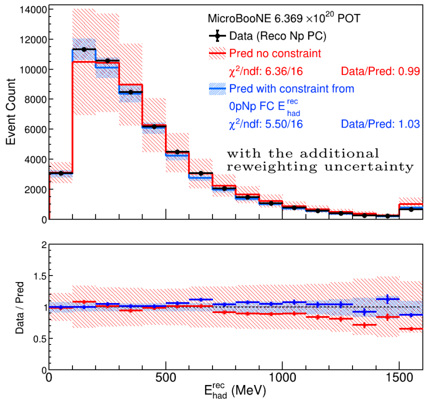


(c) Reconstructed Np PC reconstructed hadronic energy constrained by 0pNp FC reconstructed hadronic energy.

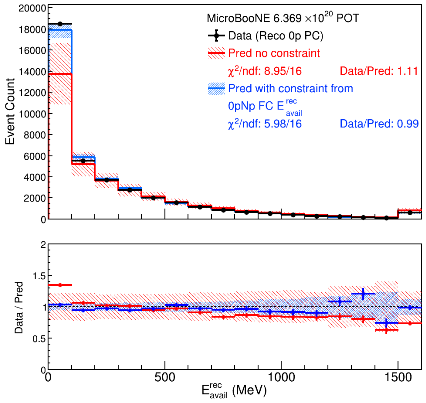


(d) Reconstructed 0p PC reconstructed available energy constrained by 0pNp FC reconstructed available energy.

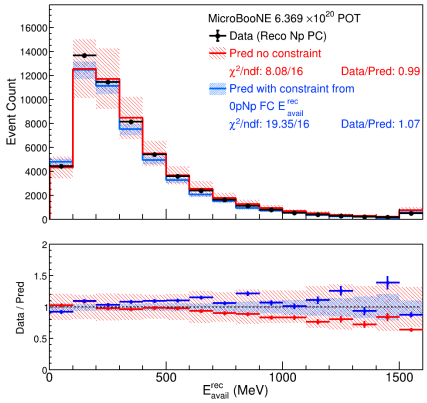


(e) Reconstructed Np PC reconstructed available energy constrained by 0pNp FC reconstructed available energy.

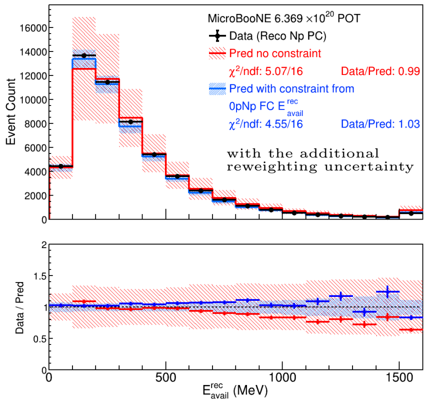


(f) Reconstructed Np PC reconstructed available energy constrained by 0pNp FC reconstructed available energy.

FIG. 16: Comparison between data and MC prediction as a function of the [(a), (b) and (c)] reconstructed hadronic energy, and [(d), (e) and (f)] reconstructed available energy. The 0p selection is shown in (a) and (d), and the Np selection is shown in (b), (c), (e), and (f). The additional reweighting uncertainty is only included on (c) and (f). In all plots, the last bin corresponds to overflow. The red (blue) lines and bands show the prediction without (with) the constraint from the [(a), (b) and (c)] reconstructed 0pNp FC reconstructed hadronic energy distributions or the [(d), (e) and (f)] reconstructed 0pNp FC reconstructed available energy distributions. The statistical and systematic uncertainties of the Monte Carlo are shown in the bands. The data statistical errors are shown on the data points and are often too small to be seen.

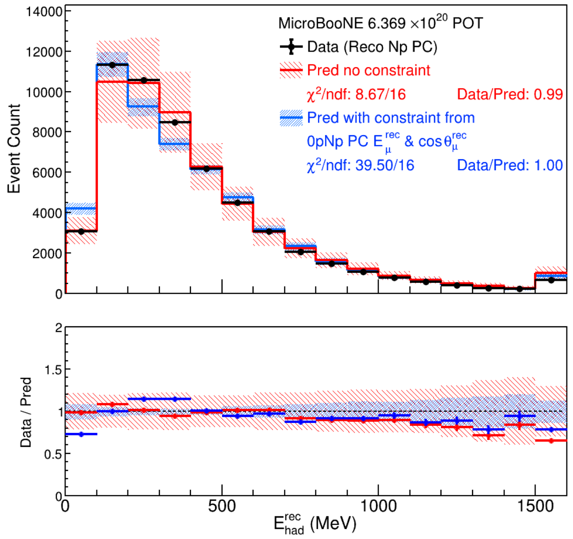


(a) Reconstructed Np PC hadronic energy constrained by reconstructed 0pNp PC muon kinematics.

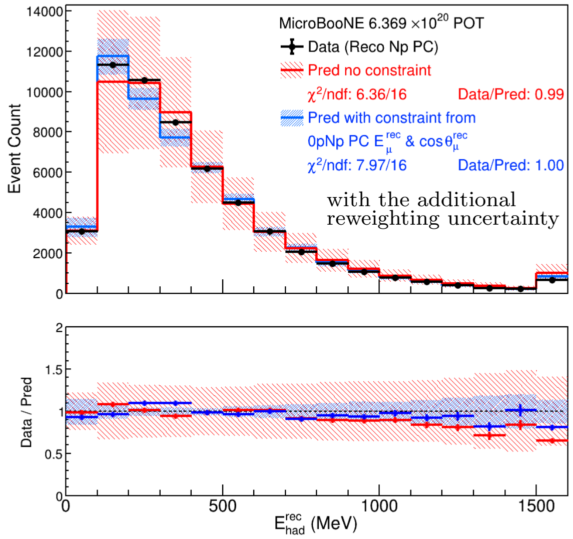


(b) Reconstructed Np PC hadronic energy constrained by reconstructed 0pNp PC muon kinematics.

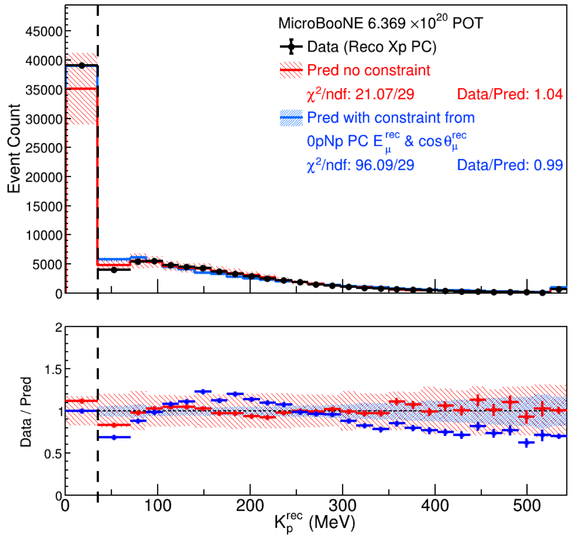


(c) Reconstructed PC leading proton kinetic energy constrained by reconstructed 0pNp PC muon kinematics.

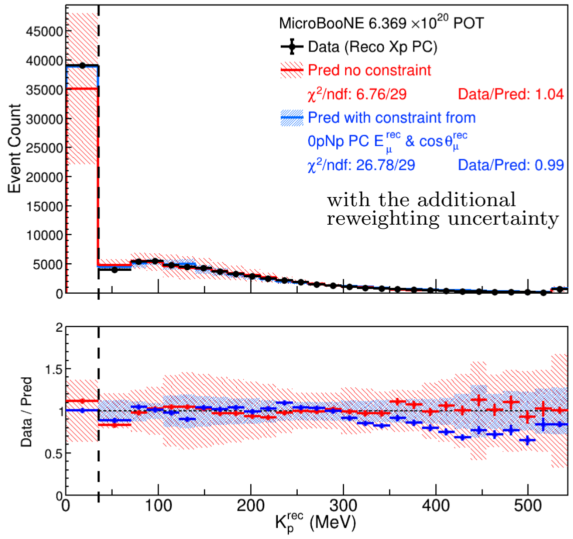


(d) Reconstructed PC leading proton kinetic energy constrained by reconstructed 0pNp PC muon kinematics.

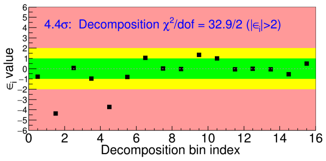


(e) Decomposition $\chi^2$ for (a).

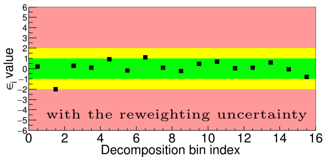


(f) Decomposition $\chi^2$ for (b).

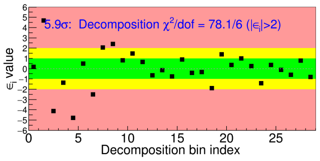


(g) Decomposition $\chi^2$ for (c).

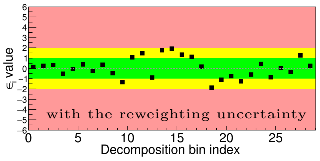


(h) Decomposition $\chi^2$ for (d).

FIG. 17: Comparison between data and prediction for the [(a),(b), (e), and (f)] reconstructed hadronic energy distribution and [(c), (d), (g), and (h)] reconstructed leading proton kinetic energy distribution for PC events. The additional reweighting systematic uncertainty is only included in (b), (d), (f), and (h). In (a)-(d), the distribution is shown in reconstructed space and the last bin corresponds to overflow. The red (blue) lines and bands show the prediction without (with) the constraint from the reconstructed 0pNp PC muon energy and muon angle distributions. The dashed line in (c) and (d) indicates the 35 MeV proton tracking threshold, below which is a single bin that includes events with no protons and events where the leading proton is below the threshold. The statistical and systematic uncertainties of the Monte Carlo are shown in the bands. The data statistical errors are shown on the data points and are often too small to be seen due to high event counts. In (e)-(h), the significance of the data to MC disagreement is shown in each independent bin after the conditional constraint and transformation to the independent basis via eigenvalue decomposition of the covariance matrix. In (e) and (h), where the reweighting systematic is not included, several of the $\epsilon_i$ fall well outside of $2\sigma$ and the $p_{\mathrm{global}}$ calculated from the $p_{\mathrm{local}}$, displayed in blue on top of the plots, indicates poor agreement. The $p_{\mathrm{global}}$ are in terms of $\sigma$ values assuming one degree of freedom and the $p_{\mathrm{local}}$ are in terms of $\chi^2/ndf$, where $ndf$ correspond to the number of extreme points.

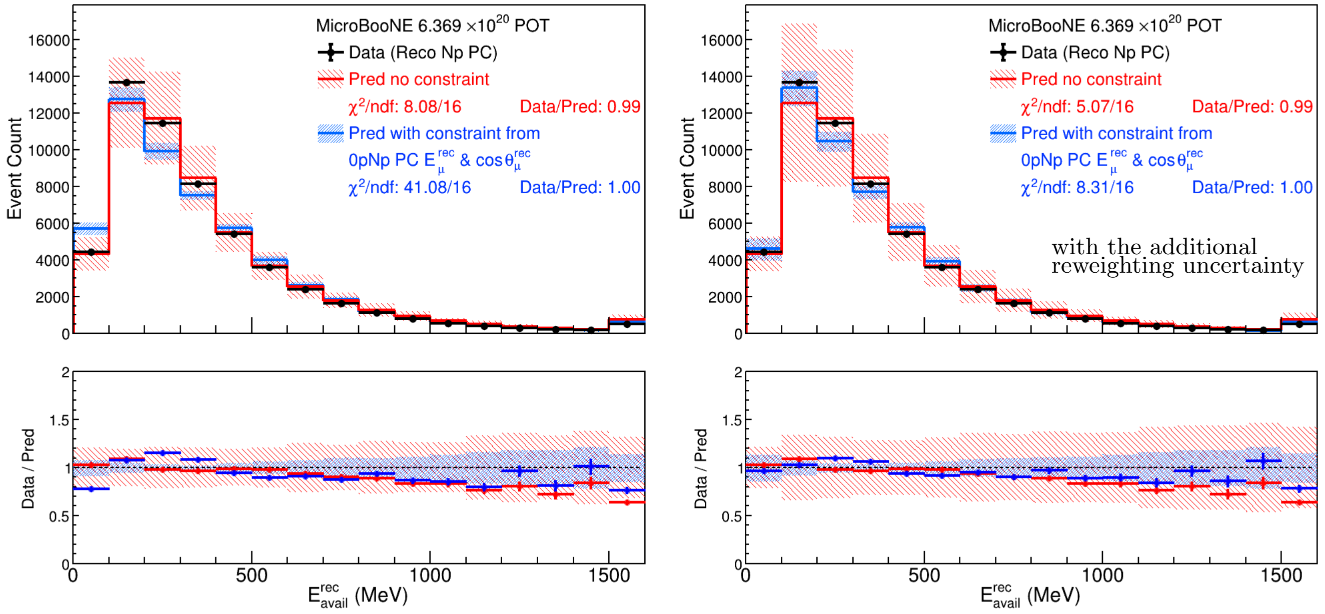


(a) Reconstructed Np PC available energy constrained by reconstructed 0pNp PC muon kinematics.

(b) Reconstructed Np PC available energy constrained by reconstructed 0pNp PC muon kinematics.

FIG. 18: Comparison between data and prediction as a function of the reconstructed available energy for PC events. The additional reweighting uncertainties included in (b). In all plots, the last bin corresponds to overflow. The red (blue) lines and bands show the prediction without (with) the constraint from the reconstructed 0pNp PC muon energy and muon angle distributions. The statistical and systematic uncertainties of the Monte Carlo are shown in the bands. The data statistical errors are shown on the data points and are often too small to be seen.

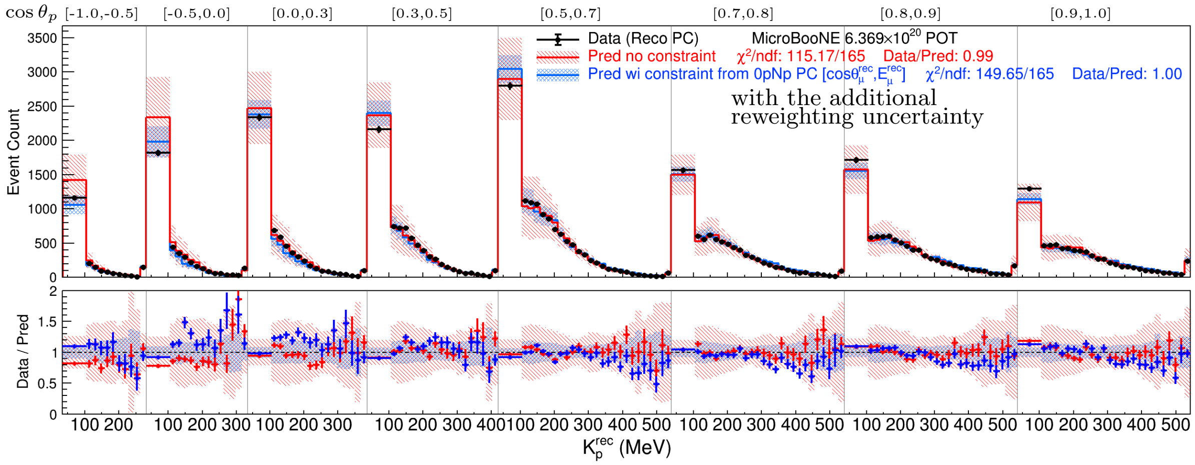


FIG. 19: Comparison between data and prediction with the additional systematic derived from the reweighting as a function of the reconstructed leading proton kinetic energy in proton angle slices for PC events. The angular slices are divided by the gray lines and go from backwards on the left to forwards on the right with the last bin in each slice corresponding to overflow. No 0p bin is included; the proton angle is not applicable for 0p events. The red (blue) lines and bands show the prediction without (with) the constraint from the reconstructed 0pNp PC $\{\cos\theta_\mu^{rec}, E_\mu^{rec}\}$ distribution. The statistical and systematic uncertainties (including the additional reweighting uncertainty) of the Monte Carlo are shown in the bands. The data statistical errors are shown on the data points.

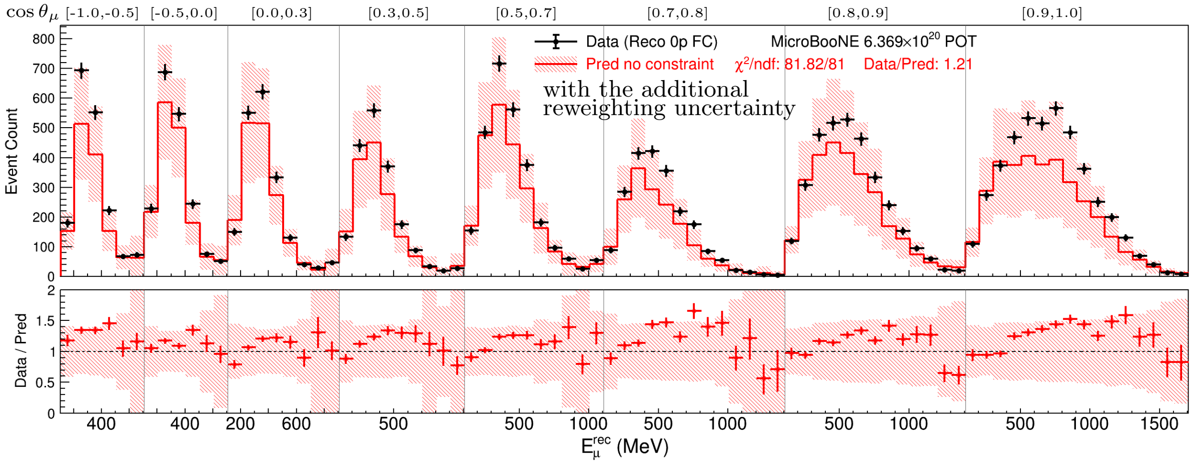


(a) Reconstructed 0p FC muon energy distribution sliced in the muon angle.

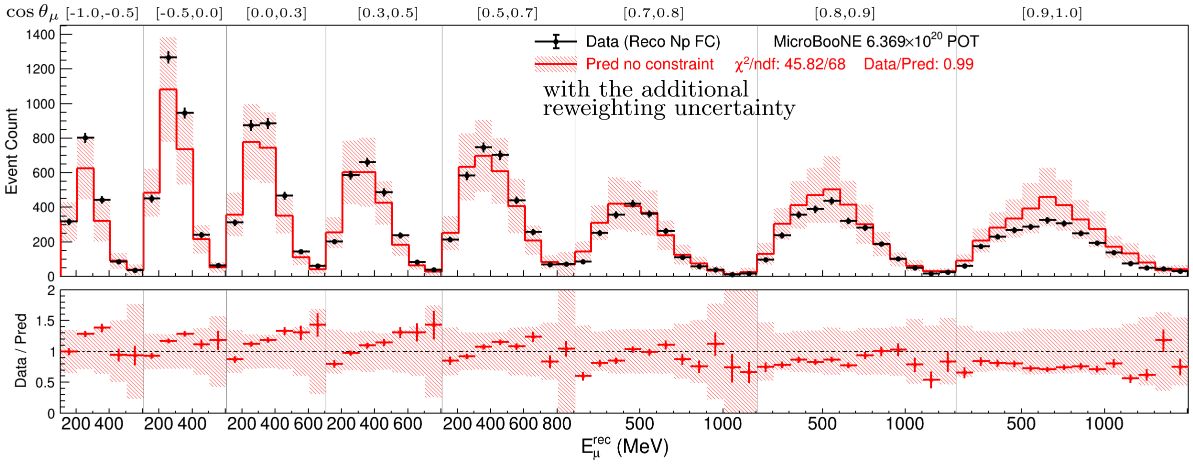


(b) Reconstructed Np FC muon energy distribution sliced in the muon angle.

FIG. 20: Comparison between data and prediction with the additional systematic derived from the reweighting as a function of muon energy in muon angle slices for FC events. The angular slices are divided by the gray lines and go from backwards on the left to forwards on the right with the last bin in each slice corresponding to overflow. The statistical and systematic uncertainties (including the additional reweighting uncertainty) of the Monte Carlo are shown in the bands. The data statistical errors are shown on the data points.

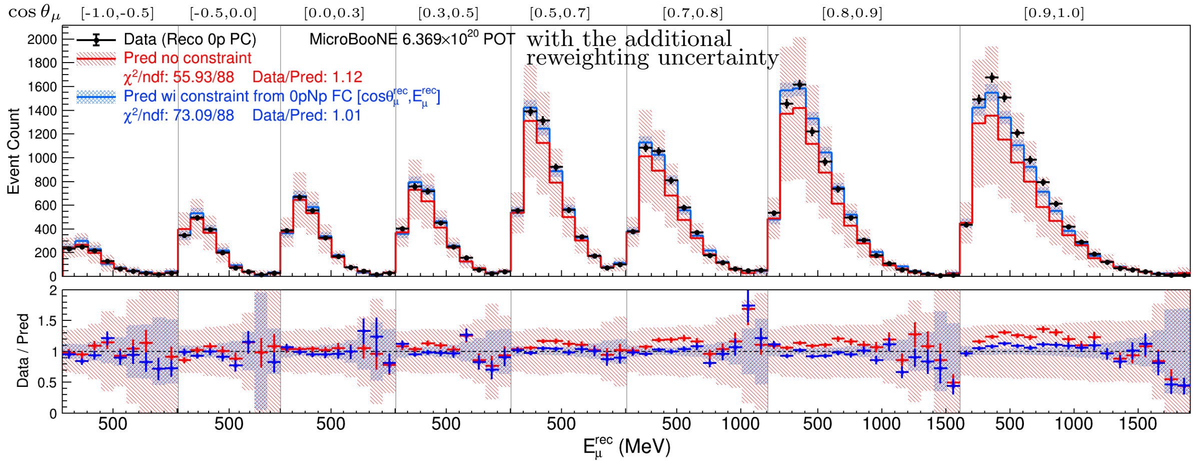


(a) Reconstructed 0p PC muon energy distribution sliced in the muon angle.

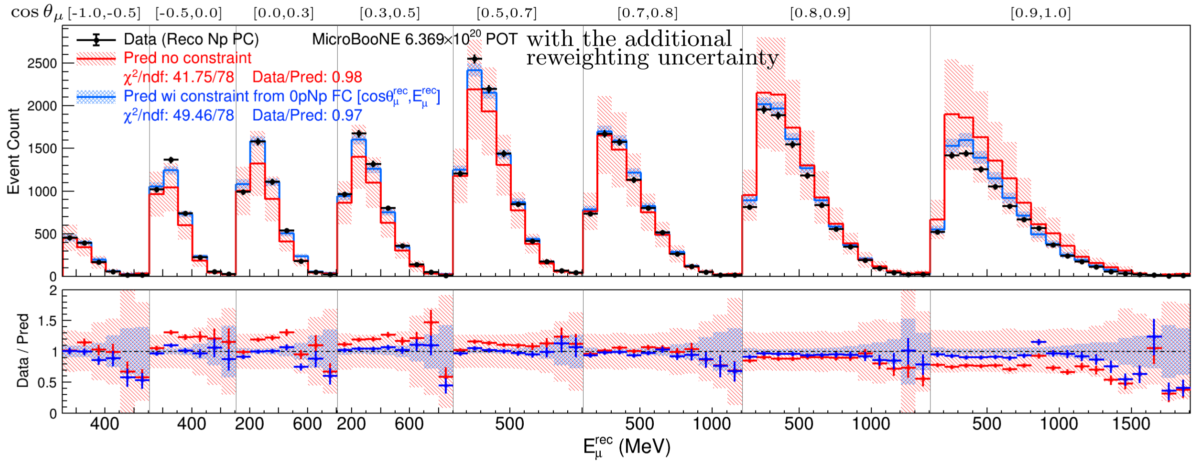


(b) Reconstructed Np PC muon energy distribution sliced in the muon angle.

FIG. 21: Comparison between data and prediction with the additional systematic derived from the reweighting as a function of muon energy in muon angle slices for PC events. The angular slices are divided by the gray lines and go from backwards on the left to forwards on the right with the last bin in each slice corresponding to overflow. The red (blue) lines and bands show the prediction without (with) the constraint from the reconstructed 0pNp FC $\{\cos\theta_\mu^{rec}, E_\mu^{rec}\}$ distribution. The statistical and systematic uncertainties (including the additional reweighting uncertainty) of the Monte Carlo are shown in the bands. The data statistical errors are shown on the data points.

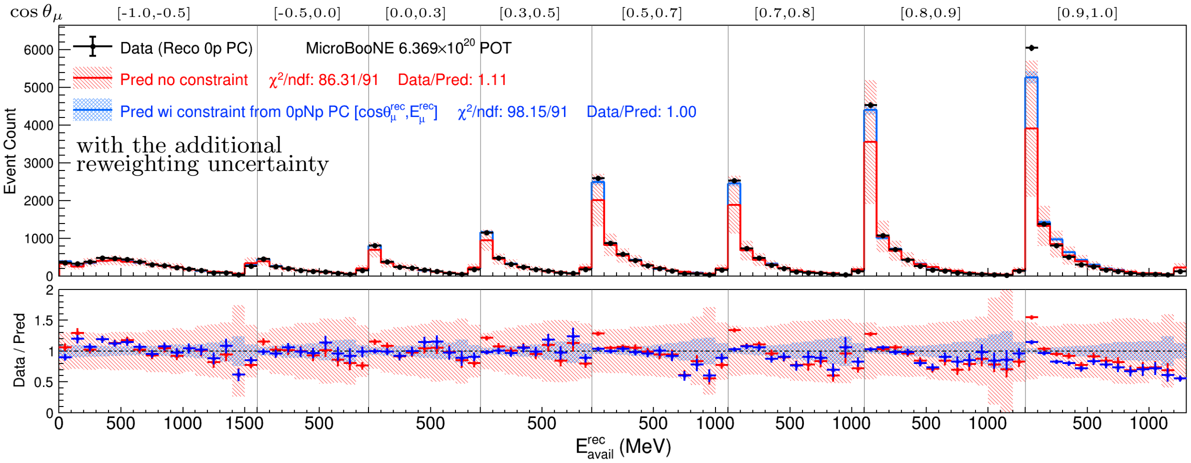


(a) Reconstructed 0p PC available energy distribution sliced in the muon angle.

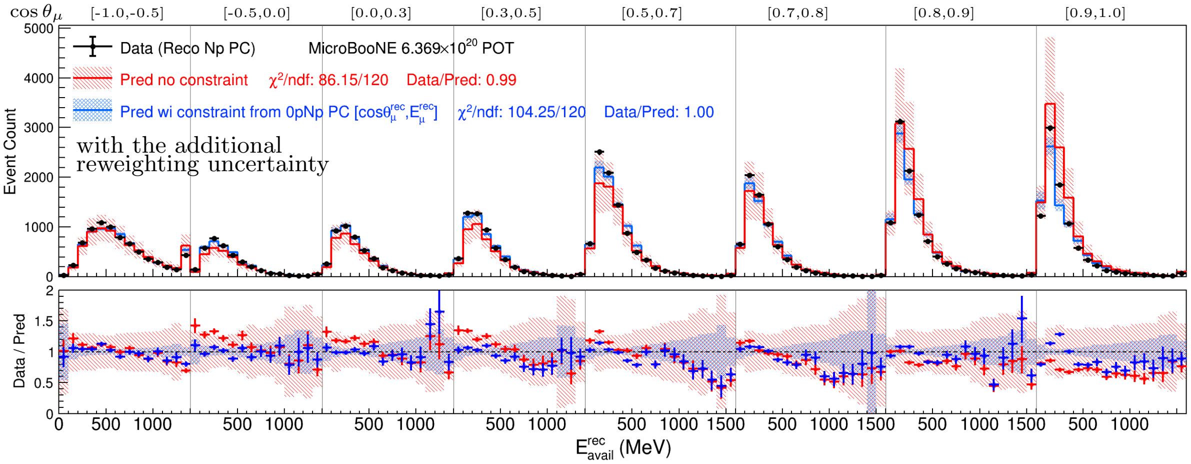


(b) Reconstructed Np PC available energy distribution sliced in the muon angle.

FIG. 22: Comparison between data and prediction with the additional systematic derived from the reweighting as a function of the reconstructed available energy in angular slices for PC events. The angular slices are divided by the gray lines and go from backwards on the left to forwards on the right with the last bin in each slice corresponding to overflow. The 0p selection is shown in (a) and the Np selection is shown in (b). The red (blue) lines and bands show the prediction without (with) the constraint from the reconstructed 0pNp PC $\{\cos\theta_\mu^{rec}, E_\mu^{rec}\}$ distribution. The statistical and systematic uncertainties (including the additional reweighting uncertainty) of the Monte Carlo are shown in the bands. The data statistical errors are shown on the data points.

## V. RECONSTRUCTED DISTRIBUTIONS WITH REWEIGHTED CENTRAL VALUES

In Sec. VII of the main text, an additional data-driven reweighing uncertainty is derived to cover data to MC discrepancies seen in the $E_{had}^{reco}$, $E_{avail}^{rec}$ and $K_p^{rec}$ distributions after constraint from the muon kinematics. The reweighting uncertainty is obtained from a reweighting function in true $K_p$ and can be seen in Fig. 23. For cross section extraction, this reweighting function is not applied to the MC prediction. Nevertheless, it is useful to examine the effect that reweighting the CV has on the data to MC agreement in the distributions the reweighing function was intended to impact. This serves as a sort of "validation of the reweighting function" and demonstrates that it is behaving as expected. As seen in the following plots, the reweighting function significantly improves the data-MC agreement on the previously problematic distributions, particularly for FC $K_p^{rec}$ from which the reweighting function was derived. This suggests the reweighting is behaving as intended.

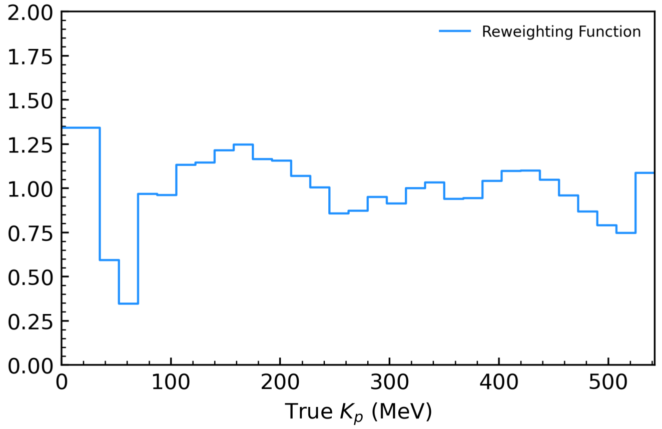


FIG. 23: The $K_p$ reweighting function derived from the discrepancy between the data and monte-carlo $K_p^{rec}$ distributions via unfolding. The first bin corresponds to true 0p events where a proton is not present or falls below the 35 MeV threshold. The last bin is overflow.

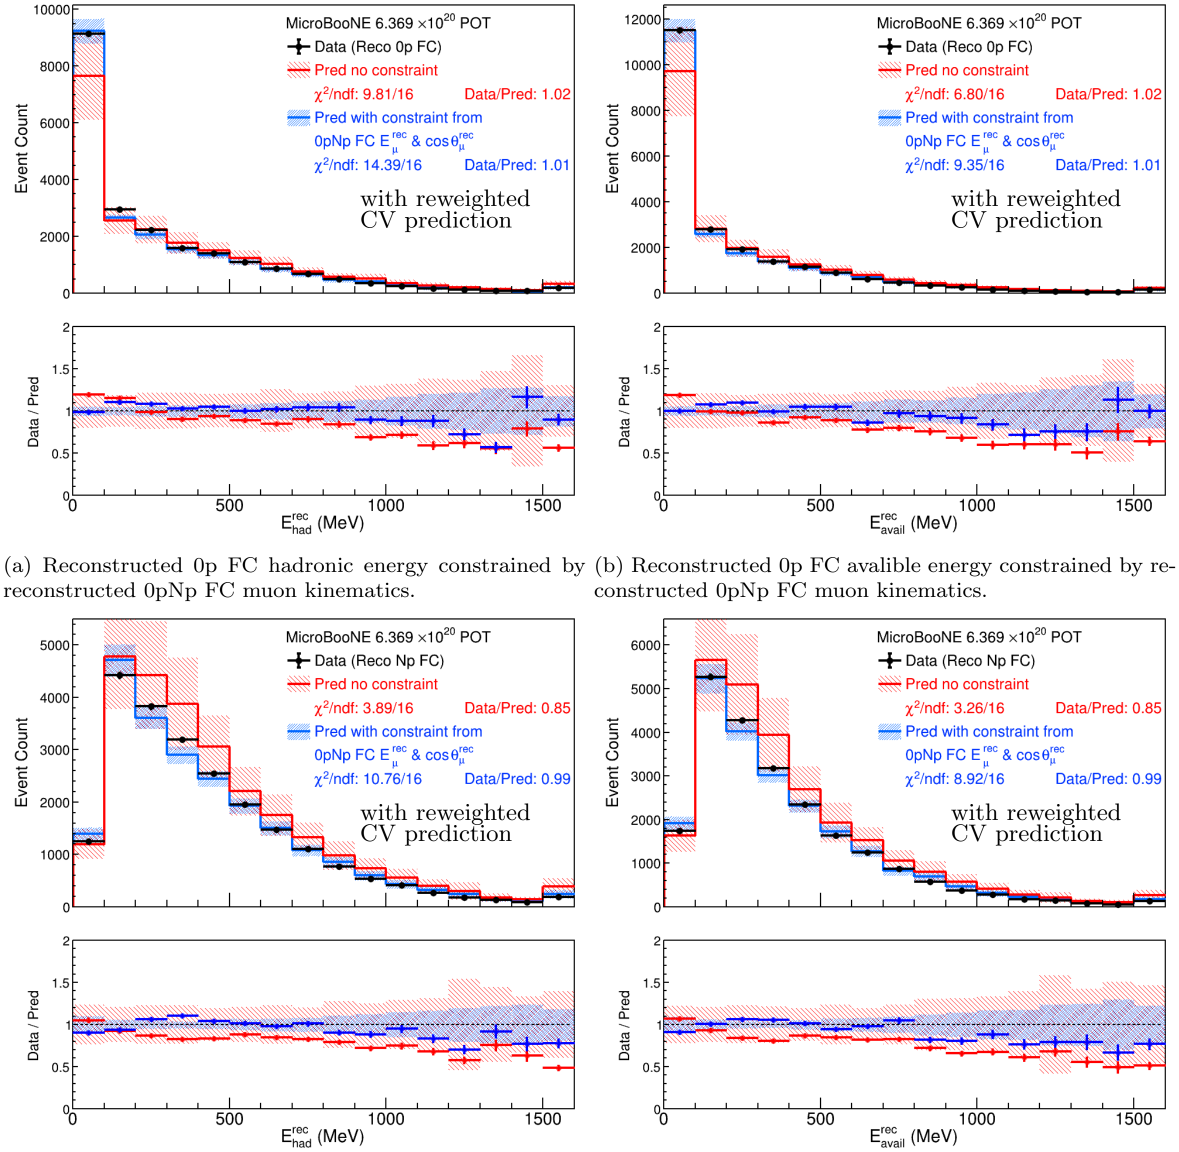


(a) Reconstructed 0p FC hadronic energy constrained by reconstructed 0pNp FC muon kinematics.

(b) Reconstructed 0p FC avalible energy constrained by reconstructed 0pNp FC muon kinematics.

(c) Reconstructed Np FC hadronic energy constrained by reconstructed 0pNp FC muon kinematics.

(d) Reconstructed Np FC available energy constrained by reconstructed 0pNp FC muon kinematics.

FIG. 24: Comparison between data and reweighted prediction as a function of the [(a) and (c)] reconstructed hadronic energy and [(b) and (d)] reconstructed available energy for FC events. In all plots, the last bin corresponds to overflow. The red (blue) lines and bands show the prediction without (with) the constraint from the reconstructed 0pNp FC muon energy and muon angle distributions. The statistical and systematic uncertainties of the Monte Carlo are shown in the bands. The data statistical errors are shown on the data points and are often too small to be seen.

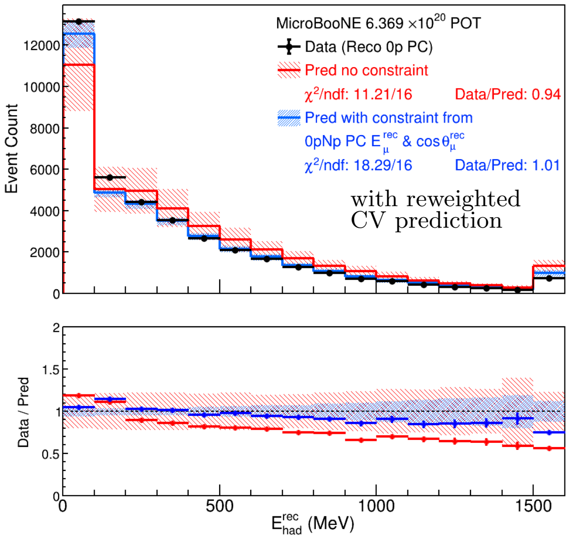


(a) Reconstructed 0p PC hadronic energy constrained by reconstructed 0pNp PC muon kinematics.

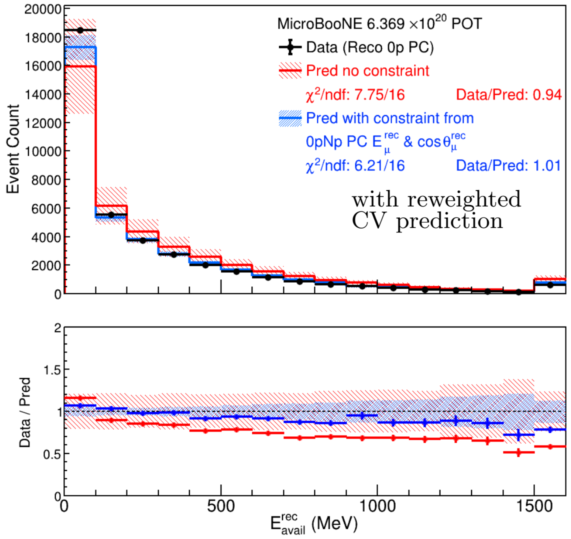


(b) Reconstructed 0p PC available energy constrained by reconstructed 0pNp PC muon kinematics.

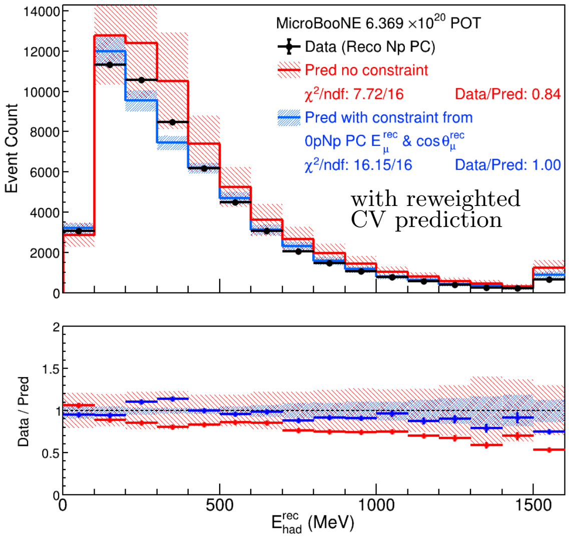


(c) Reconstructed Np PC hadronic energy constrained by reconstructed 0pNp PC muon kinematics.

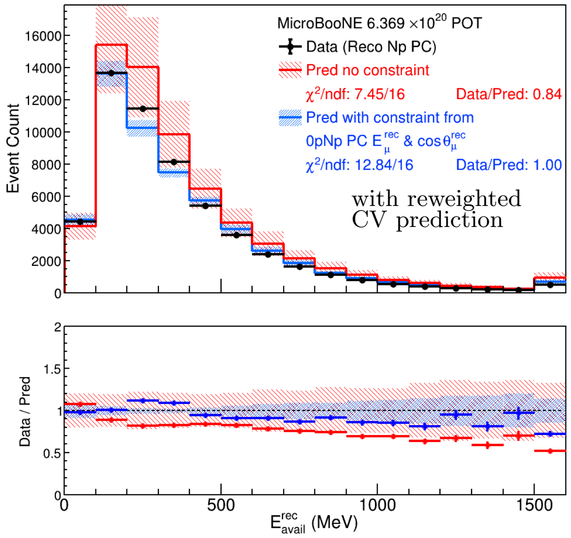


(d) Reconstructed Np PC available energy constrained by reconstructed 0pNp PC muon kinematics.

FIG. 25: Comparison between data and reweighted prediction as a function of the [(a) and (c)] reconstructed hadronic energy and [(b) and (d)] reconstructed available energy for PC events. The reconstructed 0p selections are seen in (a) and (b) and the reconstructed Np samples are seen in (c) and (d). In all plots, the last bin corresponds to overflow. The red (blue) lines and bands show the prediction without (with) the constraint from the reconstructed 0pNp PC muon energy and muon angle distributions. The statistical and systematic uncertainties of the Monte Carlo are shown in the bands. The data statistical errors are shown on the data points and are often too small to be seen.

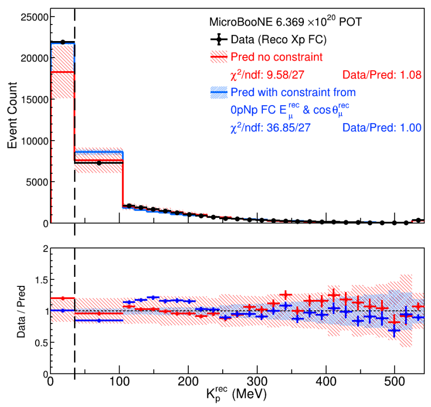


(a) Leading proton kinetic energy for FC events constrained by the 0pNp FC muon kinematics.

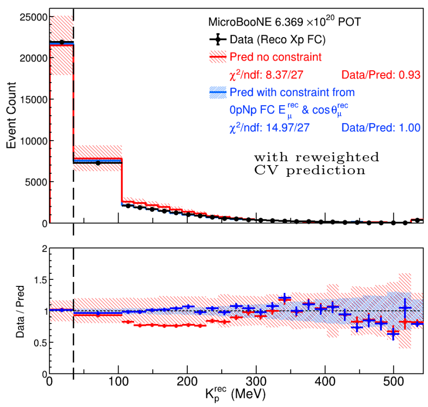


(b) Leading proton kinetic energy for FC events constrained by the 0pNp FC muon kinematics. The MC prediction has been reweighted.

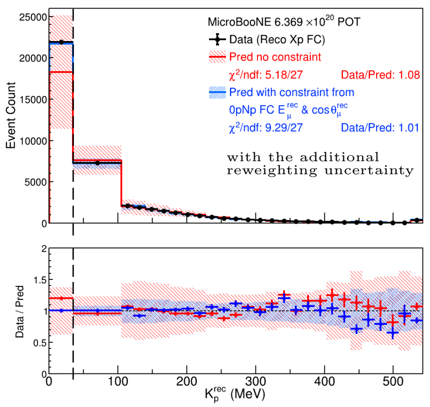


(c) Leading proton kinetic energy for FC events constrained by the 0pNp FC muon kinematics. The reweighting systematic has been added to the MC prediction.

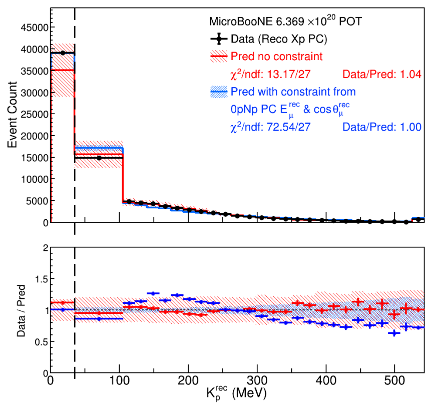


(d) Leading proton kinetic energy for PC events constrained by the 0pNp PC muon kinematics.

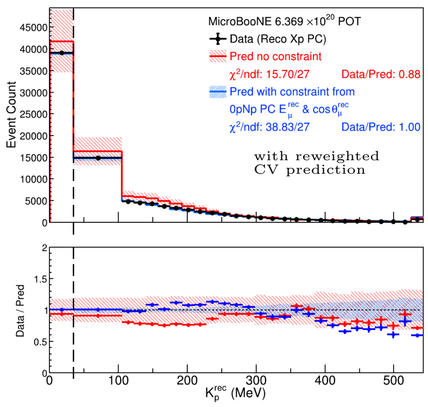


(e) Leading proton kinetic energy for PC events constrained by the 0pNp PC muon kinematics. The MC prediction has been reweighted.

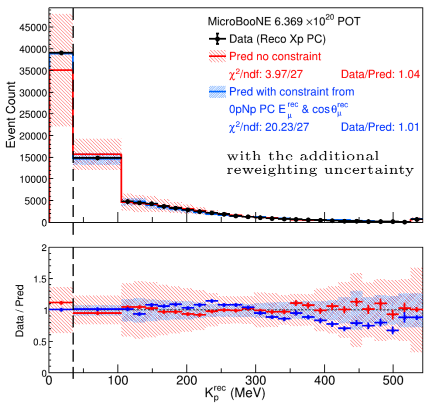


(f) Leading proton kinetic energy for PC events constrained by the 0pNp PC muon kinematics. The reweighting systematic has been added to the MC prediction.

FIG. 26: Comparison between data and MC prediction as a function of the reconstructed leading proton kinetic energy for [(a), (b) and (c)] FC events and [(d), (e) and (f)] PC events. The binning is the same as for $M$ in the cross section extraction. The nominal MC prediction is shown in (a) and (d), the reweighted MC prediction is shown in (b) and (e), and the nominal MC prediction with the additional reweighting uncertainty is shown in is shown in (c) and (f). The dashed line in indicates the 35 MeV proton tracking threshold, below which is a single bin that includes events with no protons and events where the leading proton is below the threshold. In all plots, the last bin corresponds to overflow. The red (blue) lines and bands show the prediction without (with) the constraint from the muon kinematics. The statistical and systematic uncertainties of the Monte Carlo are shown in the bands. The data statistical errors are shown on the data points.

## VI. UNCERTAINTIES ON UNFOLDED RESULTS

What follows is the contribution of uncertainties by systematic type for each cross section extracted in Sec. VIII of the main text. The corresponding correlation matrices are also shown. These plots are a function of the bin index and all bins are all equal width; bins do not correspond to their physical width. More information on the binning can be found in Sec. VIII. The regularized truth space covariance matrix containing these uncertainties is obtained from the reconstructed space covariance matrix through the Wiener-SVD unfolding via Eq. (12) of the main text.

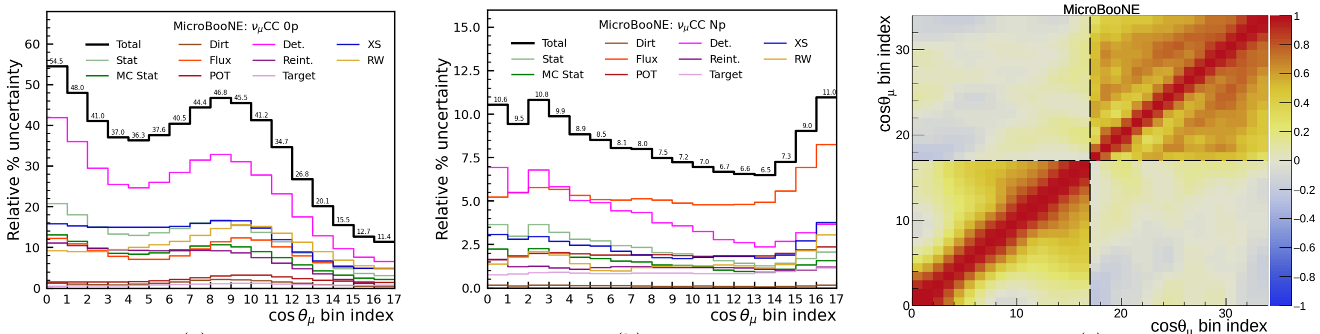


(a) (b) (c)

FIG. 27: [(a) and (b)] Contribution of uncertainties by systematic type for the extraction of the (a) 0p and (b) Np cross section as a function of $\cos\theta_\mu$. (c) The correlation matrix obtained from the extraction of the 0pNp cross section as a function of $\cos\theta_\mu$. The dashed lines separate the 0p and Np channels. On all plots, the true bins are those found in Sec. VIII and are the same as those on the extracted cross section. The entries shown in (a) and (b) correspond to the square root of the diagonal elements of the covariance matrix obtained from unfolding divided by the value of the extracted cross section for the given bin.

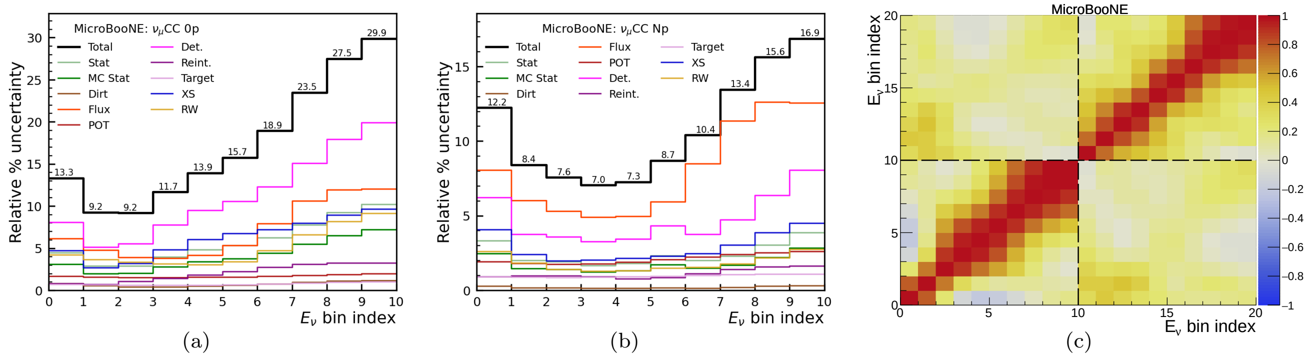


(a) (b) (c)

FIG. 28: [(a) and (b)] Contribution of uncertainties by systematic type for the extraction of the (a) 0p and (b) Np cross section as a function of $E_\nu$. (c) The correlation matrix obtained from the extraction of the 0pNp cross section as a function of $E_\nu$. The dashed lines separate the 0p and Np channels. On all plots, the true bins are those found in Sec. VIII and are the same as those on the extracted cross section. The entries shown in (a) and (b) correspond to the square root of the diagonal elements of the covariance matrix obtained from unfolding divided by the value of the extracted cross section for the given bin.

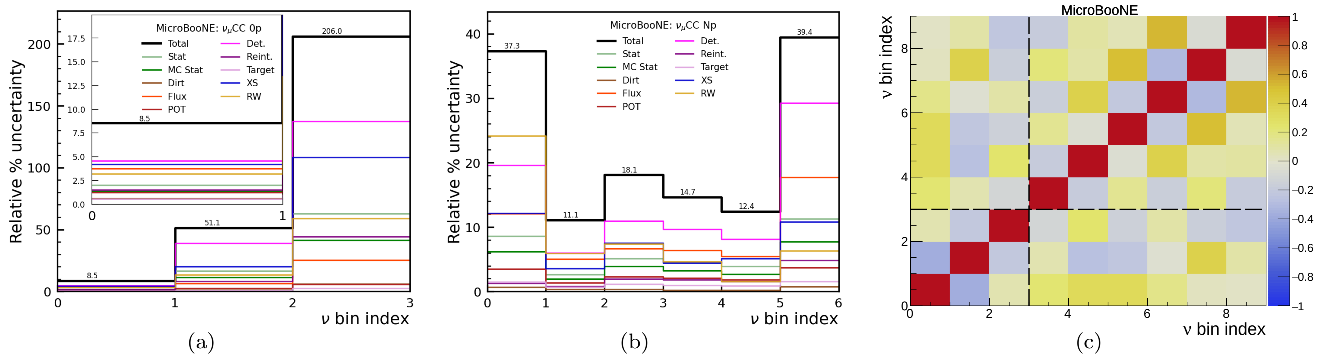


FIG. 29: [(a) and (b)] Contribution of uncertainties by systematic type for the extraction of the (a) 0p and (b) Np $\nu$ differential cross section. (c) The correlation matrix obtained from the extraction of the 0pNp $\nu$ differential cross section. The dashed lines separate the 0p and Np channels. On all plots, the true bins are those found in Sec. VIII and are the same as those on the extracted cross section. The entries shown in (a) and (b) correspond to the square root of the diagonal elements of the covariance matrix obtained from unfolding divided by the value of the extracted cross section for the given bin.

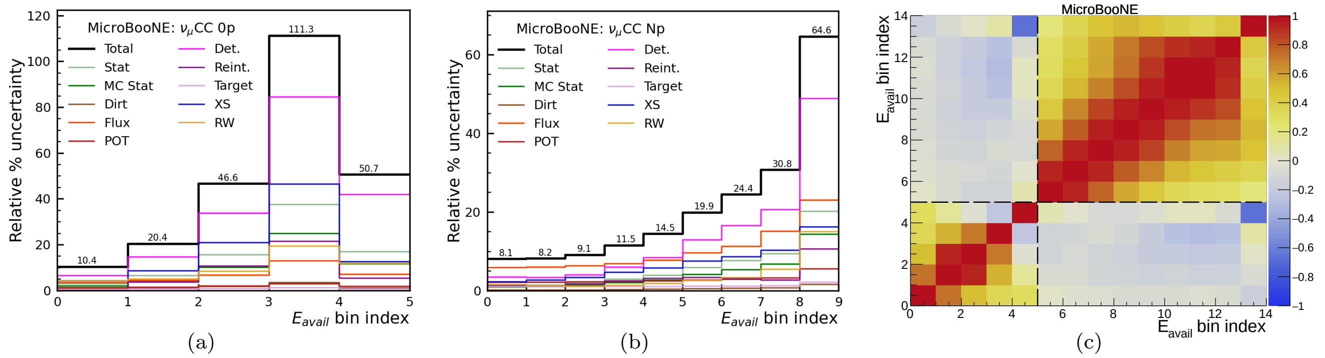


FIG. 30: [(a) and (b)] Contribution of uncertainties by systematic type for the extraction of the (a) 0p and (b) Np $E_{avail}$ differential cross section. (c) The correlation matrix obtained from the extraction of the 0pNp $E_{avail}$ differential cross section. The dashed lines separate the 0p and Np channels. On all plots, the true bins are those found in Sec. VIII and are the same as those on the extracted cross section. The entries shown in (a) and (b) correspond to the square root of the diagonal elements of the covariance matrix obtained from unfolding divided by the value of the extracted cross section for the given bin.

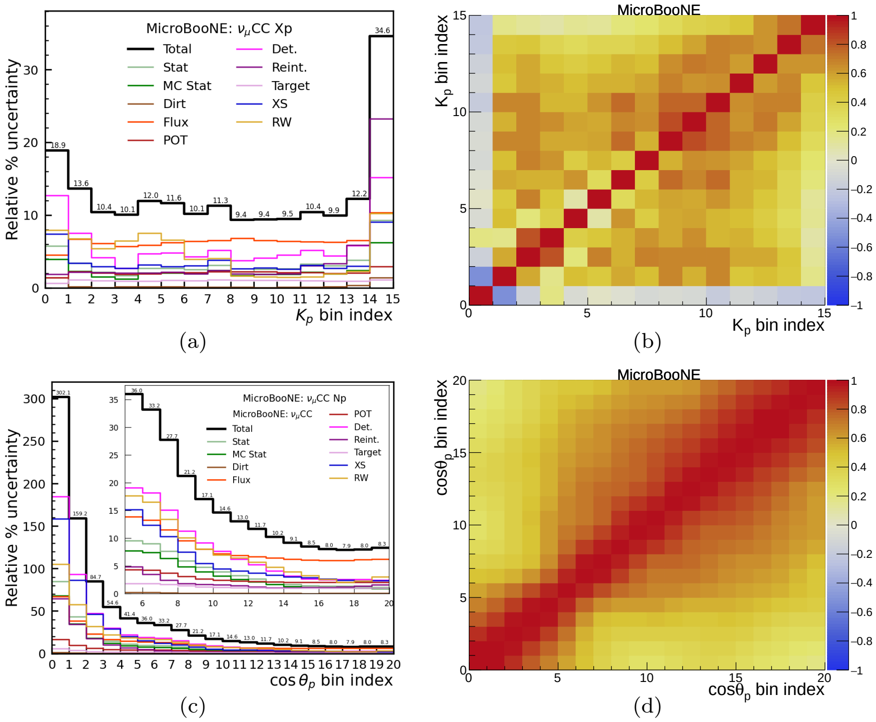


FIG. 31: [(a) and (c)] Contribution of uncertainties by systematic type for the extraction of (a) the $K_p$ differential cross section and (c) the $\cos\theta_p$ differential cross section. [(b) and (d)] The correlation matrix obtained from the extraction of the (b) $K_p$ differential cross section and (d) the $\cos\theta_p$ differential cross section. On all plots, the true bins are those found in Sec. VIII and are the same as those on the extracted cross section. The entries shown in (a) and (c) correspond to the square root of the diagonal elements of the corresponding covariance matrix obtained from the unfolding divided by the value of the extracted cross section for the given bin.

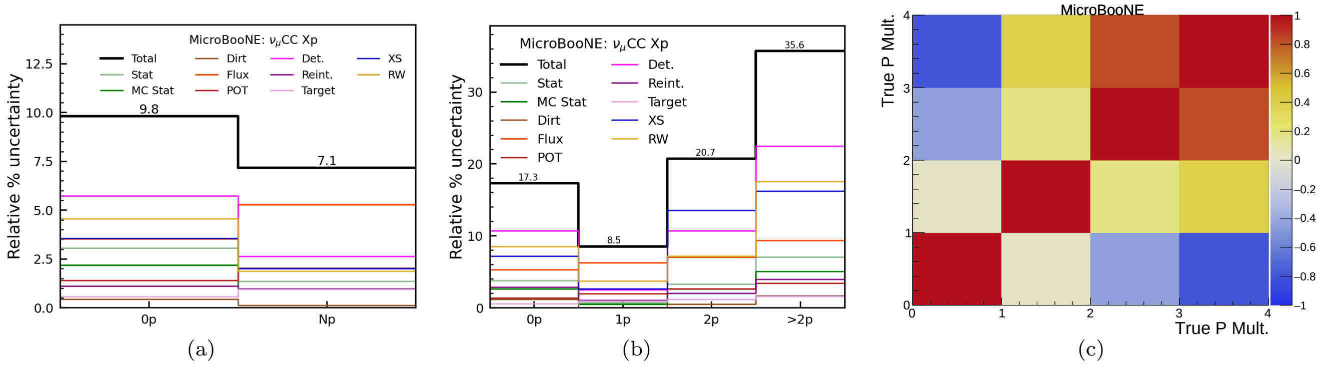


FIG. 32: [(a) and (b)] Contribution of uncertainties by systematic type for the extraction of the (a) the total 0p and Np cross sections and (b) cross section as a function of the proton multiplicity. (c) The correlation matrix obtained from the extraction of the cross section as a function of the proton multiplicity. On all plots, the true bins are those found in Sec. VIII and are the same as those on the extracted cross section. The entries shown in (b) correspond to the square root of the diagonal elements of the covariance matrix obtained from unfolding divided by the value of the extracted cross section for the given bin.

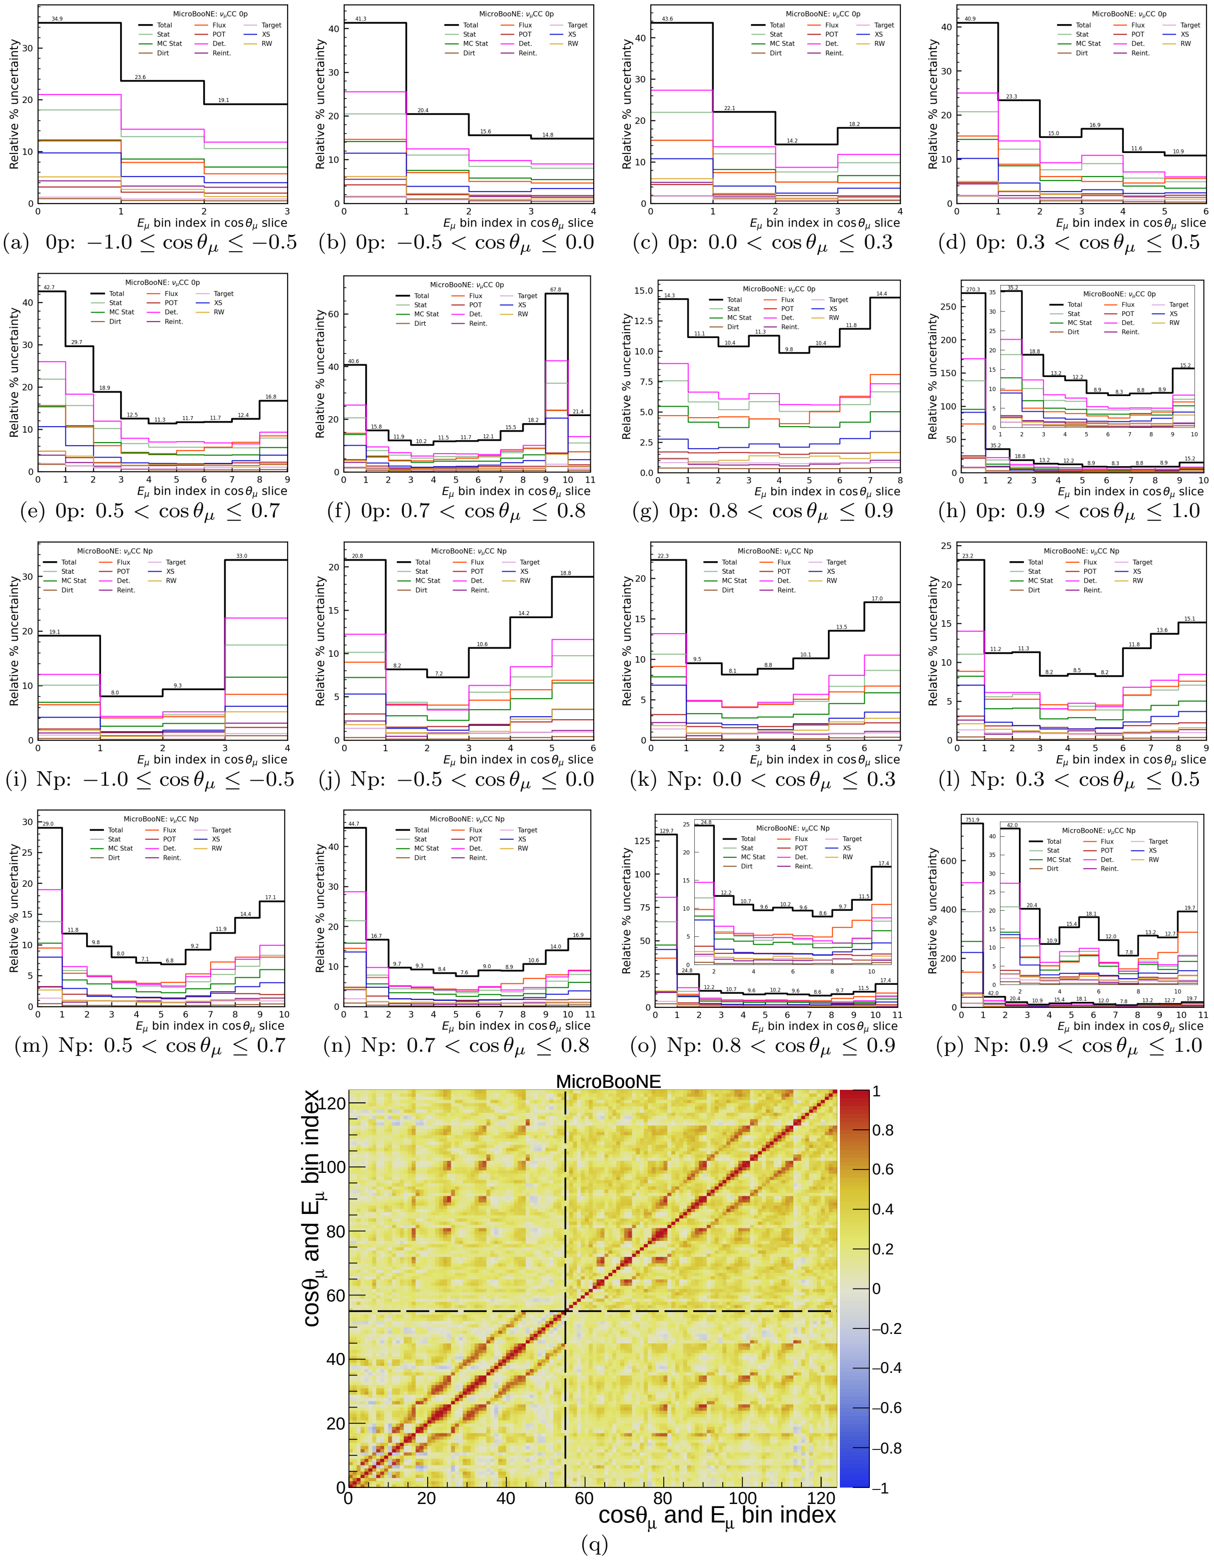


(a) 0p: $-1.0 \le \cos\theta_\mu \le -0.5$ (b) 0p: $-0.5 < \cos\theta_\mu \le 0.0$ (c) 0p: $0.0 < \cos\theta_\mu \le 0.3$ (d) 0p: $0.3 < \cos\theta_\mu \le 0.5$

(e) 0p: $0.5 < \cos\theta_\mu \le 0.7$ (f) 0p: $0.7 < \cos\theta_\mu \le 0.8$ (g) 0p: $0.8 < \cos\theta_\mu \le 0.9$ (h) 0p: $0.9 < \cos\theta_\mu \le 1.0$

(i) Np: $-1.0 \le \cos\theta_\mu \le -0.5$ (j) Np: $-0.5 < \cos\theta_\mu \le 0.0$ (k) Np: $0.0 < \cos\theta_\mu \le 0.3$ (l) Np: $0.3 < \cos\theta_\mu \le 0.5$

(m) Np: $0.5 < \cos\theta_\mu \le 0.7$ (n) Np: $0.7 < \cos\theta_\mu \le 0.8$ (o) Np: $0.8 < \cos\theta_\mu \le 0.9$ (p) Np: $0.9 < \cos\theta_\mu \le 1.0$

(q)

FIG. 33: [(a)-(p)] Contribution of uncertainties by systematic type for the extraction of the double differential $\cos\theta_\mu$ and $E_\mu$ cross section result. Each plot shows a different angular slice. (q) The correlation matrix obtained from the extraction of the double differential 0pNp $\cos\theta_\mu$ and $E_\mu$ cross section result. The dashed lines separate the 0p and Np channels. On all plots, the true bins are those found in Sec. VIII and are the same as those on the extracted cross section. The entries shown here correspond to the square root of the diagonal elements of covariance matrix obtained from unfolding divided by the value of the extracted cross section for the given bin. The POT (Target) uncertainty is not identically 2% (1%) in all bins due to smearing in the unfolding; this smearing is captured in $A_C$.

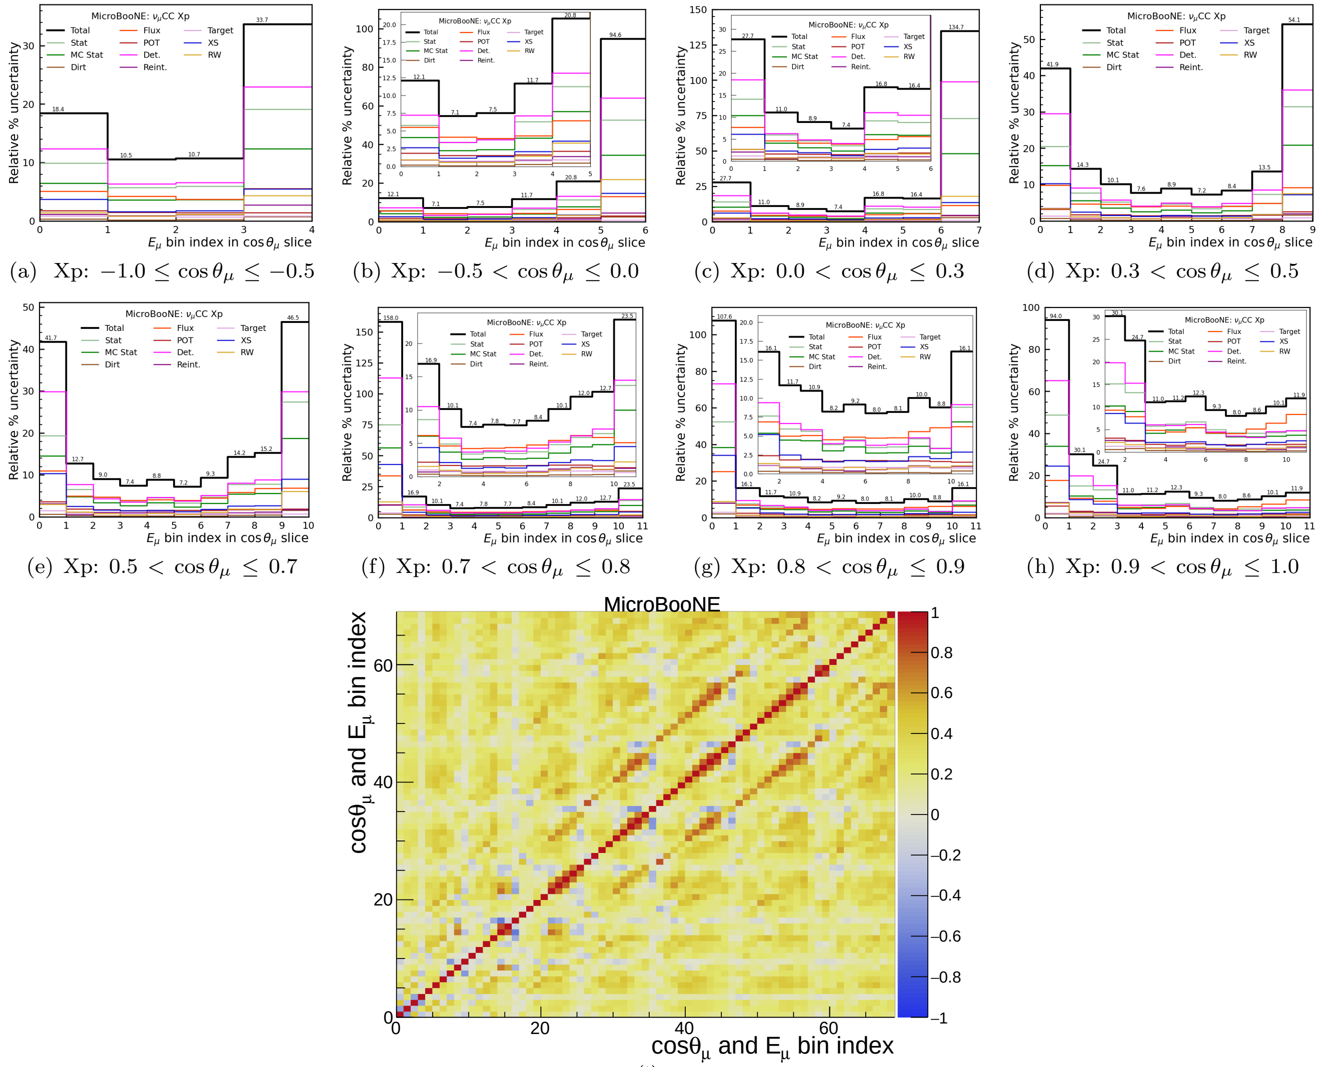


(a) Xp: $-1.0 \leq \cos\theta_\mu \leq -0.5$ (b) Xp: $-0.5 < \cos\theta_\mu \leq 0.0$ (c) Xp: $0.0 < \cos\theta_\mu \leq 0.3$ (d) Xp: $0.3 < \cos\theta_\mu \leq 0.5$

(e) Xp: $0.5 < \cos\theta_\mu \leq 0.7$ (f) Xp: $0.7 < \cos\theta_\mu \leq 0.8$ (g) Xp: $0.8 < \cos\theta_\mu \leq 0.9$ (h) Xp: $0.9 < \cos\theta_\mu \leq 1.0$

(i)

FIG. 34: [(a)-(h)] Contribution of uncertainties by systematic type for the extraction of the double-differential Xp $\cos\theta_\mu$ and $E_\mu$ cross section result. Each plots shows a different angular slice. (i) The correlation matrix obtained from the extraction of the double differential Xp $\cos\theta_\mu$ and $E_\mu$ cross section result. On all plots, the true bins are those found in Sec. VIII and are the same as those on the extracted cross section. The entries shown in (a)-(h) correspond to the square root of the diagonal elements of the covariance matrix obtained from unfolding divided by the value of the extracted cross section for the given bin.

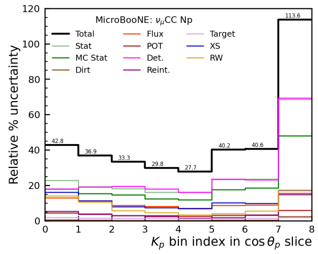


(a) $-1.0 \leq \cos\theta_p \leq -0.5$

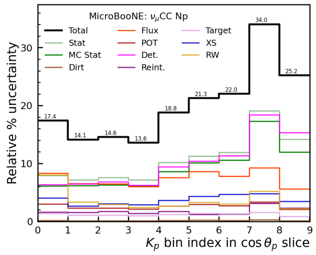


(b) $-0.5 < \cos\theta_p \leq 0.0$

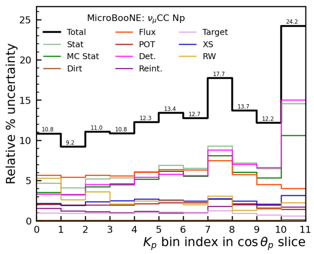


(c) $0.0 < \cos\theta_p \leq 0.3$

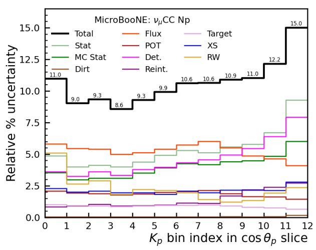


(d) $0.3 < \cos\theta_p \leq 0.5$

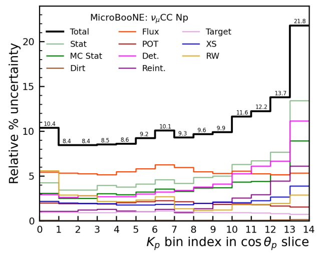


(e) $0.5 < \cos\theta_p \leq 0.7$

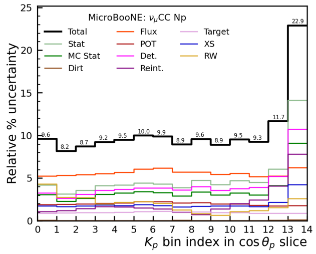


(f) $0.7 < \cos\theta_p \leq 0.8$

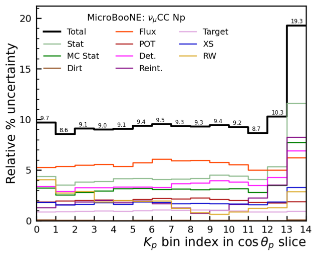


(g) $0.8 < \cos\theta_p \leq 0.9$

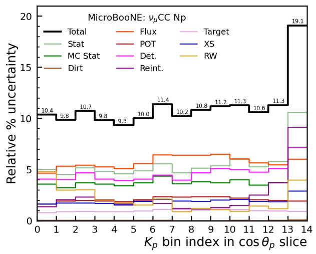


(h) $0.9 < \cos\theta_p \leq 1.0$

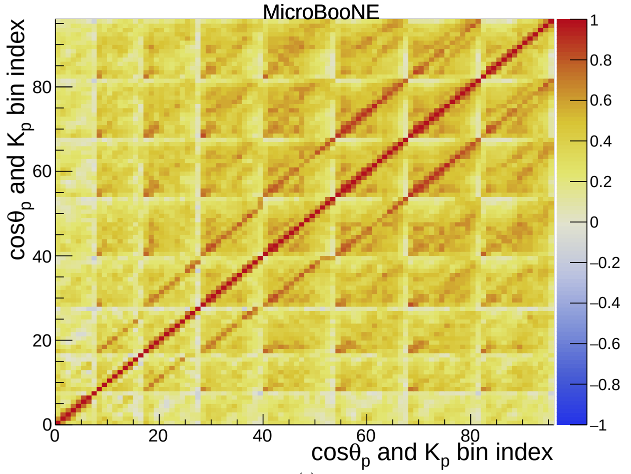


(i)

FIG. 35: [(a)-(h)] Contribution of uncertainties by systematic type for the extraction of the double differential $\cos\theta_p$ and $K_p$ cross section result. Each plot shows a different angular slice. (i) The correlation matrix obtained from the extraction of the double differential $\cos\theta_p$ and $K_p$ cross section result. On all plots, the true bins are those found in Sec. VIII and are the same as those on the extracted cross section. The entries shown in (a)-(h) correspond to the square root of the diagonal elements of the covariance matrix obtained from unfolding divided by the value of the extracted cross section for the given bin.

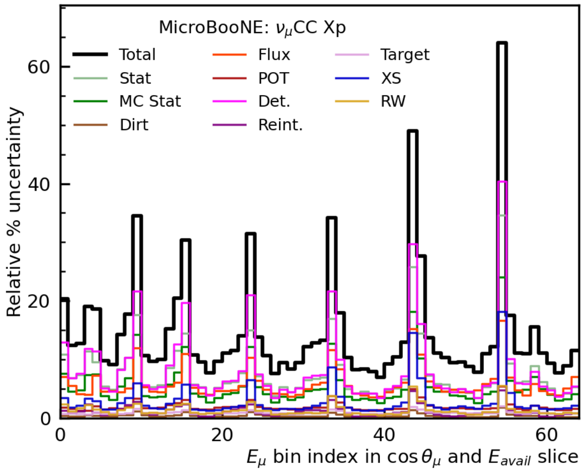


(a) Xp: $0 \leq E_{avail} \leq 0.3$

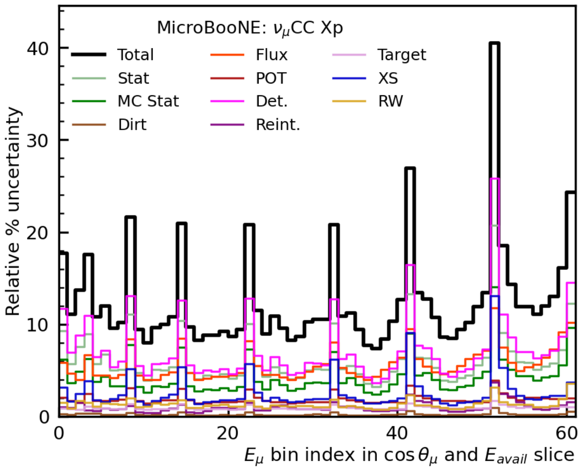


(b) Xp: $0.3 < E_{avail} \leq 0.45$

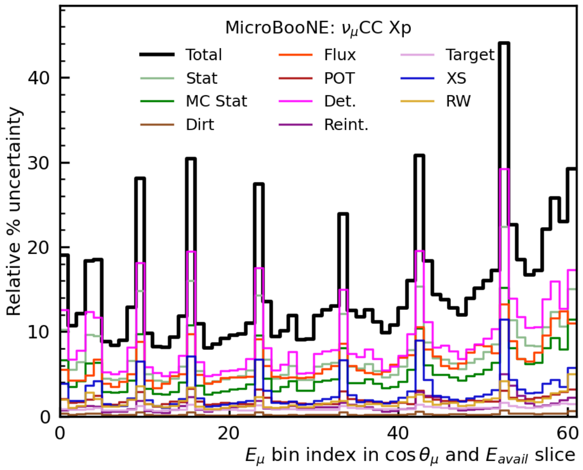


(c) Xp: $0.45 < E_{avail} \leq 0.65$

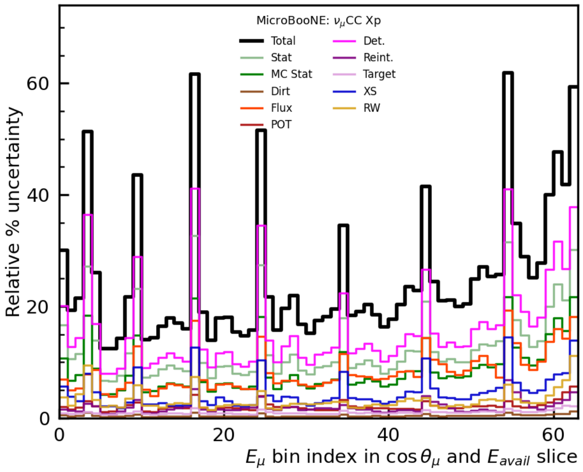


(d) Xp: $0.65 < E_{avail} \leq 2.5$

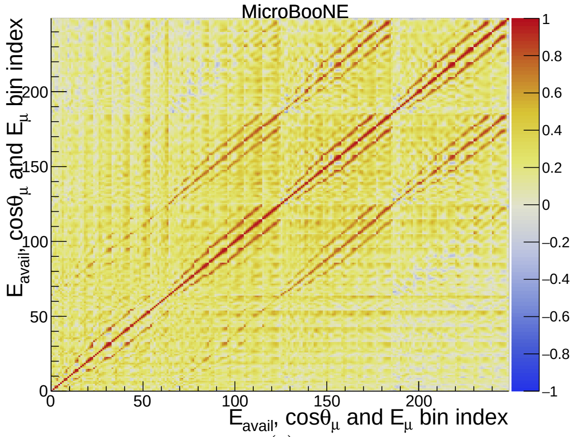


(e)

FIG. 36: [(a)-(d)] [(a) and (b)] Contribution of uncertainties by systematic type for the extraction of the triple differential Xp $E_{avail}$ $\cos\theta_\mu$ and $E_\mu$ cross section result. Each plot shows a different $E_{avail}$ slice, each with a complete set of angular slices. (e) The correlation matrix obtained from the extraction of the triple differential Xp $E_{avail}$, $\cos\theta_\mu$ and $E_\mu$ cross section result. On all plots, the true bins are those found in Sec. VIII and are the same as those on the extracted cross section. The entries shown in (a)-(d) correspond to the square root of the diagonal elements of the covariance matrix obtained from unfolding divided by the value of the extracted cross section for the given bin.

## VII. BLOCKWISE COVARIANCE MATRIX

Cross sections in different variables from the same data set are typically treated as if they are independent experiments reducing the power of the full multivariable result [3]. To overcome this limitation, a blockwise covariance matrix that contains inter-variable correlations between all cross section measurements is presented in Fig. 37 and in the data release. This covariance matrix was obtained following the procedure described in Sec. III B of the main text and at length in [4]. The $\chi^2$ values calculated with this covariance matrix properly account for inter-variable correlations across bins in different measurements thereby allowing multiple measurements to be examined simultaneously. To further articulate the points described Sec. VIII of the main text, a variety of these $\chi^2$ values for different combinations of variables and channels can be found in Table IV. These inter-variable $\chi^2$ values support the notion that `GiBUU` best describes the 0p data and that `NEUT` best describe the Np muon kinematics. Likewise, these $\chi^2$ values indicate that the $\mu$`BooNE` tune performs the best on the Np and 0pNp energy related variables, though `NuWro` is quite comparable despite its worse performance on individual measurements. `NuWro` also offers the best performance on the proton related variables, especially when the 0p bins are excluded. Despite the `NEUT` prediction's overall good performance on the Np muon kinematics, its $\chi^2$ value calculated on the proton related variables is the worst of the five generators. Across all single-differential Np bins, the $\chi^2$ value for the $\mu$`BooNE` tune, `GENIE` and `NuWro` are comparable. A similar hierarchy is also seen for the $\chi^2$ obtained using all 0pNp bins, thought `NEUT` does noticeably worse than the others here, presumably due to its inability to describe the 0p data.

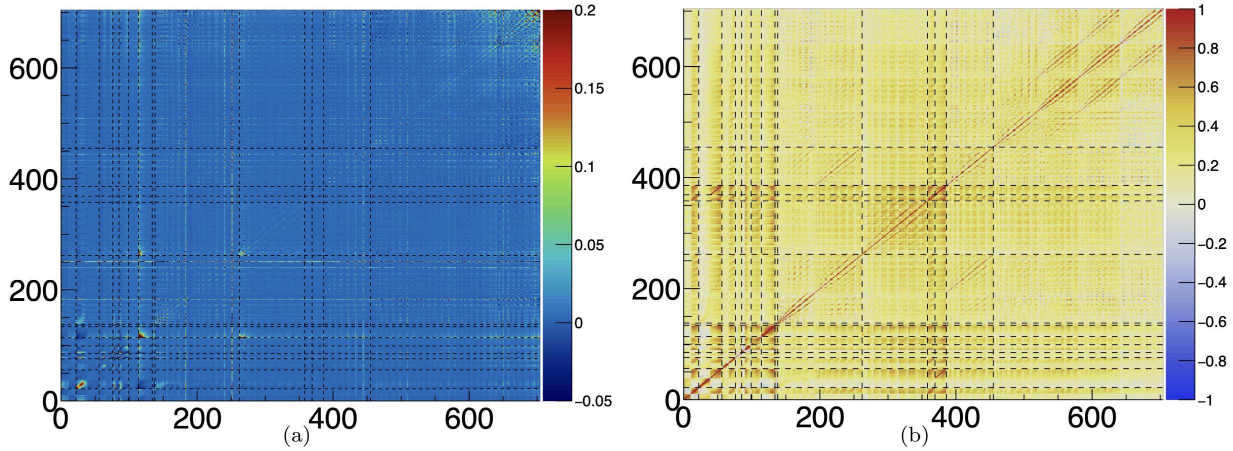


FIG. 37: The blockwise (a) fractional covariance and (b) correlation matrix obtained utilising the blockwise unfolding procedure described in Sec. III B. The dashed lines separate different measurements which are ordered as follows: 0pNp $E_\mu$, 0pNp $\cos\theta_\mu$, 0pNp $E_\nu$, 0pNp $\nu$, 0pNp $E_{avail}$, $K_p$, $\cos\theta_p$, proton multiplicity, 2D 0pNp $\{\cos\theta_\mu, E_\mu\}$, 2D $\{\cos\theta_p, K_p\}$, Xp $E_\mu$, Xp $\cos\theta_\mu$, 2D Xp $\{\cos\theta_\mu, E_\mu\}$, 3D Xp $\{E_{avail}, \cos\theta_\mu, E_\mu\}$. Each axis corresponds to the bin index and does not represent the physical width of the bin. More information on the binning is found in Sec. VIII.

| Measurements | Channel | *ndf* | $\mu$`BooNE` | `GENIE` | `NuWro` | `NEUT` | `GiBUU` |
|---|---|---|---|---|---|---|---|
| $E_\mu$,$\cos\theta_\mu$, $E_\nu$, $\nu$, $E_{avail}$ | 0p | 46 | 89.3 | 99.8 | 71.0 | 159.9 | 57.6 |
| $E_\mu$,$\cos\theta_\mu$, $E_\nu$, $\nu$, $E_{avail}$, $K_p$, $\cos\theta_p$, P Mult. (no 0p) | Np | 90 | 123.6 | 124.0 | 127.3 | 150.4 | 147.8 |
| $E_\mu$,$\cos\theta_\mu$, $E_\nu$, $\nu$, $E_{avail}$, $K_p$, $\cos\theta_p$, P Mult. | 0pNp | 138 | 246.1 | 255.6 | 229.4 | 444.1 | 321.7 |
| $E_\nu$, $\nu$, $E_{avail}$ | 0p | 18 | 47.1 | 57.3 | 40.4 | 108.9 | 30.0 |
| | Np | 25 | 30.5 | 43.6 | 34.7 | 50.4 | 43.2 |
| | 0pNp | 43 | 86.8 | 95.7 | 74.7 | 206.6 | 119.6 |
| $E_\mu$,$\cos\theta_\mu$ | 0p | 28 | 50.8 | 54.1 | 37.1 | 74.3 | 27.6 |
| | Np | 28 | 53.1 | 56.6 | 58.4 | 32.4 | 51.2 |
| | 0pNp | 56 | 98.0 | 101.0 | 91.3 | 104.7 | 88.0 |
| $K_p$, $\cos\theta_p$, P Mult. | Xp | 39 | 42.8 | 44.4 | 34.9 | 70.3 | 69.5 |
| | Np | 37 | 39.6 | 42.3 | 27.1 | 67.9 | 64.2 |

TABLE IV: Comparisons between the data and generator predictions for various combinations of single-different results. When applicable, the 0p, Np, 0pNp and Xp $\chi^2$ values and respective *ndf* are shown for each set of measured variables. These $\chi^2$ values are obtained using the blockwise covariance matrix which includes the correlations between the measurements.

## VIII. DATA RELEASE

The unfolded cross section results shown in Sec. VIII of the main text can be found tabulated below. The uncertainty corresponding to the square root of the diagonal elements of the extracted covariance matrix is shown for each bin. The extracted cross section results and their covariance matrices can be found in a machine-readable form in `xs.txt` and `cov.txt`, respectively. The measurements from [1] and its Supplemental Material are also included. The additional smearing matrix, $A_C$, obtained from the Wiener-SVD unfolding can be found in the same format in `Ac.txt`. Any theory or event generator prediction should be multiplied by the additional smearing matrix when comparing to this data. These files are presented in a blockwise fashion with inter-variable correlations obtained via the blockwise unfolding procedure described in [4] and in Sec. III B of the main text. The Global Bin index listed in the following tables corresponds to the location of the bin in the blockwise covariance matrix and the Bin index corresponds to the location within the given measurement.

An example script in `gen_compare_demo.C` demonstrating how to compare the data to an external prediction is also included. This script loads the various data release files into `ROOT` `TMatrixD` and `TVectorD` objects. It then compares the data to an external prediction contained in `pred.txt` by first smearing the prediction and then calculating $\chi^2$ values for various measurements. The example external prediction included in the data release is the $\mu$`BooNE` tune MC. More information on the files and their usage can be found in `readme.txt`.

The nominal muon neutrino flux spectrum of the Fermilab Booster Neutrino Beam at the MicroBooNE detector location can be found in `numu_flux.txt`. The results in `xs.txt` are averaged over this reference flux. External cross section predictions should likewise be averaged over this flux distribution. Note that for the total cross sections reported in Fig. 25 of the main text, the results are averaged over the flux from 0.2 to 4 GeV. This yields a total integrated flux of $4.268{\times}10^{11}$ in units of number of neutrinos per cm$^2$ for an exposure of $6.369{\times}10^{20}$ protons on target. Similarly, for the results shown in Fig. 20 of the main text, each bin is averaged over the range of the flux corresponding to the given bin. All other results have the flux integral extend over the entirety of the BNB flux. This yields a total integrated flux of $4.586{\times}10^{11}$ in units of number of neutrinos per cm$^2$ for an exposure of $6.369{\times}10^{20}$ protons on target. Neutrino flux uncertainties are fully accounted for in the extracted covariance matrix and do not need to be included in theory or event generator predictions when comparing to the results. More information `numu_flux.txt` can be found in `readme.txt`.

| 0pNp $E_\mu$ differential cross section results | | | | | |
|---|---|---|---|---|---|
| Global Bin | Bin | $E_\mu$ Low (GeV) | $E_\mu$ High (GeV) | $\frac{d\sigma}{dE_\mu}$ ($\times 10^{-36} \frac{\text{cm}^2}{\text{Ar GeV}}$) | Uncertainty ($\times 10^{-36} \frac{\text{cm}^2}{\text{Ar GeV}}$) |
| 0p | | | | | |
| 0 | 0 | 0.106 | 0.226 | 0.0417 | 0.0200 |
| 1 | 1 | 0.226 | 0.296 | 0.0692 | 0.0164 |
| 2 | 2 | 0.296 | 0.386 | 0.0830 | 0.0143 |
| 3 | 3 | 0.386 | 0.505 | 0.0881 | 0.0136 |
| 4 | 4 | 0.505 | 0.577 | 0.0815 | 0.0116 |
| 5 | 5 | 0.577 | 0.659 | 0.0773 | 0.0108 |
| 6 | 6 | 0.659 | 0.753 | 0.0691 | 0.0098 |
| 7 | 7 | 0.753 | 0.861 | 0.0692 | 0.0078 |
| 8 | 8 | 0.861 | 0.984 | 0.0577 | 0.0064 |
| 9 | 9 | 0.984 | 1.285 | 0.0392 | 0.0047 |
| 10 | 10 | 1.285 | 2.506 | 0.0047 | 0.0012 |
| Np | | | | | |
| 11 | 11 | 0.106 | 0.226 | 0.1644 | 0.0251 |
| 12 | 12 | 0.226 | 0.296 | 0.3180 | 0.0260 |
| 13 | 13 | 0.296 | 0.386 | 0.3735 | 0.0267 |
| 14 | 14 | 0.386 | 0.505 | 0.3592 | 0.0246 |
| 15 | 15 | 0.505 | 0.577 | 0.3047 | 0.0228 |
| 16 | 16 | 0.577 | 0.659 | 0.2698 | 0.0211 |
| 17 | 17 | 0.659 | 0.753 | 0.2329 | 0.0186 |
| 18 | 18 | 0.753 | 0.861 | 0.2119 | 0.0168 |
| 19 | 19 | 0.861 | 0.984 | 0.1637 | 0.0145 |
| 20 | 20 | 0.984 | 1.285 | 0.0996 | 0.0102 |
| 21 | 21 | 1.285 | 2.506 | 0.0139 | 0.0038 |

TABLE V: Unfolded 0pNp $E_\mu$ differential cross section results. Bin describes the binning structure for the given measurement and Global Bin describes the binning structure used in the blockwise covariance matrix. The Uncertainty column corresponds to the square root of the diagonal elements of the extracted covariance matrix.

| 0pNp $\cos\theta_\mu$ differential cross section | | | | | |
|---|---|---|---|---|---|
| Global Bin | Bin | $\cos\theta_\mu$ Low | $\cos\theta_\mu$ High | $\frac{d\sigma}{d\cos\theta_\mu}$ $(\times 10^{-36}\frac{\text{cm}^2}{\text{Ar}})$ | Uncertainty $(\times 10^{-36}\frac{\text{cm}^2}{\text{Ar}})$ |
| 0p | | | | | |
| 22 | 0 | -1 | -0.6 | 0.0064 | 0.0035 |
| 23 | 1 | -0.6 | -0.5 | 0.0074 | 0.0036 |
| 24 | 2 | -0.5 | -0.4 | 0.0079 | 0.0032 |
| 25 | 3 | -0.4 | -0.3 | 0.0085 | 0.0031 |
| 26 | 4 | -0.3 | -0.2 | 0.0094 | 0.0034 |
| 27 | 5 | -0.2 | -0.1 | 0.0094 | 0.0035 |
| 28 | 6 | -0.1 | 0 | 0.0096 | 0.0039 |
| 29 | 7 | 0 | 0.1 | 0.0099 | 0.0044 |
| 30 | 8 | 0.1 | 0.2 | 0.0096 | 0.0045 |
| 31 | 9 | 0.2 | 0.3 | 0.0107 | 0.0049 |
| 32 | 10 | 0.3 | 0.4 | 0.0138 | 0.0057 |
| 33 | 11 | 0.4 | 0.5 | 0.0190 | 0.0066 |
| 34 | 12 | 0.5 | 0.6 | 0.0276 | 0.0074 |
| 35 | 13 | 0.6 | 0.7 | 0.0437 | 0.0088 |
| 36 | 14 | 0.7 | 0.8 | 0.0711 | 0.0110 |
| 37 | 15 | 0.8 | 0.9 | 0.1215 | 0.0154 |
| 38 | 16 | 0.9 | 1 | 0.2051 | 0.0234 |
| Np | | | | | |
| 39 | 17 | -1 | -0.6 | 0.0366 | 0.0039 |
| 40 | 18 | -0.6 | -0.5 | 0.0411 | 0.0039 |
| 41 | 19 | -0.5 | -0.4 | 0.0430 | 0.0047 |
| 42 | 20 | -0.4 | -0.3 | 0.0481 | 0.0048 |
| 43 | 21 | -0.3 | -0.2 | 0.0561 | 0.0050 |
| 44 | 22 | -0.2 | -0.1 | 0.0646 | 0.0055 |
| 45 | 23 | -0.1 | 0 | 0.0753 | 0.0061 |
| 46 | 24 | 0 | 0.1 | 0.0848 | 0.0068 |
| 47 | 25 | 0.1 | 0.2 | 0.0958 | 0.0072 |
| 48 | 26 | 0.2 | 0.3 | 0.1110 | 0.0080 |
| 49 | 27 | 0.3 | 0.4 | 0.1326 | 0.0092 |
| 50 | 28 | 0.4 | 0.5 | 0.1648 | 0.0110 |
| 51 | 29 | 0.5 | 0.6 | 0.2012 | 0.0132 |
| 52 | 30 | 0.6 | 0.7 | 0.2477 | 0.0161 |
| 53 | 31 | 0.7 | 0.8 | 0.3087 | 0.0224 |
| 54 | 32 | 0.8 | 0.9 | 0.3912 | 0.0353 |
| 55 | 33 | 0.9 | 1 | 0.4623 | 0.0507 |

TABLE VI: Unfolded 0pNp $\cos\theta_\mu$ differential cross section results. Bin describes the binning structure for the given measurement and Global Bin describes the binning structure used in the blockwise covariance matrix. The Uncertainty column corresponds to the square root of the diagonal elements of the extracted covariance matrix.

| 0pNp cross section as a function of $E_\nu$ | | | | | |
|---|---|---|---|---|---|
| Global Bin | Bin | $E_\nu$ Low (GeV) | $E_\nu$ High (GeV) | $\sigma(E_\nu)$ ($\times 10^{-36} \frac{\text{cm}^2}{\text{Ar}}$) | Uncertainty ($\times 10^{-36} \frac{\text{cm}^2}{\text{Ar}}$) |
| 0p | | | | | |
| 56 | 0 | 0.2 | 0.54 | 0.0399 | 0.0053 |
| 57 | 1 | 0.54 | 0.705 | 0.0618 | 0.0057 |
| 58 | 2 | 0.705 | 0.805 | 0.0779 | 0.0071 |
| 59 | 3 | 0.805 | 0.92 | 0.0886 | 0.0103 |
| 60 | 4 | 0.92 | 1.05 | 0.0946 | 0.0132 |
| 61 | 5 | 1.05 | 1.2 | 0.0976 | 0.0154 |
| 62 | 6 | 1.2 | 1.375 | 0.0987 | 0.0187 |
| 63 | 7 | 1.375 | 1.57 | 0.1053 | 0.0247 |
| 64 | 8 | 1.57 | 2.05 | 0.1179 | 0.0324 |
| 65 | 9 | 2.05 | 4.0 | 0.1618 | 0.0483 |
| Np | | | | | |
| 66 | 10 | 0.2 | 0.54 | 0.0837 | 0.0102 |
| 67 | 11 | 0.54 | 0.705 | 0.2110 | 0.0177 |
| 68 | 12 | 0.705 | 0.805 | 0.3084 | 0.0233 |
| 69 | 13 | 0.805 | 0.92 | 0.3638 | 0.0256 |
| 70 | 14 | 0.92 | 1.05 | 0.3941 | 0.0286 |
| 71 | 15 | 1.05 | 1.2 | 0.4044 | 0.0352 |
| 72 | 16 | 1.2 | 1.375 | 0.4239 | 0.0441 |
| 73 | 17 | 1.375 | 1.57 | 0.4651 | 0.0626 |
| 74 | 18 | 1.57 | 2.05 | 0.5419 | 0.0846 |
| 75 | 19 | 2.05 | 4.0 | 0.6781 | 0.1144 |

TABLE VII: Unfolded 0pNp cross section as a function of $E_\nu$. Bin describes the binning structure for the given measurement and Global Bin describes the binning structure used in the blockwise covariance matrix. The Uncertainty column corresponds to the square root of the diagonal elements of the extracted covariance matrix.

| 0pNp $\nu$ differential cross section | | | | | |
|---|---|---|---|---|---|
| Global Bin | Bin | $\nu$ Low (GeV) | $\nu$ High (GeV) | $\frac{d\sigma}{d\nu}$ ($\times 10^{-36} \frac{\text{cm}^2}{\text{Ar GeV}}$) | Uncertainty ($\times 10^{-36} \frac{\text{cm}^2}{\text{Ar GeV}}$) |
| 0p | | | | | |
| 76 | 0 | 0 | 0.3 | 0.1411 | 0.0120 |
| 77 | 1 | 0.3 | 0.7 | 0.0383 | 0.0196 |
| 78 | 2 | 0.7 | 2.5 | 0.0014 | 0.0029 |
| Np | | | | | |
| 79 | 3 | 0 | 0.12 | 0.0986 | 0.0368 |
| 80 | 4 | 0.12 | 0.275 | 0.5341 | 0.0591 |
| 81 | 5 | 0.275 | 0.4 | 0.4408 | 0.0797 |
| 82 | 6 | 0.4 | 0.6 | 0.3018 | 0.0443 |
| 83 | 7 | 0.6 | 1.0 | 0.1093 | 0.0136 |
| 84 | 8 | 1.0 | 2.5 | 0.0082 | 0.0032 |

TABLE VIII: Unfolded 0pNp $\nu$ differential cross section results. Bin describes the binning structure for the given measurement and Global Bin describes the binning structure used in the blockwise covariance matrix. The Uncertainty column corresponds to the square root of the diagonal elements of the extracted covariance matrix.

| 0pNp $E_{avail}$ differential cross section | | | | | |
|---|---|---|---|---|---|
| Global Bin | Bin | $E_{avail}$ Low (GeV) | $E_{avail}$ High (GeV) | $\frac{d\sigma}{dE_{avail}}$ ($\times 10^{-36} \frac{\text{cm}^2}{\text{Ar GeV}}$) | Uncertainty ($\times 10^{-36} \frac{\text{cm}^2}{\text{Ar GeV}}$) |
| 0p | | | | | |
| 85 | 0 | 0 | 0.3 | 0.2509 | 0.0261 |
| 86 | 1 | 0.3 | 0.4 | 0.0652 | 0.0133 |
| 87 | 2 | 0.4 | 0.5 | 0.0208 | 0.0097 |
| 88 | 3 | 0.5 | 1.0 | 0.0045 | 0.0050 |
| 89 | 4 | 1.0 | 2.5 | 0.0015 | 0.0008 |
| Np | | | | | |
| 90 | 5 | 0 | 0.3 | 0.5034 | 0.0407 |
| 91 | 6 | 0.3 | 0.4 | 0.3482 | 0.0285 |
| 92 | 7 | 0.4 | 0.5 | 0.2299 | 0.0210 |
| 93 | 8 | 0.5 | 0.6 | 0.1445 | 0.0167 |
| 94 | 9 | 0.6 | 0.7 | 0.0921 | 0.0133 |
| 95 | 10 | 0.7 | 0.8 | 0.0548 | 0.0109 |
| 96 | 11 | 0.8 | 1.0 | 0.0316 | 0.0077 |
| 97 | 12 | 1.0 | 1.3 | 0.0129 | 0.0040 |
| 98 | 13 | 1.3 | 2.5 | 0.0018 | 0.0012 |

TABLE IX: Unfolded 0pNp $E_{avail}$ differential cross section results. Bin describes the binning structure for the given measurement and Global Bin describes the binning structure used in the blockwise covariance matrix. The Uncertainty column corresponds to the square root of the diagonal elements of the extracted covariance matrix.

| $K_p$ differential cross section | | | | | |
|---|---|---|---|---|---|
| Global Bin | Bin | $K_p$ Low (GeV) | $K_p$ High (GeV) | $\frac{d\sigma}{dK_p}$ ($\times 10^{-36} \frac{\text{cm}^2}{\text{Ar GeV}}$) | Uncertainty ($\times 10^{-36} \frac{\text{cm}^2}{\text{Ar GeV}}$) |
| 99 | 0 | 0 | 0.035 | 1.9323 | 0.3645 |
| 100 | 1 | 0.035 | 0.105 | 1.0636 | 0.1450 |
| 101 | 2 | 0.105 | 0.1225 | 1.0174 | 0.1058 |
| 102 | 3 | 0.1225 | 0.14 | 0.9820 | 0.0988 |
| 103 | 4 | 0.14 | 0.1575 | 0.8981 | 0.1073 |
| 104 | 5 | 0.1575 | 0.175 | 0.7884 | 0.0915 |
| 105 | 6 | 0.175 | 0.1925 | 0.7312 | 0.0742 |
| 106 | 7 | 0.1925 | 0.21 | 0.6157 | 0.0693 |
| 107 | 8 | 0.21 | 0.245 | 0.5464 | 0.0511 |
| 108 | 9 | 0.245 | 0.28 | 0.4212 | 0.0396 |
| 109 | 10 | 0.28 | 0.315 | 0.3387 | 0.0321 |
| 110 | 11 | 0.315 | 0.35 | 0.2589 | 0.0270 |
| 111 | 12 | 0.35 | 0.42 | 0.1994 | 0.0198 |
| 112 | 13 | 0.42 | 0.525 | 0.1136 | 0.0139 |
| 113 | 14 | 0.525 | 0.8 | 0.0335 | 0.0116 |

TABLE X: Unfolded $K_p$ differential cross section result. Bin describes the binning structure for the given measurement and Global Bin describes the binning structure used in the blockwise covariance matrix. The Uncertainty column corresponds to the square root of the diagonal elements of the extracted covariance matrix.

| $\cos\theta_p$ differential cross section | | | | | |
|---|---|---|---|---|---|
| Global Bin | Bin | $\cos\theta_p$ Low | $\cos\theta_p$ High | $\frac{d\sigma}{d\cos\theta_p}$ ($\times10^{-36}\frac{\text{cm}^2}{\text{Ar}}$) | Uncertainty ($\times10^{-36}\frac{\text{cm}^2}{\text{Ar}}$) |
| 114 | 0 | -1 | -0.9 | 0.0015 | 0.0046 |
| 115 | 1 | -0.9 | -0.8 | 0.0029 | 0.0046 |
| 116 | 2 | -0.8 | -0.7 | 0.0052 | 0.0044 |
| 117 | 3 | -0.7 | -0.6 | 0.0082 | 0.0045 |
| 118 | 4 | -0.6 | -0.5 | 0.0108 | 0.0045 |
| 119 | 5 | -0.5 | -0.4 | 0.0125 | 0.0045 |
| 120 | 6 | -0.4 | -0.3 | 0.0147 | 0.0049 |
| 121 | 7 | -0.3 | -0.2 | 0.0199 | 0.0055 |
| 122 | 8 | -0.2 | -0.1 | 0.0290 | 0.0061 |
| 123 | 9 | -0.1 | 0 | 0.0407 | 0.0069 |
| 124 | 10 | 0 | 0.1 | 0.0528 | 0.0077 |
| 125 | 11 | 0.1 | 0.2 | 0.0673 | 0.0087 |
| 126 | 12 | 0.2 | 0.3 | 0.0883 | 0.0103 |
| 127 | 13 | 0.3 | 0.4 | 0.1228 | 0.0125 |
| 128 | 14 | 0.4 | 0.5 | 0.1682 | 0.0154 |
| 129 | 15 | 0.5 | 0.6 | 0.2222 | 0.0188 |
| 130 | 16 | 0.6 | 0.7 | 0.2861 | 0.0230 |
| 131 | 17 | 0.7 | 0.8 | 0.3580 | 0.0282 |
| 132 | 18 | 0.8 | 0.9 | 0.4345 | 0.0346 |
| 133 | 19 | 0.9 | 1 | 0.5203 | 0.0431 |

TABLE XI: Unfolded $\cos\theta_p$ differential cross section result. Bin describes the binning structure for the given measurement and Global Bin describes the binning structure used in the blockwise covariance matrix. The Uncertainty column corresponds to the square root of the diagonal elements of the extracted covariance matrix.

| Cross section as a function of proton multiplicity | | | | |
|---|---|---|---|---|
| Global Bin | Bin | Multiplicity | $\sigma$ ($\times10^{-36}\frac{\text{cm}^2}{\text{Ar}}$) | Uncertainty ($\times10^{-36}\frac{\text{cm}^2}{\text{Ar}}$) |
| 134 | 0 | 0 | 0.0874 | 0.0151 |
| 135 | 1 | 1 | 0.1920 | 0.0164 |
| 136 | 2 | 2 | 0.0488 | 0.0101 |
| 137 | 3 | $> 2$ | 0.0148 | 0.0053 |

TABLE XII: Unfolded cross section as a function of multiplicity. Bin describes the binning structure for the given measurement and Global Bin describes the binning structure used in the blockwise covariance matrix. The Uncertainty column corresponds to the square root of the diagonal elements of the extracted covariance matrix.

| 0pNp $\cos\theta_\mu$ and $E_\mu$ double-differential cross section | | | | | | | |
|---|---|---|---|---|---|---|---|
| Global Bin | Bin | $\cos\theta_\mu$ Low | $\cos\theta_\mu$ High | $E_\mu$ Low (GeV) | $E_\mu$ High (GeV) | $\frac{d^2\sigma}{d\cos\theta_\mu dE_\mu}$ ($\times 10^{-36}\frac{\text{cm}^2}{\text{Ar GeV}}$) | Uncertainty ($\times 10^{-36}\frac{\text{cm}^2}{\text{Ar GeV}}$) |
| 0p | | | | | | | |
| 138 | 0 | -1 | -0.5 | 0.106 | 0.226 | 0.00652 | 0.00227 |
| 139 | 1 | -1 | -0.5 | 0.226 | 0.296 | 0.01443 | 0.00341 |
| 140 | 2 | -1 | -0.5 | 0.296 | 2.506 | 0.00053 | 0.00010 |
| 141 | 3 | -0.5 | 0 | 0.106 | 0.226 | 0.00615 | 0.00254 |
| 142 | 4 | -0.5 | 0 | 0.226 | 0.296 | 0.02031 | 0.00415 |
| 143 | 5 | -0.5 | 0 | 0.296 | 0.386 | 0.01580 | 0.00246 |
| 144 | 6 | -0.5 | 0 | 0.386 | 2.506 | 0.00067 | 0.00010 |
| 145 | 7 | 0 | 0.3 | 0.106 | 0.226 | 0.00554 | 0.00242 |
| 146 | 8 | 0 | 0.3 | 0.226 | 0.296 | 0.02283 | 0.00504 |
| 147 | 9 | 0 | 0.3 | 0.296 | 0.386 | 0.02476 | 0.00352 |
| 148 | 10 | 0 | 0.3 | 0.386 | 2.506 | 0.00235 | 0.00043 |
| 149 | 11 | 0.3 | 0.5 | 0.106 | 0.226 | 0.00520 | 0.00213 |
| 150 | 12 | 0.3 | 0.5 | 0.226 | 0.296 | 0.02290 | 0.00535 |
| 151 | 13 | 0.3 | 0.5 | 0.296 | 0.386 | 0.03408 | 0.00511 |
| 152 | 14 | 0.3 | 0.5 | 0.386 | 0.505 | 0.03759 | 0.00634 |
| 153 | 15 | 0.3 | 0.5 | 0.505 | 0.577 | 0.03076 | 0.00356 |
| 154 | 16 | 0.3 | 0.5 | 0.577 | 2.506 | 0.00200 | 0.00022 |
| 155 | 17 | 0.5 | 0.7 | 0.106 | 0.226 | 0.00533 | 0.00228 |
| 156 | 18 | 0.5 | 0.7 | 0.226 | 0.296 | 0.02082 | 0.00618 |
| 157 | 19 | 0.5 | 0.7 | 0.296 | 0.386 | 0.03998 | 0.00754 |
| 158 | 20 | 0.5 | 0.7 | 0.386 | 0.505 | 0.06162 | 0.00772 |
| 159 | 21 | 0.5 | 0.7 | 0.505 | 0.577 | 0.06453 | 0.00732 |
| 160 | 22 | 0.5 | 0.7 | 0.577 | 0.659 | 0.04579 | 0.00535 |
| 161 | 23 | 0.5 | 0.7 | 0.659 | 0.753 | 0.02669 | 0.00314 |
| 162 | 24 | 0.5 | 0.7 | 0.753 | 0.861 | 0.01302 | 0.00162 |
| 163 | 25 | 0.5 | 0.7 | 0.861 | 2.506 | 0.00094 | 0.00016 |
| 164 | 26 | 0.7 | 0.8 | 0.106 | 0.296 | 0.00712 | 0.00289 |
| 165 | 27 | 0.7 | 0.8 | 0.296 | 0.386 | 0.03687 | 0.00581 |
| 166 | 28 | 0.7 | 0.8 | 0.386 | 0.505 | 0.07374 | 0.00879 |
| 167 | 29 | 0.7 | 0.8 | 0.505 | 0.577 | 0.09042 | 0.00922 |
| 168 | 30 | 0.7 | 0.8 | 0.577 | 0.659 | 0.08027 | 0.00927 |
| 169 | 31 | 0.7 | 0.8 | 0.659 | 0.753 | 0.05918 | 0.00694 |
| 170 | 32 | 0.7 | 0.8 | 0.753 | 0.861 | 0.03405 | 0.00411 |
| 171 | 33 | 0.7 | 0.8 | 0.861 | 0.984 | 0.02128 | 0.00329 |
| 172 | 34 | 0.7 | 0.8 | 0.984 | 2.506 | 0.00232 | 0.00042 |
| 173 | 35 | 0.8 | 0.9 | 0.106 | 0.296 | 0.00426 | 0.00289 |
| 174 | 36 | 0.8 | 0.9 | 0.296 | 0.386 | 0.02919 | 0.00626 |
| 175 | 37 | 0.8 | 0.9 | 0.386 | 0.505 | 0.07524 | 0.01074 |
| 176 | 38 | 0.8 | 0.9 | 0.505 | 0.577 | 0.10432 | 0.01162 |
| 177 | 39 | 0.8 | 0.9 | 0.577 | 0.659 | 0.11531 | 0.01198 |
| 178 | 40 | 0.8 | 0.9 | 0.659 | 0.753 | 0.10733 | 0.01210 |
| 179 | 41 | 0.8 | 0.9 | 0.753 | 0.861 | 0.09633 | 0.00947 |
| 180 | 42 | 0.8 | 0.9 | 0.861 | 0.984 | 0.07758 | 0.00803 |
| 181 | 43 | 0.8 | 0.9 | 0.984 | 1.285 | 0.03987 | 0.00471 |
| 182 | 44 | 0.8 | 0.9 | 1.285 | 2.506 | 0.00417 | 0.00060 |
| 183 | 45 | 0.9 | 1 | 0.106 | 0.296 | 0.00088 | 0.00239 |
| 184 | 46 | 0.9 | 1 | 0.296 | 0.386 | 0.02101 | 0.00740 |
| 185 | 47 | 0.9 | 1 | 0.386 | 0.505 | 0.06760 | 0.01272 |

continued on next page

continued from previous page

| Global Bin | Bin | $\cos\theta_\mu$ Low | $\cos\theta_\mu$ High | $E_\mu$ Low (GeV) | $E_\mu$ High (GeV) | $\frac{d^2\sigma}{d\cos\theta_\mu dE_\mu}$ ($\times10^{-36}\frac{\text{cm}^2}{\text{Ar GeV}}$) | Uncertainty ($\times10^{-36}\frac{\text{cm}^2}{\text{Ar GeV}}$) |
|---|---|---|---|---|---|---|---|
| 186 | 48 | 0.9 | 1 | 0.505 | 0.577 | 0.09532 | 0.01260 |
| 187 | 49 | 0.9 | 1 | 0.577 | 0.659 | 0.12443 | 0.01517 |
| 188 | 50 | 0.9 | 1 | 0.659 | 0.753 | 0.16087 | 0.01426 |
| 189 | 51 | 0.9 | 1 | 0.753 | 0.861 | 0.21292 | 0.01773 |
| 190 | 52 | 0.9 | 1 | 0.861 | 0.984 | 0.22278 | 0.01964 |
| 191 | 53 | 0.9 | 1 | 0.984 | 1.285 | 0.18994 | 0.01699 |
| 192 | 54 | 0.9 | 1 | 1.285 | 2.506 | 0.03650 | 0.00555 |
| Np | | | | | | | |
| 193 | 55 | -1 | -0.5 | 0.106 | 0.226 | 0.07747 | 0.01481 |
| 194 | 56 | -1 | -0.5 | 0.226 | 0.296 | 0.19303 | 0.01547 |
| 195 | 57 | -1 | -0.5 | 0.296 | 0.386 | 0.10229 | 0.00950 |
| 196 | 58 | -1 | -0.5 | 0.386 | 2.506 | 0.00068 | 0.00023 |
| 197 | 59 | -0.5 | 0 | 0.106 | 0.226 | 0.06534 | 0.01360 |
| 198 | 60 | -0.5 | 0 | 0.226 | 0.296 | 0.18816 | 0.01535 |
| 199 | 61 | -0.5 | 0 | 0.296 | 0.386 | 0.21169 | 0.01533 |
| 200 | 62 | -0.5 | 0 | 0.386 | 0.505 | 0.09339 | 0.00992 |
| 201 | 63 | -0.5 | 0 | 0.505 | 0.577 | 0.02200 | 0.00312 |
| 202 | 64 | -0.5 | 0 | 0.577 | 2.506 | 0.00032 | 0.00006 |
| 203 | 65 | 0 | 0.3 | 0.106 | 0.226 | 0.06428 | 0.01432 |
| 204 | 66 | 0 | 0.3 | 0.226 | 0.296 | 0.20691 | 0.01967 |
| 205 | 67 | 0 | 0.3 | 0.296 | 0.386 | 0.25428 | 0.02058 |
| 206 | 68 | 0 | 0.3 | 0.386 | 0.505 | 0.22566 | 0.01984 |
| 207 | 69 | 0 | 0.3 | 0.505 | 0.577 | 0.13428 | 0.01354 |
| 208 | 70 | 0 | 0.3 | 0.577 | 0.659 | 0.06307 | 0.00851 |
| 209 | 71 | 0 | 0.3 | 0.659 | 2.506 | 0.00172 | 0.00029 |
| 210 | 72 | 0.3 | 0.5 | 0.106 | 0.226 | 0.05595 | 0.01296 |
| 211 | 73 | 0.3 | 0.5 | 0.226 | 0.296 | 0.18944 | 0.02119 |
| 212 | 74 | 0.3 | 0.5 | 0.296 | 0.386 | 0.22124 | 0.02498 |
| 213 | 75 | 0.3 | 0.5 | 0.386 | 0.505 | 0.31043 | 0.02557 |
| 214 | 76 | 0.3 | 0.5 | 0.505 | 0.577 | 0.31372 | 0.02661 |
| 215 | 77 | 0.3 | 0.5 | 0.577 | 0.659 | 0.22918 | 0.01882 |
| 216 | 78 | 0.3 | 0.5 | 0.659 | 0.753 | 0.11224 | 0.01325 |
| 217 | 79 | 0.3 | 0.5 | 0.753 | 0.861 | 0.03749 | 0.00511 |
| 218 | 80 | 0.3 | 0.5 | 0.861 | 2.506 | 0.00107 | 0.00016 |
| 219 | 81 | 0.5 | 0.7 | 0.106 | 0.226 | 0.04575 | 0.01328 |
| 220 | 82 | 0.5 | 0.7 | 0.226 | 0.296 | 0.18302 | 0.02160 |
| 221 | 83 | 0.5 | 0.7 | 0.296 | 0.386 | 0.25710 | 0.02510 |
| 222 | 84 | 0.5 | 0.7 | 0.386 | 0.505 | 0.38117 | 0.03033 |
| 223 | 85 | 0.5 | 0.7 | 0.505 | 0.577 | 0.46728 | 0.03311 |
| 224 | 86 | 0.5 | 0.7 | 0.577 | 0.659 | 0.42578 | 0.02905 |
| 225 | 87 | 0.5 | 0.7 | 0.659 | 0.753 | 0.28779 | 0.02646 |
| 226 | 88 | 0.5 | 0.7 | 0.753 | 0.861 | 0.15137 | 0.01807 |
| 227 | 89 | 0.5 | 0.7 | 0.861 | 0.984 | 0.07251 | 0.01042 |
| 228 | 90 | 0.5 | 0.7 | 0.984 | 2.506 | 0.00433 | 0.00074 |
| 229 | 91 | 0.7 | 0.8 | 0.106 | 0.226 | 0.02394 | 0.01070 |
| 230 | 92 | 0.7 | 0.8 | 0.226 | 0.296 | 0.11359 | 0.01892 |
| 231 | 93 | 0.7 | 0.8 | 0.296 | 0.386 | 0.24990 | 0.02425 |
| 232 | 94 | 0.7 | 0.8 | 0.386 | 0.505 | 0.36976 | 0.03423 |
| 233 | 95 | 0.7 | 0.8 | 0.505 | 0.577 | 0.49966 | 0.04173 |

continued on next page

continued from previous page

| Global Bin | Bin | $\cos\theta_\mu$ Low | $\cos\theta_\mu$ High | $E_\mu$ Low (GeV) | $E_\mu$ High (GeV) | $\frac{d^2\sigma}{d\cos\theta_\mu dE_\mu}$ ($\times 10^{-36} \frac{\text{cm}^2}{\text{Ar GeV}}$) | Uncertainty ($\times 10^{-36} \frac{\text{cm}^2}{\text{Ar GeV}}$) |
|---|---|---|---|---|---|---|---|
| 234 | 96 | 0.7 | 0.8 | 0.577 | 0.659 | 0.54037 | 0.04080 |
| 235 | 97 | 0.7 | 0.8 | 0.659 | 0.753 | 0.47126 | 0.04263 |
| 236 | 98 | 0.7 | 0.8 | 0.753 | 0.861 | 0.38377 | 0.03425 |
| 237 | 99 | 0.7 | 0.8 | 0.861 | 0.984 | 0.26227 | 0.02778 |
| 238 | 100 | 0.7 | 0.8 | 0.984 | 1.285 | 0.10295 | 0.01443 |
| 239 | 101 | 0.7 | 0.8 | 1.285 | 2.506 | 0.00513 | 0.00087 |
| 240 | 102 | 0.8 | 0.9 | 0.106 | 0.226 | 0.00678 | 0.00879 |
| 241 | 103 | 0.8 | 0.9 | 0.226 | 0.296 | 0.06822 | 0.01689 |
| 242 | 104 | 0.8 | 0.9 | 0.296 | 0.386 | 0.18117 | 0.02210 |
| 243 | 105 | 0.8 | 0.9 | 0.386 | 0.505 | 0.29558 | 0.03151 |
| 244 | 106 | 0.8 | 0.9 | 0.505 | 0.577 | 0.40656 | 0.03920 |
| 245 | 107 | 0.8 | 0.9 | 0.577 | 0.659 | 0.45926 | 0.04662 |
| 246 | 108 | 0.8 | 0.9 | 0.659 | 0.753 | 0.55078 | 0.05271 |
| 247 | 109 | 0.8 | 0.9 | 0.753 | 0.861 | 0.61614 | 0.05275 |
| 248 | 110 | 0.8 | 0.9 | 0.861 | 0.984 | 0.48886 | 0.04749 |
| 249 | 111 | 0.8 | 0.9 | 0.984 | 1.285 | 0.29180 | 0.03358 |
| 250 | 112 | 0.8 | 0.9 | 1.285 | 2.506 | 0.02866 | 0.00499 |
| 251 | 113 | 0.9 | 1 | 0.106 | 0.226 | 0.00120 | 0.00901 |
| 252 | 114 | 0.9 | 1 | 0.226 | 0.296 | 0.03343 | 0.01405 |
| 253 | 115 | 0.9 | 1 | 0.296 | 0.386 | 0.08148 | 0.01665 |
| 254 | 116 | 0.9 | 1 | 0.386 | 0.505 | 0.16937 | 0.01846 |
| 255 | 117 | 0.9 | 1 | 0.505 | 0.577 | 0.20494 | 0.03159 |
| 256 | 118 | 0.9 | 1 | 0.577 | 0.659 | 0.23187 | 0.04205 |
| 257 | 119 | 0.9 | 1 | 0.659 | 0.753 | 0.35676 | 0.04281 |
| 258 | 120 | 0.9 | 1 | 0.753 | 0.861 | 0.56180 | 0.04363 |
| 259 | 121 | 0.9 | 1 | 0.861 | 0.984 | 0.45531 | 0.06002 |
| 260 | 122 | 0.9 | 1 | 0.984 | 1.285 | 0.43240 | 0.05498 |
| 261 | 123 | 0.9 | 1 | 1.285 | 2.506 | 0.09820 | 0.01936 |

TABLE XIII: Unfolded 0pNp $\cos\theta_\mu$ and $E_\mu$ double-differential cross section results. Bin describes the binning structure for the given measurement and Global Bin describes the binning structure used in the blockwise covariance matrix. The Uncertainty column corresponds to the square root of the diagonal elements of the extracted covariance matrix.

| $\cos\theta_p$ and $K_p$ double-differential cross section | | | | | | | |
|---|---|---|---|---|---|---|---|
| Global Bin | Bin | $\cos\theta_p$ low | $\cos\theta_p$ High | $K_p$ Low (GeV) | $K_p$ High (GeV) | $\frac{d^2\sigma}{d\cos\theta_p dK_p}$ ($\times 10^{-36} \frac{\text{cm}^2}{\text{Ar GeV}}$) | Uncertainty ($\times 10^{-36} \frac{\text{cm}^2}{\text{Ar GeV}}$) |
| 262 | 0 | -1 | -0.5 | 0.035 | 0.105 | 0.07240 | 0.03100 |
| 263 | 1 | -1 | -0.5 | 0.105 | 0.1225 | 0.03378 | 0.01245 |
| 264 | 2 | -1 | -0.5 | 0.1225 | 0.14 | 0.03331 | 0.01108 |
| 265 | 3 | -1 | -0.5 | 0.14 | 0.1575 | 0.02899 | 0.00865 |
| 266 | 4 | -1 | -0.5 | 0.1575 | 0.175 | 0.02403 | 0.00666 |
| 267 | 5 | -1 | -0.5 | 0.175 | 0.1925 | 0.01292 | 0.00520 |
| 268 | 6 | -1 | -0.5 | 0.1925 | 0.21 | 0.00725 | 0.00294 |
| 269 | 7 | -1 | -0.5 | 0.21 | 0.8 | 0.00023 | 0.00027 |
| 270 | 8 | -0.5 | 0 | 0.035 | 0.105 | 0.19222 | 0.03342 |
| 271 | 9 | -0.5 | 0 | 0.105 | 0.1225 | 0.14242 | 0.02011 |
| 272 | 10 | -0.5 | 0 | 0.1225 | 0.14 | 0.10271 | 0.01496 |
| 273 | 11 | -0.5 | 0 | 0.14 | 0.1575 | 0.09815 | 0.01334 |
| 274 | 12 | -0.5 | 0 | 0.1575 | 0.175 | 0.06260 | 0.01176 |

continued on next page

continued from previous page

| Global Bin | Bin | $\cos\theta_p$ low | $\cos\theta_p$ High | $K_p$ Low (GeV) | $K_p$ High (GeV) | $\frac{d^2\sigma}{d\cos\theta_p dK_p}$ ($\times 10^{-36} \frac{\text{cm}^2}{\text{Ar GeV}}$) | Uncertainty ($\times 10^{-36} \frac{\text{cm}^2}{\text{Ar GeV}}$) |
|---|---|---|---|---|---|---|---|
| 275 | 13 | -0.5 | 0 | 0.175 | 0.1925 | 0.04534 | 0.00964 |
| 276 | 14 | -0.5 | 0 | 0.1925 | 0.21 | 0.03892 | 0.00857 |
| 277 | 15 | -0.5 | 0 | 0.21 | 0.245 | 0.01388 | 0.00473 |
| 278 | 16 | -0.5 | 0 | 0.245 | 0.8 | 0.00153 | 0.00039 |
| 279 | 17 | 0 | 0.3 | 0.035 | 0.105 | 0.48657 | 0.05268 |
| 280 | 18 | 0 | 0.3 | 0.105 | 0.1225 | 0.38399 | 0.03528 |
| 281 | 19 | 0 | 0.3 | 0.1225 | 0.14 | 0.27822 | 0.03074 |
| 282 | 20 | 0 | 0.3 | 0.14 | 0.1575 | 0.21929 | 0.02377 |
| 283 | 21 | 0 | 0.3 | 0.1575 | 0.175 | 0.17049 | 0.02091 |
| 284 | 22 | 0 | 0.3 | 0.175 | 0.1925 | 0.14951 | 0.02002 |
| 285 | 23 | 0 | 0.3 | 0.1925 | 0.21 | 0.06964 | 0.00887 |
| 286 | 24 | 0 | 0.3 | 0.21 | 0.245 | 0.06457 | 0.01145 |
| 287 | 25 | 0 | 0.3 | 0.245 | 0.28 | 0.04983 | 0.00682 |
| 288 | 26 | 0 | 0.3 | 0.28 | 0.315 | 0.02955 | 0.00359 |
| 289 | 27 | 0 | 0.3 | 0.315 | 0.8 | 0.00296 | 0.00072 |
| 290 | 28 | 0.3 | 0.5 | 0.035 | 0.105 | 0.71346 | 0.07816 |
| 291 | 29 | 0.3 | 0.5 | 0.105 | 0.1225 | 0.69494 | 0.06273 |
| 292 | 30 | 0.3 | 0.5 | 0.1225 | 0.14 | 0.62207 | 0.05805 |
| 293 | 31 | 0.3 | 0.5 | 0.14 | 0.1575 | 0.59210 | 0.05074 |
| 294 | 32 | 0.3 | 0.5 | 0.1575 | 0.175 | 0.48052 | 0.04455 |
| 295 | 33 | 0.3 | 0.5 | 0.175 | 0.1925 | 0.38039 | 0.03770 |
| 296 | 34 | 0.3 | 0.5 | 0.1925 | 0.21 | 0.32630 | 0.03459 |
| 297 | 35 | 0.3 | 0.5 | 0.21 | 0.245 | 0.25276 | 0.02688 |
| 298 | 36 | 0.3 | 0.5 | 0.245 | 0.28 | 0.17629 | 0.01919 |
| 299 | 37 | 0.3 | 0.5 | 0.28 | 0.315 | 0.11106 | 0.01224 |
| 300 | 38 | 0.3 | 0.5 | 0.315 | 0.35 | 0.04910 | 0.00597 |
| 301 | 39 | 0.3 | 0.5 | 0.35 | 0.8 | 0.00936 | 0.00141 |
| 302 | 40 | 0.5 | 0.7 | 0.035 | 0.105 | 0.90862 | 0.09406 |
| 303 | 41 | 0.5 | 0.7 | 0.105 | 0.1225 | 1.02599 | 0.08633 |
| 304 | 42 | 0.5 | 0.7 | 0.1225 | 0.14 | 0.98754 | 0.08316 |
| 305 | 43 | 0.5 | 0.7 | 0.14 | 0.1575 | 0.88903 | 0.07569 |
| 306 | 44 | 0.5 | 0.7 | 0.1575 | 0.175 | 0.84011 | 0.07201 |
| 307 | 45 | 0.5 | 0.7 | 0.175 | 0.1925 | 0.72015 | 0.06630 |
| 308 | 46 | 0.5 | 0.7 | 0.1925 | 0.21 | 0.62607 | 0.06296 |
| 309 | 47 | 0.5 | 0.7 | 0.21 | 0.245 | 0.55368 | 0.05145 |
| 310 | 48 | 0.5 | 0.7 | 0.245 | 0.28 | 0.44683 | 0.04306 |
| 311 | 49 | 0.5 | 0.7 | 0.28 | 0.315 | 0.33026 | 0.03261 |
| 312 | 50 | 0.5 | 0.7 | 0.315 | 0.35 | 0.21888 | 0.02541 |
| 313 | 51 | 0.5 | 0.7 | 0.35 | 0.42 | 0.13939 | 0.01704 |
| 314 | 52 | 0.5 | 0.7 | 0.42 | 0.525 | 0.05425 | 0.00746 |
| 315 | 53 | 0.5 | 0.7 | 0.525 | 0.8 | 0.01005 | 0.00219 |
| 316 | 54 | 0.7 | 0.8 | 0.035 | 0.105 | 1.03581 | 0.09931 |
| 317 | 55 | 0.7 | 0.8 | 0.105 | 0.1225 | 1.13305 | 0.09262 |
| 318 | 56 | 0.7 | 0.8 | 0.1225 | 0.14 | 1.11089 | 0.09673 |
| 319 | 57 | 0.7 | 0.8 | 0.14 | 0.1575 | 0.94466 | 0.08717 |
| 320 | 58 | 0.7 | 0.8 | 0.1575 | 0.175 | 0.93632 | 0.08871 |
| 321 | 59 | 0.7 | 0.8 | 0.175 | 0.1925 | 0.94144 | 0.09407 |
| 322 | 60 | 0.7 | 0.8 | 0.1925 | 0.21 | 0.83820 | 0.08283 |
| 323 | 61 | 0.7 | 0.8 | 0.21 | 0.245 | 0.80307 | 0.07171 |

continued on next page

continued from previous page

| Global Bin | Bin | $\cos\theta_p$ low | $\cos\theta_p$ High | $K_p$ Low (GeV) | $K_p$ High (GeV) | $\frac{d^2\sigma}{d\cos\theta_p dK_p}$ ($\times10^{-36}\frac{\text{cm}^2}{\text{Ar GeV}}$) | Uncertainty ($\times10^{-36}\frac{\text{cm}^2}{\text{Ar GeV}}$) |
|---|---|---|---|---|---|---|---|
| 324 | 62 | 0.7 | 0.8 | 0.245 | 0.28 | 0.66662 | 0.06385 |
| 325 | 63 | 0.7 | 0.8 | 0.28 | 0.315 | 0.58290 | 0.05197 |
| 326 | 64 | 0.7 | 0.8 | 0.315 | 0.35 | 0.47355 | 0.04505 |
| 327 | 65 | 0.7 | 0.8 | 0.35 | 0.42 | 0.37479 | 0.03469 |
| 328 | 66 | 0.7 | 0.8 | 0.42 | 0.525 | 0.17690 | 0.02063 |
| 329 | 67 | 0.7 | 0.8 | 0.525 | 0.8 | 0.03806 | 0.00872 |
| 330 | 68 | 0.8 | 0.9 | 0.035 | 0.105 | 1.11724 | 0.10850 |
| 331 | 69 | 0.8 | 0.9 | 0.105 | 0.1225 | 1.19203 | 0.10197 |
| 332 | 70 | 0.8 | 0.9 | 0.1225 | 0.14 | 1.12271 | 0.10231 |
| 333 | 71 | 0.8 | 0.9 | 0.14 | 0.1575 | 1.01675 | 0.09160 |
| 334 | 72 | 0.8 | 0.9 | 0.1575 | 0.175 | 1.09754 | 0.09943 |
| 335 | 73 | 0.8 | 0.9 | 0.175 | 0.1925 | 1.08460 | 0.10171 |
| 336 | 74 | 0.8 | 0.9 | 0.1925 | 0.21 | 0.99510 | 0.09470 |
| 337 | 75 | 0.8 | 0.9 | 0.21 | 0.245 | 0.93419 | 0.08724 |
| 338 | 76 | 0.8 | 0.9 | 0.245 | 0.28 | 0.78141 | 0.07263 |
| 339 | 77 | 0.8 | 0.9 | 0.28 | 0.315 | 0.68312 | 0.06443 |
| 340 | 78 | 0.8 | 0.9 | 0.315 | 0.35 | 0.58252 | 0.05387 |
| 341 | 79 | 0.8 | 0.9 | 0.35 | 0.42 | 0.51988 | 0.04503 |
| 342 | 80 | 0.8 | 0.9 | 0.42 | 0.525 | 0.32856 | 0.03376 |
| 343 | 81 | 0.8 | 0.9 | 0.525 | 0.8 | 0.10378 | 0.02002 |
| 344 | 82 | 0.9 | 1 | 0.035 | 0.105 | 1.22812 | 0.12728 |
| 345 | 83 | 0.9 | 1 | 0.105 | 0.1225 | 1.31989 | 0.12990 |
| 346 | 84 | 0.9 | 1 | 0.1225 | 0.14 | 1.27551 | 0.13671 |
| 347 | 85 | 0.9 | 1 | 0.14 | 0.1575 | 1.22133 | 0.11990 |
| 348 | 86 | 0.9 | 1 | 0.1575 | 0.175 | 1.32071 | 0.12317 |
| 349 | 87 | 0.9 | 1 | 0.175 | 0.1925 | 1.22109 | 0.12217 |
| 350 | 88 | 0.9 | 1 | 0.1925 | 0.21 | 1.06913 | 0.12179 |
| 351 | 89 | 0.9 | 1 | 0.21 | 0.245 | 1.05762 | 0.10812 |
| 352 | 90 | 0.9 | 1 | 0.245 | 0.28 | 0.91116 | 0.09864 |
| 353 | 91 | 0.9 | 1 | 0.28 | 0.315 | 0.77007 | 0.08611 |
| 354 | 92 | 0.9 | 1 | 0.315 | 0.35 | 0.69381 | 0.07828 |
| 355 | 93 | 0.9 | 1 | 0.35 | 0.42 | 0.58983 | 0.06249 |
| 356 | 94 | 0.9 | 1 | 0.42 | 0.525 | 0.46670 | 0.05269 |
| 357 | 95 | 0.9 | 1 | 0.525 | 0.8 | 0.22252 | 0.04247 |

TABLE XIV: Unfolded $\cos\theta_p$ and $K_p$ double-differential cross section results. Bin describes the binning structure for the given measurement and Global Bin describes the binning structure used in the blockwise covariance matrix. The Uncertainty column corresponds to the square root of the diagonal elements of the extracted covariance matrix.

| Xp $E_\mu$ differential cross section | | | | | |
|---|---|---|---|---|---|
| Global Bin | Bin | $E_\mu$ Low (GeV) | $E_\mu$ High (GeV) | $\frac{d\sigma}{dE_\mu}$ ($\times 10^{-36} \frac{\text{cm}^2}{\text{Ar GeV}}$) | Uncertainty ($\times 10^{-36} \frac{\text{cm}^2}{\text{Ar GeV}}$) |
| 358 | 0 | 0.106 | 0.226 | 0.2080 | 0.0276 |
| 359 | 1 | 0.226 | 0.296 | 0.4137 | 0.0307 |
| 360 | 2 | 0.296 | 0.386 | 0.4994 | 0.0304 |
| 361 | 3 | 0.386 | 0.505 | 0.4652 | 0.0275 |
| 362 | 4 | 0.505 | 0.577 | 0.4068 | 0.0263 |
| 363 | 5 | 0.577 | 0.659 | 0.3455 | 0.0236 |
| 364 | 6 | 0.659 | 0.753 | 0.3051 | 0.0207 |
| 365 | 7 | 0.753 | 0.861 | 0.2730 | 0.0196 |
| 366 | 8 | 0.861 | 0.984 | 0.2215 | 0.0166 |
| 367 | 9 | 0.984 | 1.285 | 0.1226 | 0.0116 |
| 368 | 10 | 1.285 | 2.506 | 0.0228 | 0.0039 |

TABLE XV: Unfolded $E_\mu$ differential cross section result. Bin describes the binning structure for the given measurement and Global Bin describes the binning structure used in the blockwise covariance matrix. The Uncertainty column corresponds to the square root of the diagonal elements of the extracted covariance matrix.

| Xp $\cos\theta_\mu$ differential cross section | | | | | |
|---|---|---|---|---|---|
| Global Bin | Bin | $\cos\theta_\mu$ Low | $\cos\theta_\mu$ High | $\frac{d\sigma}{d\cos\theta_\mu}$ ($\times 10^{-36} \frac{\text{cm}^2}{\text{Ar}}$) | Uncertainty ($\times 10^{-36} \frac{\text{cm}^2}{\text{Ar}}$) |
| 369 | 0 | -1 | -0.6 | 0.0423 | 0.0042 |
| 370 | 1 | -0.6 | -0.5 | 0.0469 | 0.0043 |
| 371 | 2 | -0.5 | -0.4 | 0.0490 | 0.0052 |
| 372 | 3 | -0.4 | -0.3 | 0.0557 | 0.0053 |
| 373 | 4 | -0.3 | -0.2 | 0.0667 | 0.0056 |
| 374 | 5 | -0.2 | -0.1 | 0.0771 | 0.0062 |
| 375 | 6 | -0.1 | 0 | 0.0883 | 0.0068 |
| 376 | 7 | 0 | 0.1 | 0.0984 | 0.0077 |
| 377 | 8 | 0.1 | 0.2 | 0.1109 | 0.0082 |
| 378 | 9 | 0.2 | 0.3 | 0.1306 | 0.0091 |
| 379 | 10 | 0.3 | 0.4 | 0.1591 | 0.0105 |
| 380 | 11 | 0.4 | 0.5 | 0.1975 | 0.0126 |
| 381 | 12 | 0.5 | 0.6 | 0.2402 | 0.0151 |
| 382 | 13 | 0.6 | 0.7 | 0.3005 | 0.0184 |
| 383 | 14 | 0.7 | 0.8 | 0.3918 | 0.0256 |
| 384 | 15 | 0.8 | 0.9 | 0.5392 | 0.0398 |
| 385 | 16 | 0.9 | 1 | 0.7085 | 0.0588 |

TABLE XVI: Unfolded $\cos\theta_\mu$ differential cross section result. Bin describes the binning structure for the given measurement and Global Bin describes the binning structure used in the blockwise covariance matrix. The Uncertainty column corresponds to the square root of the diagonal elements of the extracted covariance matrix.

| Xp $\cos\theta_\mu$ and $E_\mu$ double-differential cross section results | | | | | | | |
|---|---|---|---|---|---|---|---|
| Global Bin | Bin | $\cos\theta_\mu$ Low | $\cos\theta_\mu$ High | $E_\mu$ Low (GeV) | $E_\mu$ High (GeV) | $\frac{d^2\sigma}{d\cos\theta_\mu dE_\mu}$ ($\times 10^{-36} \frac{\text{cm}^2}{\text{Ar GeV}}$) | Uncertainty ($\times 10^{-36} \frac{\text{cm}^2}{\text{Ar GeV}}$) |
| 386 | 0 | -1 | -0.5 | 0.106 | 0.226 | 0.1229 | 0.0226 |
| 387 | 1 | -1 | -0.5 | 0.226 | 0.296 | 0.1938 | 0.0203 |
| 388 | 2 | -1 | -0.5 | 0.296 | 0.386 | 0.1358 | 0.0145 |
| 389 | 3 | -1 | -0.5 | 0.386 | 2.506 | 0.0012 | 0.0004 |
| 390 | 4 | -0.5 | 0 | 0.106 | 0.226 | 0.1225 | 0.0148 |
| 391 | 5 | -0.5 | 0 | 0.226 | 0.296 | 0.2292 | 0.0163 |
| 392 | 6 | -0.5 | 0 | 0.296 | 0.386 | 0.2393 | 0.0180 |
| 393 | 7 | -0.5 | 0 | 0.386 | 0.505 | 0.1074 | 0.0125 |
| 394 | 8 | -0.5 | 0 | 0.505 | 0.577 | 0.0240 | 0.0050 |
| 395 | 9 | -0.5 | 0 | 0.577 | 2.506 | 0.0006 | 0.0006 |
| 396 | 10 | 0 | 0.3 | 0.106 | 0.226 | 0.0911 | 0.0252 |
| 397 | 11 | 0 | 0.3 | 0.226 | 0.296 | 0.2456 | 0.0271 |
| 398 | 12 | 0 | 0.3 | 0.296 | 0.386 | 0.2995 | 0.0266 |
| 399 | 13 | 0 | 0.3 | 0.386 | 0.505 | 0.3057 | 0.0226 |
| 400 | 14 | 0 | 0.3 | 0.505 | 0.577 | 0.1576 | 0.0264 |
| 401 | 15 | 0 | 0.3 | 0.577 | 0.659 | 0.0513 | 0.0084 |
| 402 | 16 | 0 | 0.3 | 0.659 | 2.506 | 0.0012 | 0.0016 |
| 403 | 17 | 0.3 | 0.5 | 0.106 | 0.226 | 0.0758 | 0.0318 |
| 404 | 18 | 0.3 | 0.5 | 0.226 | 0.296 | 0.2386 | 0.0342 |
| 405 | 19 | 0.3 | 0.5 | 0.296 | 0.386 | 0.3242 | 0.0327 |
| 406 | 20 | 0.3 | 0.5 | 0.386 | 0.505 | 0.4264 | 0.0326 |
| 407 | 21 | 0.3 | 0.5 | 0.505 | 0.577 | 0.3572 | 0.0317 |
| 408 | 22 | 0.3 | 0.5 | 0.577 | 0.659 | 0.2707 | 0.0195 |
| 409 | 23 | 0.3 | 0.5 | 0.659 | 0.753 | 0.1428 | 0.0120 |
| 410 | 24 | 0.3 | 0.5 | 0.753 | 0.861 | 0.0528 | 0.0072 |
| 411 | 25 | 0.3 | 0.5 | 0.861 | 2.506 | 0.0026 | 0.0014 |
| 412 | 26 | 0.5 | 0.7 | 0.106 | 0.226 | 0.0619 | 0.0258 |
| 413 | 27 | 0.5 | 0.7 | 0.226 | 0.296 | 0.2152 | 0.0274 |
| 414 | 28 | 0.5 | 0.7 | 0.296 | 0.386 | 0.3253 | 0.0293 |
| 415 | 29 | 0.5 | 0.7 | 0.386 | 0.505 | 0.4917 | 0.0362 |
| 416 | 30 | 0.5 | 0.7 | 0.505 | 0.577 | 0.5129 | 0.0451 |
| 417 | 31 | 0.5 | 0.7 | 0.577 | 0.659 | 0.5024 | 0.0360 |
| 418 | 32 | 0.5 | 0.7 | 0.659 | 0.753 | 0.3813 | 0.0355 |
| 419 | 33 | 0.5 | 0.7 | 0.753 | 0.861 | 0.1954 | 0.0278 |
| 420 | 34 | 0.5 | 0.7 | 0.861 | 0.984 | 0.0758 | 0.0115 |
| 421 | 35 | 0.5 | 0.7 | 0.984 | 2.506 | 0.0088 | 0.0041 |
| 422 | 36 | 0.7 | 0.8 | 0.106 | 0.226 | 0.0155 | 0.0245 |
| 423 | 37 | 0.7 | 0.8 | 0.226 | 0.296 | 0.1562 | 0.0265 |
| 424 | 38 | 0.7 | 0.8 | 0.296 | 0.386 | 0.3147 | 0.0319 |
| 425 | 39 | 0.7 | 0.8 | 0.386 | 0.505 | 0.4913 | 0.0365 |
| 426 | 40 | 0.7 | 0.8 | 0.505 | 0.577 | 0.6139 | 0.0478 |
| 427 | 41 | 0.7 | 0.8 | 0.577 | 0.659 | 0.6881 | 0.0528 |
| 428 | 42 | 0.7 | 0.8 | 0.659 | 0.753 | 0.6334 | 0.0530 |
| 429 | 43 | 0.7 | 0.8 | 0.753 | 0.861 | 0.4702 | 0.0476 |
| 430 | 44 | 0.7 | 0.8 | 0.861 | 0.984 | 0.2958 | 0.0355 |
| 431 | 45 | 0.7 | 0.8 | 0.984 | 1.285 | 0.1321 | 0.0168 |
| 432 | 46 | 0.7 | 0.8 | 1.285 | 2.506 | 0.0201 | 0.0047 |
| 433 | 47 | 0.8 | 0.9 | 0.106 | 0.226 | 0.0172 | 0.0185 |
| 434 | 48 | 0.8 | 0.9 | 0.226 | 0.296 | 0.1443 | 0.0232 |

continued on next page

continued from previous page

| Global Bin | Bin | $\cos\theta_\mu$ Low | $\cos\theta_\mu$ High | $E_\mu$ Low (GeV) | $E_\mu$ High (GeV) | $\frac{d^2\sigma}{d\cos\theta_\mu dE_\mu}$ ($\times 10^{-36}\frac{\text{cm}^2}{\text{Ar GeV}}$) | Uncertainty ($\times 10^{-36}\frac{\text{cm}^2}{\text{Ar GeV}}$) |
|---|---|---|---|---|---|---|---|
| 435 | 49 | 0.8 | 0.9 | 0.296 | 0.386 | 0.2494 | 0.0291 |
| 436 | 50 | 0.8 | 0.9 | 0.386 | 0.505 | 0.3655 | 0.0400 |
| 437 | 51 | 0.8 | 0.9 | 0.505 | 0.577 | 0.5536 | 0.0454 |
| 438 | 52 | 0.8 | 0.9 | 0.577 | 0.659 | 0.6248 | 0.0572 |
| 439 | 53 | 0.8 | 0.9 | 0.659 | 0.753 | 0.7094 | 0.0566 |
| 440 | 54 | 0.8 | 0.9 | 0.753 | 0.861 | 0.7089 | 0.0577 |
| 441 | 55 | 0.8 | 0.9 | 0.861 | 0.984 | 0.5810 | 0.0581 |
| 442 | 56 | 0.8 | 0.9 | 0.984 | 1.285 | 0.3292 | 0.0288 |
| 443 | 57 | 0.8 | 0.9 | 1.285 | 2.506 | 0.0614 | 0.0099 |
| 444 | 58 | 0.9 | 1 | 0.106 | 0.226 | 0.0206 | 0.0194 |
| 445 | 59 | 0.9 | 1 | 0.226 | 0.296 | 0.0865 | 0.0261 |
| 446 | 60 | 0.9 | 1 | 0.296 | 0.386 | 0.1102 | 0.0272 |
| 447 | 61 | 0.9 | 1 | 0.386 | 0.505 | 0.2818 | 0.0310 |
| 448 | 62 | 0.9 | 1 | 0.505 | 0.577 | 0.4142 | 0.0465 |
| 449 | 63 | 0.9 | 1 | 0.577 | 0.659 | 0.4093 | 0.0505 |
| 450 | 64 | 0.9 | 1 | 0.659 | 0.753 | 0.6005 | 0.0560 |
| 451 | 65 | 0.9 | 1 | 0.753 | 0.861 | 0.8366 | 0.0671 |
| 452 | 66 | 0.9 | 1 | 0.861 | 0.984 | 0.8516 | 0.0730 |
| 453 | 67 | 0.9 | 1 | 0.984 | 1.285 | 0.6476 | 0.0655 |
| 454 | 68 | 0.9 | 1 | 1.285 | 2.506 | 0.1755 | 0.0209 |

TABLE XVII: Unfolded Xp $\cos\theta_\mu$ and $E_\mu$ double-differential cross section result. Bin describes the binning structure for the given measurement and Global Bin describes the binning structure used in the blockwise covariance matrix. The Uncertainty column corresponds to the square root of the diagonal elements of the extracted covariance matrix.

Xp $E_{avail}$, $\cos\theta_\mu$ and $E_\mu$ triple-differential cross section

| Global Bin | Bin | $E_{avail}$ Low (GeV) | $E_{avail}$ High (GeV) | $\cos\theta_\mu$ Low | $\cos\theta_\mu$ High | $E_\mu$ Low (GeV) | $E_\mu$ High (GeV) | $\frac{d^3\sigma}{dE_{avail}d\cos\theta_\mu dE_\mu}$ ($\times 10^{-36}\frac{\text{cm}^2}{\text{Ar GeV}^2}$) | Uncertainty ($\times 10^{-36}\frac{\text{cm}^2}{\text{Ar GeV}^2}$) |
|---|---|---|---|---|---|---|---|---|---|
| 455 | 0 | 0 | 0.3 | -1 | -0.5 | 0.106 | 0.226 | 0.2257 | 0.0459 |
| 456 | 1 | 0 | 0.3 | -1 | -0.5 | 0.226 | 0.296 | 0.3085 | 0.0382 |
| 457 | 2 | 0 | 0.3 | -1 | -0.5 | 0.296 | 0.386 | 0.1613 | 0.0206 |
| 458 | 3 | 0 | 0.3 | -1 | -0.5 | 0.386 | 2.506 | 0.0010 | 0.0002 |
| 459 | 4 | 0 | 0.3 | -0.5 | 0 | 0.106 | 0.226 | 0.1764 | 0.0328 |
| 460 | 5 | 0 | 0.3 | -0.5 | 0 | 0.226 | 0.296 | 0.4063 | 0.0398 |
| 461 | 6 | 0 | 0.3 | -0.5 | 0 | 0.296 | 0.386 | 0.3960 | 0.0360 |
| 462 | 7 | 0 | 0.3 | -0.5 | 0 | 0.386 | 0.505 | 0.1397 | 0.0198 |
| 463 | 8 | 0 | 0.3 | -0.5 | 0 | 0.505 | 2.506 | 0.0009 | 0.0002 |
| 464 | 9 | 0 | 0.3 | 0 | 0.3 | 0.106 | 0.226 | 0.1004 | 0.0346 |
| 465 | 10 | 0 | 0.3 | 0 | 0.3 | 0.226 | 0.296 | 0.4416 | 0.0471 |
| 466 | 11 | 0 | 0.3 | 0 | 0.3 | 0.296 | 0.386 | 0.5614 | 0.0543 |
| 467 | 12 | 0 | 0.3 | 0 | 0.3 | 0.386 | 0.505 | 0.4323 | 0.0433 |
| 468 | 13 | 0 | 0.3 | 0 | 0.3 | 0.505 | 0.577 | 0.1441 | 0.0220 |
| 469 | 14 | 0 | 0.3 | 0 | 0.3 | 0.577 | 2.506 | 0.0033 | 0.0007 |
| 470 | 15 | 0 | 0.3 | 0.3 | 0.5 | 0.106 | 0.226 | 0.1127 | 0.0342 |
| 471 | 16 | 0 | 0.3 | 0.3 | 0.5 | 0.226 | 0.296 | 0.4775 | 0.0515 |
| 472 | 17 | 0 | 0.3 | 0.3 | 0.5 | 0.296 | 0.386 | 0.6305 | 0.0604 |
| 473 | 18 | 0 | 0.3 | 0.3 | 0.5 | 0.386 | 0.505 | 0.8133 | 0.0628 |
| 474 | 19 | 0 | 0.3 | 0.3 | 0.5 | 0.505 | 0.577 | 0.5487 | 0.0530 |
| 475 | 20 | 0 | 0.3 | 0.3 | 0.5 | 0.577 | 0.659 | 0.2980 | 0.0330 |

continued on next page

continued from previous page

| Global Bin | Bin | $E_{avail}$ Low (GeV) | $E_{avail}$ High (GeV) | $\cos\theta_\mu$ Low | $\cos\theta_\mu$ High | $E_\mu$ Low (GeV) | $E_\mu$ High (GeV) | $\frac{d^3\sigma}{dE_{avail}d\cos\theta_\mu dE_\mu}$ ($\times 10^{-36}\frac{\text{cm}^2}{\text{Ar GeV}^2}$) | Uncertainty ($\times 10^{-36}\frac{\text{cm}^2}{\text{Ar GeV}^2}$) |
|---|---|---|---|---|---|---|---|---|---|
| 476 | 21 | 0 | 0.3 | 0.3 | 0.5 | 0.659 | 0.753 | 0.1295 | 0.0149 |
| 477 | 22 | 0 | 0.3 | 0.3 | 0.5 | 0.753 | 2.506 | 0.0035 | 0.0005 |
| 478 | 23 | 0 | 0.3 | 0.5 | 0.7 | 0.106 | 0.226 | 0.1161 | 0.0365 |
| 479 | 24 | 0 | 0.3 | 0.5 | 0.7 | 0.226 | 0.296 | 0.4018 | 0.0552 |
| 480 | 25 | 0 | 0.3 | 0.5 | 0.7 | 0.296 | 0.386 | 0.5747 | 0.0613 |
| 481 | 26 | 0 | 0.3 | 0.5 | 0.7 | 0.386 | 0.505 | 0.9743 | 0.0741 |
| 482 | 27 | 0 | 0.3 | 0.5 | 0.7 | 0.505 | 0.577 | 1.1080 | 0.1044 |
| 483 | 28 | 0 | 0.3 | 0.5 | 0.7 | 0.577 | 0.659 | 0.9999 | 0.0834 |
| 484 | 29 | 0 | 0.3 | 0.5 | 0.7 | 0.659 | 0.753 | 0.7008 | 0.0663 |
| 485 | 30 | 0 | 0.3 | 0.5 | 0.7 | 0.753 | 0.861 | 0.3367 | 0.0408 |
| 486 | 31 | 0 | 0.3 | 0.5 | 0.7 | 0.861 | 0.984 | 0.1191 | 0.0153 |
| 487 | 32 | 0 | 0.3 | 0.5 | 0.7 | 0.984 | 2.506 | 0.0042 | 0.0006 |
| 488 | 33 | 0 | 0.3 | 0.7 | 0.8 | 0.106 | 0.226 | 0.0744 | 0.0254 |
| 489 | 34 | 0 | 0.3 | 0.7 | 0.8 | 0.226 | 0.296 | 0.2340 | 0.0421 |
| 490 | 35 | 0 | 0.3 | 0.7 | 0.8 | 0.296 | 0.386 | 0.5245 | 0.0540 |
| 491 | 36 | 0 | 0.3 | 0.7 | 0.8 | 0.386 | 0.505 | 1.0020 | 0.0830 |
| 492 | 37 | 0 | 0.3 | 0.7 | 0.8 | 0.505 | 0.577 | 1.4747 | 0.1230 |
| 493 | 38 | 0 | 0.3 | 0.7 | 0.8 | 0.577 | 0.659 | 1.6545 | 0.1308 |
| 494 | 39 | 0 | 0.3 | 0.7 | 0.8 | 0.659 | 0.753 | 1.5524 | 0.1085 |
| 495 | 40 | 0 | 0.3 | 0.7 | 0.8 | 0.753 | 0.861 | 1.1306 | 0.1042 |
| 496 | 41 | 0 | 0.3 | 0.7 | 0.8 | 0.861 | 0.984 | 0.6664 | 0.0692 |
| 497 | 42 | 0 | 0.3 | 0.7 | 0.8 | 0.984 | 2.506 | 0.0443 | 0.0057 |
| 498 | 43 | 0 | 0.3 | 0.8 | 0.9 | 0.106 | 0.226 | 0.0423 | 0.0207 |
| 499 | 44 | 0 | 0.3 | 0.8 | 0.9 | 0.226 | 0.296 | 0.1565 | 0.0433 |
| 500 | 45 | 0 | 0.3 | 0.8 | 0.9 | 0.296 | 0.386 | 0.4337 | 0.0594 |
| 501 | 46 | 0 | 0.3 | 0.8 | 0.9 | 0.386 | 0.505 | 0.8476 | 0.0936 |
| 502 | 47 | 0 | 0.3 | 0.8 | 0.9 | 0.505 | 0.577 | 1.2958 | 0.1340 |
| 503 | 48 | 0 | 0.3 | 0.8 | 0.9 | 0.577 | 0.659 | 1.4168 | 0.1342 |
| 504 | 49 | 0 | 0.3 | 0.8 | 0.9 | 0.659 | 0.753 | 1.6751 | 0.1605 |
| 505 | 50 | 0 | 0.3 | 0.8 | 0.9 | 0.753 | 0.861 | 1.7370 | 0.1527 |
| 506 | 51 | 0 | 0.3 | 0.8 | 0.9 | 0.861 | 0.984 | 1.5487 | 0.1202 |
| 507 | 52 | 0 | 0.3 | 0.8 | 0.9 | 0.984 | 1.285 | 0.8132 | 0.0889 |
| 508 | 53 | 0 | 0.3 | 0.8 | 0.9 | 1.285 | 2.506 | 0.0529 | 0.0064 |
| 509 | 54 | 0 | 0.3 | 0.9 | 1 | 0.106 | 0.296 | 0.0411 | 0.0263 |
| 510 | 55 | 0 | 0.3 | 0.9 | 1 | 0.296 | 0.386 | 0.2704 | 0.0474 |
| 511 | 56 | 0 | 0.3 | 0.9 | 1 | 0.386 | 0.505 | 0.6101 | 0.0674 |
| 512 | 57 | 0 | 0.3 | 0.9 | 1 | 0.505 | 0.577 | 0.9462 | 0.1036 |
| 513 | 58 | 0 | 0.3 | 0.9 | 1 | 0.577 | 0.659 | 0.8564 | 0.1329 |
| 514 | 59 | 0 | 0.3 | 0.9 | 1 | 0.659 | 0.753 | 1.3596 | 0.1501 |
| 515 | 60 | 0 | 0.3 | 0.9 | 1 | 0.753 | 0.861 | 1.8552 | 0.1734 |
| 516 | 61 | 0 | 0.3 | 0.9 | 1 | 0.861 | 0.984 | 2.2332 | 0.1717 |
| 517 | 62 | 0 | 0.3 | 0.9 | 1 | 0.984 | 1.285 | 1.9993 | 0.1787 |
| 518 | 63 | 0 | 0.3 | 0.9 | 1 | 1.285 | 2.506 | 0.4039 | 0.0466 |
| 519 | 64 | 0.3 | 0.45 | -1 | -0.5 | 0.106 | 0.226 | 0.1132 | 0.0200 |
| 520 | 65 | 0.3 | 0.45 | -1 | -0.5 | 0.226 | 0.296 | 0.1961 | 0.0218 |
| 521 | 66 | 0.3 | 0.45 | -1 | -0.5 | 0.296 | 2.506 | 0.0094 | 0.0013 |
| 522 | 67 | 0.3 | 0.45 | -0.5 | 0 | 0.106 | 0.226 | 0.1089 | 0.0191 |
| 523 | 68 | 0.3 | 0.45 | -0.5 | 0 | 0.226 | 0.296 | 0.2272 | 0.0245 |
| 524 | 69 | 0.3 | 0.45 | -0.5 | 0 | 0.296 | 0.386 | 0.2591 | 0.0311 |

continued on next page

continued from previous page

| Global Bin | Bin | $E_{avail}$ Low (GeV) | $E_{avail}$ High (GeV) | $\cos\theta_\mu$ Low | $\cos\theta_\mu$ High | $E_\mu$ Low (GeV) | $E_\mu$ High (GeV) | $\frac{d^3\sigma}{dE_{avail}d\cos\theta_\mu dE_\mu}$ ($\times 10^{-36}\frac{\text{cm}^2}{\text{Ar GeV}^2}$) | Uncertainty ($\times 10^{-36}\frac{\text{cm}^2}{\text{Ar GeV}^2}$) |
|---|---|---|---|---|---|---|---|---|---|
| 525 | 70 | 0.3 | 0.45 | -0.5 | 0 | 0.386 | 0.505 | 0.1446 | 0.0138 |
| 526 | 71 | 0.3 | 0.45 | -0.5 | 0 | 0.505 | 2.506 | 0.0019 | 0.0002 |
| 527 | 72 | 0.3 | 0.45 | 0 | 0.3 | 0.106 | 0.226 | 0.0754 | 0.0163 |
| 528 | 73 | 0.3 | 0.45 | 0 | 0.3 | 0.226 | 0.296 | 0.2591 | 0.0245 |
| 529 | 74 | 0.3 | 0.45 | 0 | 0.3 | 0.296 | 0.386 | 0.3409 | 0.0271 |
| 530 | 75 | 0.3 | 0.45 | 0 | 0.3 | 0.386 | 0.505 | 0.3763 | 0.0364 |
| 531 | 76 | 0.3 | 0.45 | 0 | 0.3 | 0.505 | 0.577 | 0.2230 | 0.0222 |
| 532 | 77 | 0.3 | 0.45 | 0 | 0.3 | 0.577 | 2.506 | 0.0068 | 0.0007 |
| 533 | 78 | 0.3 | 0.45 | 0.3 | 0.5 | 0.106 | 0.226 | 0.0737 | 0.0154 |
| 534 | 79 | 0.3 | 0.45 | 0.3 | 0.5 | 0.226 | 0.296 | 0.3091 | 0.0300 |
| 535 | 80 | 0.3 | 0.45 | 0.3 | 0.5 | 0.296 | 0.386 | 0.4172 | 0.0345 |
| 536 | 81 | 0.3 | 0.45 | 0.3 | 0.5 | 0.386 | 0.505 | 0.4627 | 0.0406 |
| 537 | 82 | 0.3 | 0.45 | 0.3 | 0.5 | 0.505 | 0.577 | 0.4479 | 0.0394 |
| 538 | 83 | 0.3 | 0.45 | 0.3 | 0.5 | 0.577 | 0.659 | 0.4022 | 0.0369 |
| 539 | 84 | 0.3 | 0.45 | 0.3 | 0.5 | 0.659 | 0.753 | 0.2092 | 0.0181 |
| 540 | 85 | 0.3 | 0.45 | 0.3 | 0.5 | 0.753 | 2.506 | 0.0055 | 0.0005 |
| 541 | 86 | 0.3 | 0.45 | 0.5 | 0.7 | 0.106 | 0.226 | 0.0754 | 0.0157 |
| 542 | 87 | 0.3 | 0.45 | 0.5 | 0.7 | 0.226 | 0.296 | 0.3018 | 0.0346 |
| 543 | 88 | 0.3 | 0.45 | 0.5 | 0.7 | 0.296 | 0.386 | 0.4261 | 0.0382 |
| 544 | 89 | 0.3 | 0.45 | 0.5 | 0.7 | 0.386 | 0.505 | 0.4696 | 0.0509 |
| 545 | 90 | 0.3 | 0.45 | 0.5 | 0.7 | 0.505 | 0.577 | 0.5172 | 0.0495 |
| 546 | 91 | 0.3 | 0.45 | 0.5 | 0.7 | 0.577 | 0.659 | 0.5599 | 0.0460 |
| 547 | 92 | 0.3 | 0.45 | 0.5 | 0.7 | 0.659 | 0.753 | 0.5670 | 0.0489 |
| 548 | 93 | 0.3 | 0.45 | 0.5 | 0.7 | 0.753 | 0.861 | 0.3835 | 0.0392 |
| 549 | 94 | 0.3 | 0.45 | 0.5 | 0.7 | 0.861 | 0.984 | 0.1698 | 0.0179 |
| 550 | 95 | 0.3 | 0.45 | 0.5 | 0.7 | 0.984 | 2.506 | 0.0062 | 0.0007 |
| 551 | 96 | 0.3 | 0.45 | 0.7 | 0.8 | 0.106 | 0.296 | 0.0982 | 0.0204 |
| 552 | 97 | 0.3 | 0.45 | 0.7 | 0.8 | 0.296 | 0.386 | 0.3414 | 0.0372 |
| 553 | 98 | 0.3 | 0.45 | 0.7 | 0.8 | 0.386 | 0.505 | 0.4527 | 0.0507 |
| 554 | 99 | 0.3 | 0.45 | 0.7 | 0.8 | 0.505 | 0.577 | 0.5465 | 0.0516 |
| 555 | 100 | 0.3 | 0.45 | 0.7 | 0.8 | 0.577 | 0.659 | 0.6710 | 0.0517 |
| 556 | 101 | 0.3 | 0.45 | 0.7 | 0.8 | 0.659 | 0.753 | 0.6392 | 0.0469 |
| 557 | 102 | 0.3 | 0.45 | 0.7 | 0.8 | 0.753 | 0.861 | 0.6180 | 0.0520 |
| 558 | 103 | 0.3 | 0.45 | 0.7 | 0.8 | 0.861 | 0.984 | 0.5031 | 0.0518 |
| 559 | 104 | 0.3 | 0.45 | 0.7 | 0.8 | 0.984 | 2.506 | 0.0546 | 0.0069 |
| 560 | 105 | 0.3 | 0.45 | 0.8 | 0.9 | 0.106 | 0.296 | 0.0617 | 0.0166 |
| 561 | 106 | 0.3 | 0.45 | 0.8 | 0.9 | 0.296 | 0.386 | 0.2409 | 0.0324 |
| 562 | 107 | 0.3 | 0.45 | 0.8 | 0.9 | 0.386 | 0.505 | 0.3800 | 0.0483 |
| 563 | 108 | 0.3 | 0.45 | 0.8 | 0.9 | 0.505 | 0.577 | 0.5904 | 0.0634 |
| 564 | 109 | 0.3 | 0.45 | 0.8 | 0.9 | 0.577 | 0.659 | 0.6178 | 0.0530 |
| 565 | 110 | 0.3 | 0.45 | 0.8 | 0.9 | 0.659 | 0.753 | 0.7452 | 0.0628 |
| 566 | 111 | 0.3 | 0.45 | 0.8 | 0.9 | 0.753 | 0.861 | 0.6839 | 0.0646 |
| 567 | 112 | 0.3 | 0.45 | 0.8 | 0.9 | 0.861 | 0.984 | 0.6485 | 0.0662 |
| 568 | 113 | 0.3 | 0.45 | 0.8 | 0.9 | 0.984 | 1.285 | 0.4327 | 0.0516 |
| 569 | 114 | 0.3 | 0.45 | 0.8 | 0.9 | 1.285 | 2.506 | 0.0451 | 0.0061 |
| 570 | 115 | 0.3 | 0.45 | 0.9 | 1 | 0.106 | 0.296 | 0.0335 | 0.0136 |
| 571 | 116 | 0.3 | 0.45 | 0.9 | 1 | 0.296 | 0.386 | 0.1182 | 0.0219 |
| 572 | 117 | 0.3 | 0.45 | 0.9 | 1 | 0.386 | 0.505 | 0.2332 | 0.0334 |
| 573 | 118 | 0.3 | 0.45 | 0.9 | 1 | 0.505 | 0.577 | 0.3473 | 0.0414 |

continued on next page

continued from previous page

| Global Bin | Bin | $E_{avail}$ Low (GeV) | $E_{avail}$ High (GeV) | $\cos\theta_\mu$ Low | $\cos\theta_\mu$ High | $E_\mu$ Low (GeV) | $E_\mu$ High (GeV) | $\frac{d^3\sigma}{dE_{avail}d\cos\theta_\mu dE_\mu}$ ($\times10^{-36}\frac{\text{cm}^2}{\text{Ar GeV}^2}$) | Uncertainty ($\times10^{-36}\frac{\text{cm}^2}{\text{Ar GeV}^2}$) |
|---|---|---|---|---|---|---|---|---|---|
| 574 | 119 | 0.3 | 0.45 | 0.9 | 1 | 0.577 | 0.659 | 0.4093 | 0.0487 |
| 575 | 120 | 0.3 | 0.45 | 0.9 | 1 | 0.659 | 0.753 | 0.5344 | 0.0591 |
| 576 | 121 | 0.3 | 0.45 | 0.9 | 1 | 0.753 | 0.861 | 0.5774 | 0.0691 |
| 577 | 122 | 0.3 | 0.45 | 0.9 | 1 | 0.861 | 0.984 | 0.5686 | 0.0741 |
| 578 | 123 | 0.3 | 0.45 | 0.9 | 1 | 0.984 | 1.285 | 0.3660 | 0.0588 |
| 579 | 124 | 0.3 | 0.45 | 0.9 | 1 | 1.285 | 2.506 | 0.0884 | 0.0215 |
| 580 | 125 | 0.45 | 0.65 | -1 | -0.5 | 0.106 | 0.226 | 0.0600 | 0.0114 |
| 581 | 126 | 0.45 | 0.65 | -1 | -0.5 | 0.226 | 0.296 | 0.1084 | 0.0116 |
| 582 | 127 | 0.45 | 0.65 | -1 | -0.5 | 0.296 | 0.386 | 0.0804 | 0.0097 |
| 583 | 128 | 0.45 | 0.65 | -1 | -0.5 | 0.386 | 2.506 | 0.0010 | 0.0002 |
| 584 | 129 | 0.45 | 0.65 | -0.5 | 0 | 0.106 | 0.226 | 0.0548 | 0.0101 |
| 585 | 130 | 0.45 | 0.65 | -0.5 | 0 | 0.226 | 0.296 | 0.1375 | 0.0121 |
| 586 | 131 | 0.45 | 0.65 | -0.5 | 0 | 0.296 | 0.386 | 0.1613 | 0.0135 |
| 587 | 132 | 0.45 | 0.65 | -0.5 | 0 | 0.386 | 0.505 | 0.1046 | 0.0094 |
| 588 | 133 | 0.45 | 0.65 | -0.5 | 0 | 0.505 | 2.506 | 0.0018 | 0.0002 |
| 589 | 134 | 0.45 | 0.65 | 0 | 0.3 | 0.106 | 0.226 | 0.0362 | 0.0102 |
| 590 | 135 | 0.45 | 0.65 | 0 | 0.3 | 0.226 | 0.296 | 0.1434 | 0.0140 |
| 591 | 136 | 0.45 | 0.65 | 0 | 0.3 | 0.296 | 0.386 | 0.1803 | 0.0149 |
| 592 | 137 | 0.45 | 0.65 | 0 | 0.3 | 0.386 | 0.505 | 0.1864 | 0.0151 |
| 593 | 138 | 0.45 | 0.65 | 0 | 0.3 | 0.505 | 0.577 | 0.1454 | 0.0136 |
| 594 | 139 | 0.45 | 0.65 | 0 | 0.3 | 0.577 | 2.506 | 0.0070 | 0.0008 |
| 595 | 140 | 0.45 | 0.65 | 0.3 | 0.5 | 0.106 | 0.226 | 0.0272 | 0.0083 |
| 596 | 141 | 0.45 | 0.65 | 0.3 | 0.5 | 0.226 | 0.296 | 0.1408 | 0.0154 |
| 597 | 142 | 0.45 | 0.65 | 0.3 | 0.5 | 0.296 | 0.386 | 0.1967 | 0.0158 |
| 598 | 143 | 0.45 | 0.65 | 0.3 | 0.5 | 0.386 | 0.505 | 0.1890 | 0.0161 |
| 599 | 144 | 0.45 | 0.65 | 0.3 | 0.5 | 0.505 | 0.577 | 0.1965 | 0.0181 |
| 600 | 145 | 0.45 | 0.65 | 0.3 | 0.5 | 0.577 | 0.659 | 0.1957 | 0.0187 |
| 601 | 146 | 0.45 | 0.65 | 0.3 | 0.5 | 0.659 | 0.753 | 0.1526 | 0.0149 |
| 602 | 147 | 0.45 | 0.65 | 0.3 | 0.5 | 0.753 | 2.506 | 0.0063 | 0.0007 |
| 603 | 148 | 0.45 | 0.65 | 0.5 | 0.7 | 0.106 | 0.226 | 0.0288 | 0.0079 |
| 604 | 149 | 0.45 | 0.65 | 0.5 | 0.7 | 0.226 | 0.296 | 0.1182 | 0.0160 |
| 605 | 150 | 0.45 | 0.65 | 0.5 | 0.7 | 0.296 | 0.386 | 0.1852 | 0.0174 |
| 606 | 151 | 0.45 | 0.65 | 0.5 | 0.7 | 0.386 | 0.505 | 0.1857 | 0.0188 |
| 607 | 152 | 0.45 | 0.65 | 0.5 | 0.7 | 0.505 | 0.577 | 0.1794 | 0.0214 |
| 608 | 153 | 0.45 | 0.65 | 0.5 | 0.7 | 0.577 | 0.659 | 0.1911 | 0.0173 |
| 609 | 154 | 0.45 | 0.65 | 0.5 | 0.7 | 0.659 | 0.753 | 0.2033 | 0.0185 |
| 610 | 155 | 0.45 | 0.65 | 0.5 | 0.7 | 0.753 | 0.861 | 0.1660 | 0.0198 |
| 611 | 156 | 0.45 | 0.65 | 0.5 | 0.7 | 0.861 | 0.984 | 0.1041 | 0.0131 |
| 612 | 157 | 0.45 | 0.65 | 0.5 | 0.7 | 0.984 | 2.506 | 0.0055 | 0.0007 |
| 613 | 158 | 0.45 | 0.65 | 0.7 | 0.8 | 0.106 | 0.296 | 0.0399 | 0.0095 |
| 614 | 159 | 0.45 | 0.65 | 0.7 | 0.8 | 0.296 | 0.386 | 0.1346 | 0.0168 |
| 615 | 160 | 0.45 | 0.65 | 0.7 | 0.8 | 0.386 | 0.505 | 0.1709 | 0.0200 |
| 616 | 161 | 0.45 | 0.65 | 0.7 | 0.8 | 0.505 | 0.577 | 0.1882 | 0.0236 |
| 617 | 162 | 0.45 | 0.65 | 0.7 | 0.8 | 0.577 | 0.659 | 0.1870 | 0.0208 |
| 618 | 163 | 0.45 | 0.65 | 0.7 | 0.8 | 0.659 | 0.753 | 0.1867 | 0.0185 |
| 619 | 164 | 0.45 | 0.65 | 0.7 | 0.8 | 0.753 | 0.861 | 0.1981 | 0.0214 |
| 620 | 165 | 0.45 | 0.65 | 0.7 | 0.8 | 0.861 | 0.984 | 0.1500 | 0.0192 |
| 621 | 166 | 0.45 | 0.65 | 0.7 | 0.8 | 0.984 | 2.506 | 0.0223 | 0.0036 |
| 622 | 167 | 0.45 | 0.65 | 0.8 | 0.9 | 0.106 | 0.296 | 0.0292 | 0.0090 |

continued on next page

continued from previous page

| Global Bin | Bin | $E_{avail}$ Low (GeV) | $E_{avail}$ High (GeV) | $\cos\theta_\mu$ Low | $\cos\theta_\mu$ High | $E_\mu$ Low (GeV) | $E_\mu$ High (GeV) | $\frac{d^3\sigma}{dE_{avail}d\cos\theta_\mu dE_\mu}$ ($\times10^{-36}\frac{\text{cm}^2}{\text{Ar GeV}^2}$) | Uncertainty ($\times10^{-36}\frac{\text{cm}^2}{\text{Ar GeV}^2}$) |
|---|---|---|---|---|---|---|---|---|---|
| 623 | 168 | 0.45 | 0.65 | 0.8 | 0.9 | 0.296 | 0.386 | 0.0974 | 0.0178 |
| 624 | 169 | 0.45 | 0.65 | 0.8 | 0.9 | 0.386 | 0.505 | 0.1359 | 0.0195 |
| 625 | 170 | 0.45 | 0.65 | 0.8 | 0.9 | 0.505 | 0.577 | 0.1638 | 0.0225 |
| 626 | 171 | 0.45 | 0.65 | 0.8 | 0.9 | 0.577 | 0.659 | 0.1966 | 0.0251 |
| 627 | 172 | 0.45 | 0.65 | 0.8 | 0.9 | 0.659 | 0.753 | 0.1970 | 0.0237 |
| 628 | 173 | 0.45 | 0.65 | 0.8 | 0.9 | 0.753 | 0.861 | 0.1871 | 0.0260 |
| 629 | 174 | 0.45 | 0.65 | 0.8 | 0.9 | 0.861 | 0.984 | 0.1404 | 0.0212 |
| 630 | 175 | 0.45 | 0.65 | 0.8 | 0.9 | 0.984 | 1.285 | 0.0871 | 0.0140 |
| 631 | 176 | 0.45 | 0.65 | 0.8 | 0.9 | 1.285 | 2.506 | 0.0150 | 0.0026 |
| 632 | 177 | 0.45 | 0.65 | 0.9 | 1 | 0.106 | 0.386 | 0.0223 | 0.0098 |
| 633 | 178 | 0.45 | 0.65 | 0.9 | 1 | 0.386 | 0.505 | 0.0741 | 0.0167 |
| 634 | 179 | 0.45 | 0.65 | 0.9 | 1 | 0.505 | 0.577 | 0.1087 | 0.0201 |
| 635 | 180 | 0.45 | 0.65 | 0.9 | 1 | 0.577 | 0.659 | 0.1343 | 0.0224 |
| 636 | 181 | 0.45 | 0.65 | 0.9 | 1 | 0.659 | 0.753 | 0.1319 | 0.0227 |
| 637 | 182 | 0.45 | 0.65 | 0.9 | 1 | 0.753 | 0.861 | 0.1208 | 0.0267 |
| 638 | 183 | 0.45 | 0.65 | 0.9 | 1 | 0.861 | 0.984 | 0.0939 | 0.0242 |
| 639 | 184 | 0.45 | 0.65 | 0.9 | 1 | 0.984 | 1.285 | 0.0527 | 0.0121 |
| 640 | 185 | 0.45 | 0.65 | 0.9 | 1 | 1.285 | 2.506 | 0.0178 | 0.0052 |
| 641 | 186 | 0.65 | 2.5 | -1 | -0.5 | 0.106 | 0.226 | 0.0069 | 0.0021 |
| 642 | 187 | 0.65 | 2.5 | -1 | -0.5 | 0.226 | 0.296 | 0.0114 | 0.0022 |
| 643 | 188 | 0.65 | 2.5 | -1 | -0.5 | 0.296 | 0.386 | 0.0071 | 0.0015 |
| 644 | 189 | 0.65 | 2.5 | -1 | -0.5 | 0.386 | 2.506 | 0.0001 | 0.0001 |
| 645 | 190 | 0.65 | 2.5 | -0.5 | 0 | 0.106 | 0.226 | 0.0075 | 0.0019 |
| 646 | 191 | 0.65 | 2.5 | -0.5 | 0 | 0.226 | 0.296 | 0.0192 | 0.0024 |
| 647 | 192 | 0.65 | 2.5 | -0.5 | 0 | 0.296 | 0.386 | 0.0159 | 0.0020 |
| 648 | 193 | 0.65 | 2.5 | -0.5 | 0 | 0.386 | 0.505 | 0.0097 | 0.0014 |
| 649 | 194 | 0.65 | 2.5 | -0.5 | 0 | 0.505 | 2.506 | 0.0003 | 0.0001 |
| 650 | 195 | 0.65 | 2.5 | 0 | 0.3 | 0.106 | 0.226 | 0.0049 | 0.0021 |
| 651 | 196 | 0.65 | 2.5 | 0 | 0.3 | 0.226 | 0.296 | 0.0185 | 0.0026 |
| 652 | 197 | 0.65 | 2.5 | 0 | 0.3 | 0.296 | 0.386 | 0.0190 | 0.0027 |
| 653 | 198 | 0.65 | 2.5 | 0 | 0.3 | 0.386 | 0.505 | 0.0147 | 0.0024 |
| 654 | 199 | 0.65 | 2.5 | 0 | 0.3 | 0.505 | 0.577 | 0.0116 | 0.0021 |
| 655 | 200 | 0.65 | 2.5 | 0 | 0.3 | 0.577 | 0.659 | 0.0089 | 0.0015 |
| 656 | 201 | 0.65 | 2.5 | 0 | 0.3 | 0.659 | 2.506 | 0.0004 | 0.0001 |
| 657 | 202 | 0.65 | 2.5 | 0.3 | 0.5 | 0.106 | 0.226 | 0.0032 | 0.0020 |
| 658 | 203 | 0.65 | 2.5 | 0.3 | 0.5 | 0.226 | 0.296 | 0.0161 | 0.0030 |
| 659 | 204 | 0.65 | 2.5 | 0.3 | 0.5 | 0.296 | 0.386 | 0.0205 | 0.0029 |
| 660 | 205 | 0.65 | 2.5 | 0.3 | 0.5 | 0.386 | 0.505 | 0.0160 | 0.0029 |
| 661 | 206 | 0.65 | 2.5 | 0.3 | 0.5 | 0.505 | 0.577 | 0.0134 | 0.0024 |
| 662 | 207 | 0.65 | 2.5 | 0.3 | 0.5 | 0.577 | 0.659 | 0.0143 | 0.0022 |
| 663 | 208 | 0.65 | 2.5 | 0.3 | 0.5 | 0.659 | 0.753 | 0.0122 | 0.0018 |
| 664 | 209 | 0.65 | 2.5 | 0.3 | 0.5 | 0.753 | 2.506 | 0.0009 | 0.0001 |
| 665 | 210 | 0.65 | 2.5 | 0.5 | 0.7 | 0.106 | 0.226 | 0.0035 | 0.0018 |
| 666 | 211 | 0.65 | 2.5 | 0.5 | 0.7 | 0.226 | 0.296 | 0.0143 | 0.0031 |
| 667 | 212 | 0.65 | 2.5 | 0.5 | 0.7 | 0.296 | 0.386 | 0.0205 | 0.0032 |
| 668 | 213 | 0.65 | 2.5 | 0.5 | 0.7 | 0.386 | 0.505 | 0.0187 | 0.0037 |
| 669 | 214 | 0.65 | 2.5 | 0.5 | 0.7 | 0.505 | 0.577 | 0.0153 | 0.0034 |
| 670 | 215 | 0.65 | 2.5 | 0.5 | 0.7 | 0.577 | 0.659 | 0.0150 | 0.0025 |
| 671 | 216 | 0.65 | 2.5 | 0.5 | 0.7 | 0.659 | 0.753 | 0.0140 | 0.0021 |

continued on next page

continued from previous page

| Global Bin | Bin | $E_{avail}$ Low (GeV) | $E_{avail}$ High (GeV) | $\cos\theta_\mu$ Low | $\cos\theta_\mu$ High | $E_\mu$ Low (GeV) | $E_\mu$ High (GeV) | $\frac{d^3\sigma}{dE_{avail}d\cos\theta_\mu dE_\mu}$ $(\times10^{-36}\frac{\text{cm}^2}{\text{Ar GeV}^2})$ | Uncertainty $(\times10^{-36}\frac{\text{cm}^2}{\text{Ar GeV}^2})$ |
|---|---|---|---|---|---|---|---|---|---|
| 672 | 217 | 0.65 | 2.5 | 0.5 | 0.7 | 0.753 | 0.861 | 0.0114 | 0.0020 |
| 673 | 218 | 0.65 | 2.5 | 0.5 | 0.7 | 0.861 | 0.984 | 0.0083 | 0.0015 |
| 674 | 219 | 0.65 | 2.5 | 0.5 | 0.7 | 0.984 | 2.506 | 0.0008 | 0.0002 |
| 675 | 220 | 0.65 | 2.5 | 0.7 | 0.8 | 0.106 | 0.296 | 0.0056 | 0.0019 |
| 676 | 221 | 0.65 | 2.5 | 0.7 | 0.8 | 0.296 | 0.386 | 0.0190 | 0.0035 |
| 677 | 222 | 0.65 | 2.5 | 0.7 | 0.8 | 0.386 | 0.505 | 0.0208 | 0.0040 |
| 678 | 223 | 0.65 | 2.5 | 0.7 | 0.8 | 0.505 | 0.577 | 0.0178 | 0.0036 |
| 679 | 224 | 0.65 | 2.5 | 0.7 | 0.8 | 0.577 | 0.659 | 0.0157 | 0.0029 |
| 680 | 225 | 0.65 | 2.5 | 0.7 | 0.8 | 0.659 | 0.753 | 0.0143 | 0.0023 |
| 681 | 226 | 0.65 | 2.5 | 0.7 | 0.8 | 0.753 | 0.861 | 0.0120 | 0.0021 |
| 682 | 227 | 0.65 | 2.5 | 0.7 | 0.8 | 0.861 | 0.984 | 0.0105 | 0.0021 |
| 683 | 228 | 0.65 | 2.5 | 0.7 | 0.8 | 0.984 | 1.285 | 0.0064 | 0.0015 |
| 684 | 229 | 0.65 | 2.5 | 0.7 | 0.8 | 1.285 | 2.506 | 0.0011 | 0.0002 |
| 685 | 230 | 0.65 | 2.5 | 0.8 | 0.9 | 0.106 | 0.296 | 0.0045 | 0.0019 |
| 686 | 231 | 0.65 | 2.5 | 0.8 | 0.9 | 0.296 | 0.386 | 0.0122 | 0.0030 |
| 687 | 232 | 0.65 | 2.5 | 0.8 | 0.9 | 0.386 | 0.505 | 0.0150 | 0.0032 |
| 688 | 233 | 0.65 | 2.5 | 0.8 | 0.9 | 0.505 | 0.577 | 0.0175 | 0.0037 |
| 689 | 234 | 0.65 | 2.5 | 0.8 | 0.9 | 0.577 | 0.659 | 0.0163 | 0.0033 |
| 690 | 235 | 0.65 | 2.5 | 0.8 | 0.9 | 0.659 | 0.753 | 0.0144 | 0.0030 |
| 691 | 236 | 0.65 | 2.5 | 0.8 | 0.9 | 0.753 | 0.861 | 0.0127 | 0.0032 |
| 692 | 237 | 0.65 | 2.5 | 0.8 | 0.9 | 0.861 | 0.984 | 0.0086 | 0.0023 |
| 693 | 238 | 0.65 | 2.5 | 0.8 | 0.9 | 0.984 | 1.285 | 0.0063 | 0.0016 |
| 694 | 239 | 0.65 | 2.5 | 0.8 | 0.9 | 1.285 | 2.506 | 0.0028 | 0.0007 |
| 695 | 240 | 0.65 | 2.5 | 0.9 | 1 | 0.106 | 0.386 | 0.0032 | 0.0020 |
| 696 | 241 | 0.65 | 2.5 | 0.9 | 1 | 0.386 | 0.505 | 0.0085 | 0.0030 |
| 697 | 242 | 0.65 | 2.5 | 0.9 | 1 | 0.505 | 0.577 | 0.0107 | 0.0031 |
| 698 | 243 | 0.65 | 2.5 | 0.9 | 1 | 0.577 | 0.659 | 0.0111 | 0.0028 |
| 699 | 244 | 0.65 | 2.5 | 0.9 | 1 | 0.659 | 0.753 | 0.0108 | 0.0030 |
| 700 | 245 | 0.65 | 2.5 | 0.9 | 1 | 0.753 | 0.861 | 0.0081 | 0.0032 |
| 701 | 246 | 0.65 | 2.5 | 0.9 | 1 | 0.861 | 0.984 | 0.0053 | 0.0025 |
| 702 | 247 | 0.65 | 2.5 | 0.9 | 1 | 0.984 | 1.285 | 0.0032 | 0.0013 |
| 703 | 248 | 0.65 | 2.5 | 0.9 | 1 | 1.285 | 2.506 | 0.0027 | 0.0016 |

TABLE XVIII: Unfolded Xp $E_{avail}$, $\cos\theta_\mu$, and $E_\mu$ triple-differential cross section result. Bin describes the binning structure for the given measurement and Global Bin describes the binning structure used in the blockwise covariance matrix. The Uncertainty column corresponds to the square root of the diagonal elements of the extracted covariance matrix.

[1] P. Abratenko *et al.* (MicroBooNE Collaboration), First Simultaneous Measurement of Differential Muon-Neutrino Charged-Current Cross Sections on Argon for Final States with and Without Protons Using MicroBooNE Data, Phys. Rev. Lett. **133**, 041801 (2024).
[2] P. Abratenko *et al.* (MicroBooNE Collaboration), First Measurement of Energy-Dependent Inclusive Muon Neutrino Charged-Current Cross Sections on Argon with the MicroBooNE Detector, Phys. Rev. Lett. **128**, 151801 (2022).
[3] P. Stowell *et al.* (MINER$\nu$A Collaboration), Tuning the GENIE pion production model with MINER$\nu$A data, Phys. Rev. D **100**, 072005 (2019).
[4] S. Gardiner, Mathematical methods for neutrino cross-section extraction, arXiv preprint (2024), arXiv:2401.04065 [hep-ex].
